# Supplementary material for: Z-Sequence: Photometric redshift predictions for galaxy clusters with sequential random k-nearest neighbours
Source: arXiv:2104.11335 source file (2021-04-22)
Supplement: Supplementary file 1 [file supplementary_material_online.pdf]

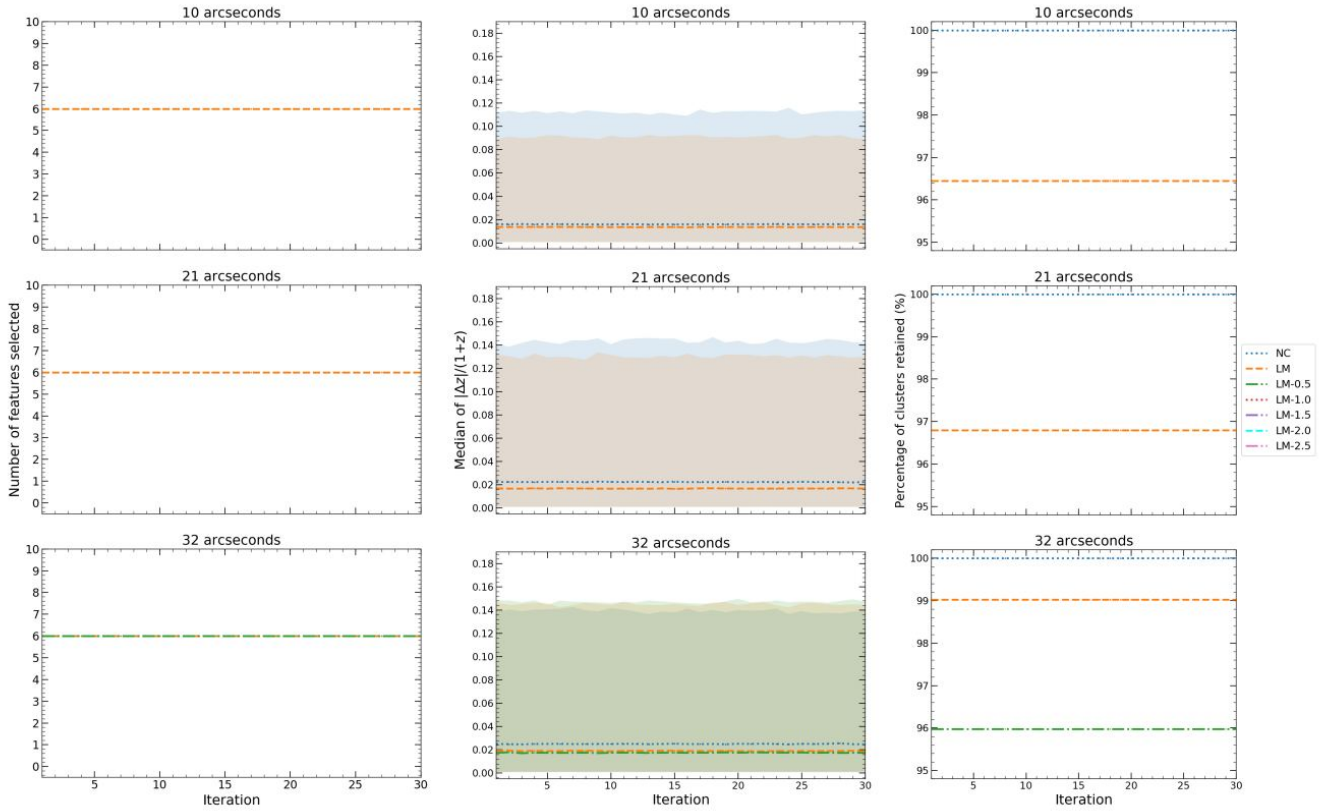

**Figure S1.** Plots displaying the results from applying filter magnitude-cuts to the MWAR training set using a single KNN algorithm with a control group of manually selected features for each search radii (10 arcseconds on the top row, 21 arcseconds on the middle row and 32 arcseconds on the bottom row). 'NC' represents a dataset with no filter magnitude-cuts applied and 'LM' represents the MWAR dataset with SFS selected features where filter magnitude-cuts are applied to the limiting magnitude of SDSS. In addition, 'LM' is the faintest filter magnitude-cut whilst 'LM-2.5' is the brightest filter magnitude-cut. Left column: Number of features selected for the control group feature subset in ten-fold cross validation across thirty repeats. Middle column: Median of photometric redshift prediction errors ( $|\Delta z|/(1+z)$ ) across all tested clusters for the control group feature subset in ten-fold cross validation across thirty repeats, where the shaded regions represent 95 per cent confidence intervals. Right column: Percentage of test clusters retained after filter magnitude-cuts are applied with the control group feature subset in ten-fold cross validation across thirty repeats. It should be noted that if the percentage of clusters retained, after filter magnitude-cuts are applied, do not satisfy the 95 per cent cluster retainment threshold we would not display the corresponding results in the other columns.

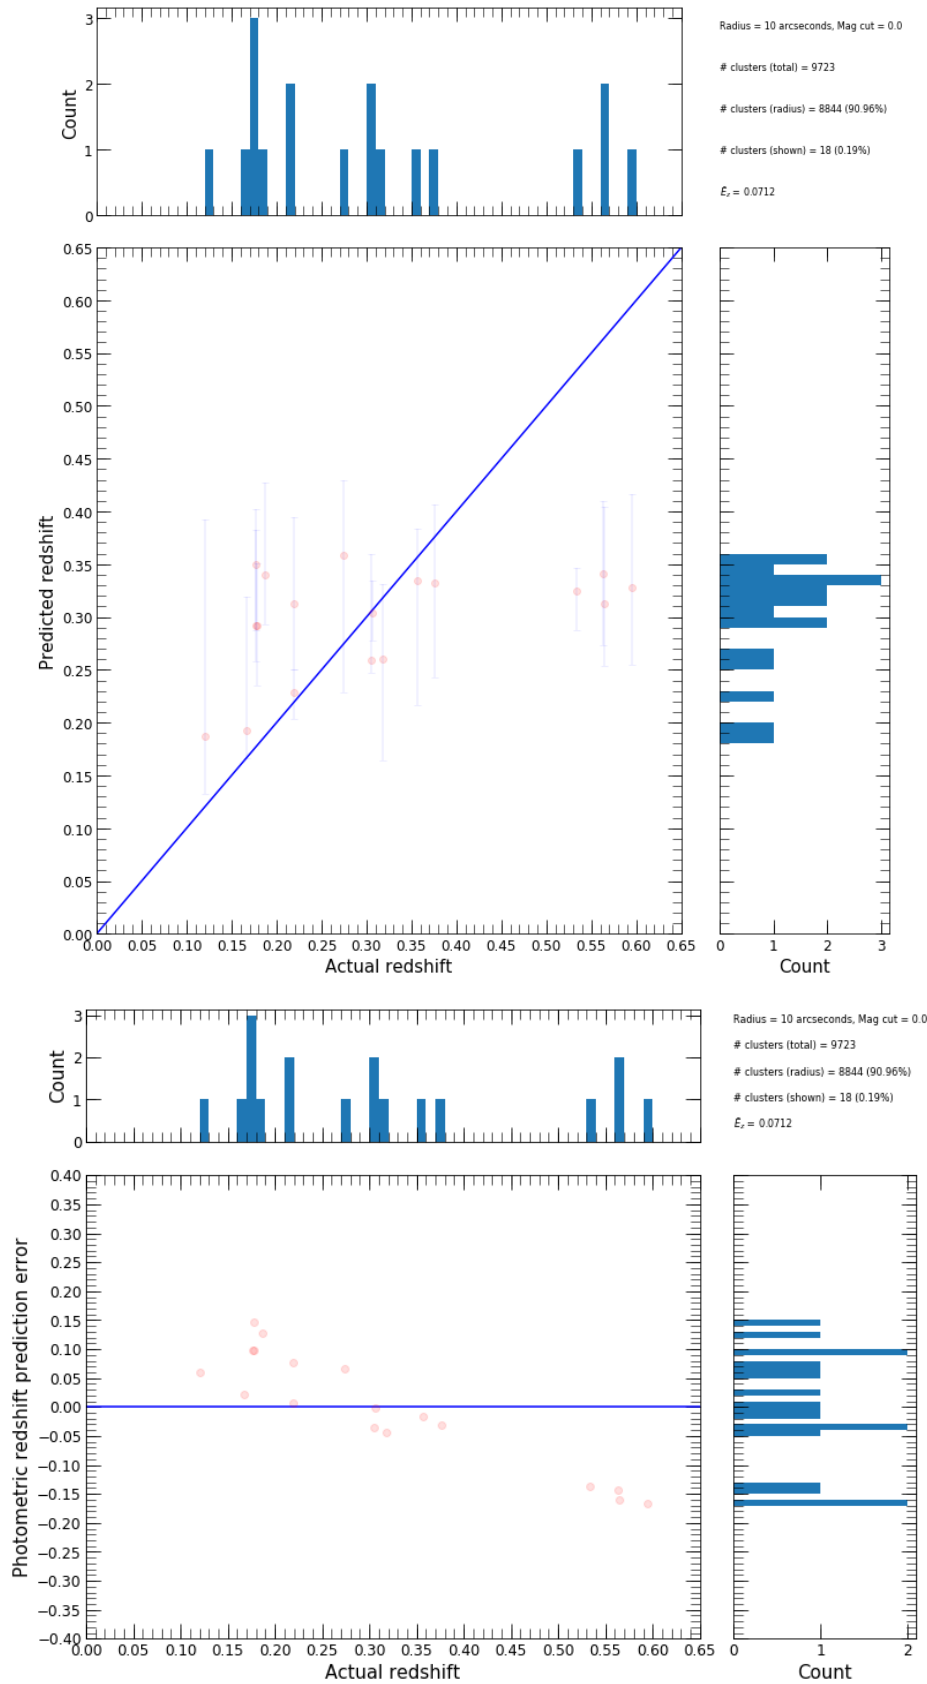

**Figure S2.** Plots displaying the performance of photometric redshift predictions of clusters for the WNMR dataset that had partial bootstrap resamples returned within a 10 arcseconds search radius. Top row: Predicted versus 'actual' photometric redshift of tested clusters with frequency histograms of the distributions. Bottom row: Non-absolute photometric redshift prediction error versus 'actual' redshift of tested clusters with frequency histograms of the distributions. Other: '# clusters (total)' represents the total number of clusters in the WNMR dataset, '# clusters (radius)' represents the number of clusters in the WNMR test set that have observed galaxies within a 10 arcseconds search radius, '# clusters (shown)' represents the number of clusters in the WNMR test set that have observed galaxies within a 10 arcseconds search radius with partial bootstrap resamples returned,  $\tilde{E}_z$  represents the median of photometric redshift prediction errors across all tested clusters within a 10 arcseconds search radius with partial bootstrap resamples returned.

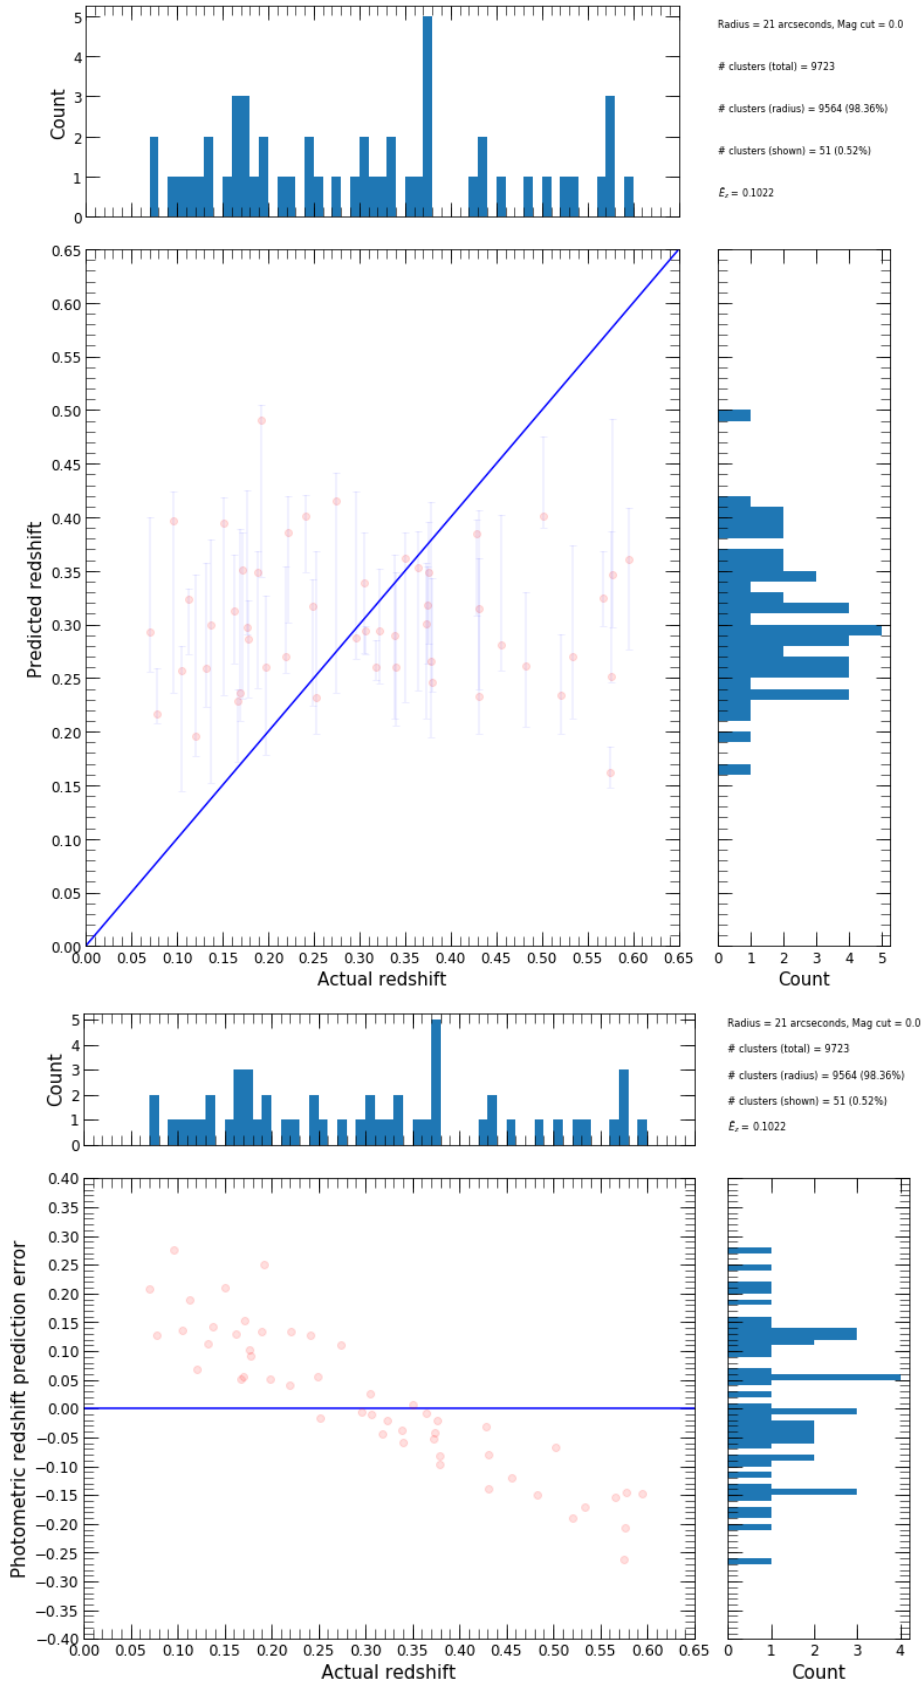

**Figure S3.** Plots displaying the performance of photometric redshift predictions of clusters for the WNMN dataset that had partial bootstrap resamples returned within a 21 arcseconds search radius. Top row: Predicted versus 'actual' photometric redshift of tested clusters with frequency histograms of the distributions. Bottom row: Non-absolute photometric redshift prediction error versus 'actual' redshift of tested clusters with frequency histograms of the distributions. Other: '# clusters (total)' represents the total number of clusters in the WNMN dataset, '# clusters (radius)' represents the number of clusters in the WNMN test set that have observed galaxies within a 21 arcseconds search radius, '# clusters (shown)' represents the number of clusters in the WNMN test set that have observed galaxies within a 21 arcseconds search radius with partial bootstrap resamples returned,  $\bar{E}_z$  represents the median of photometric redshift prediction errors across all tested clusters within a 21 arcseconds search radius with partial bootstrap resamples returned.

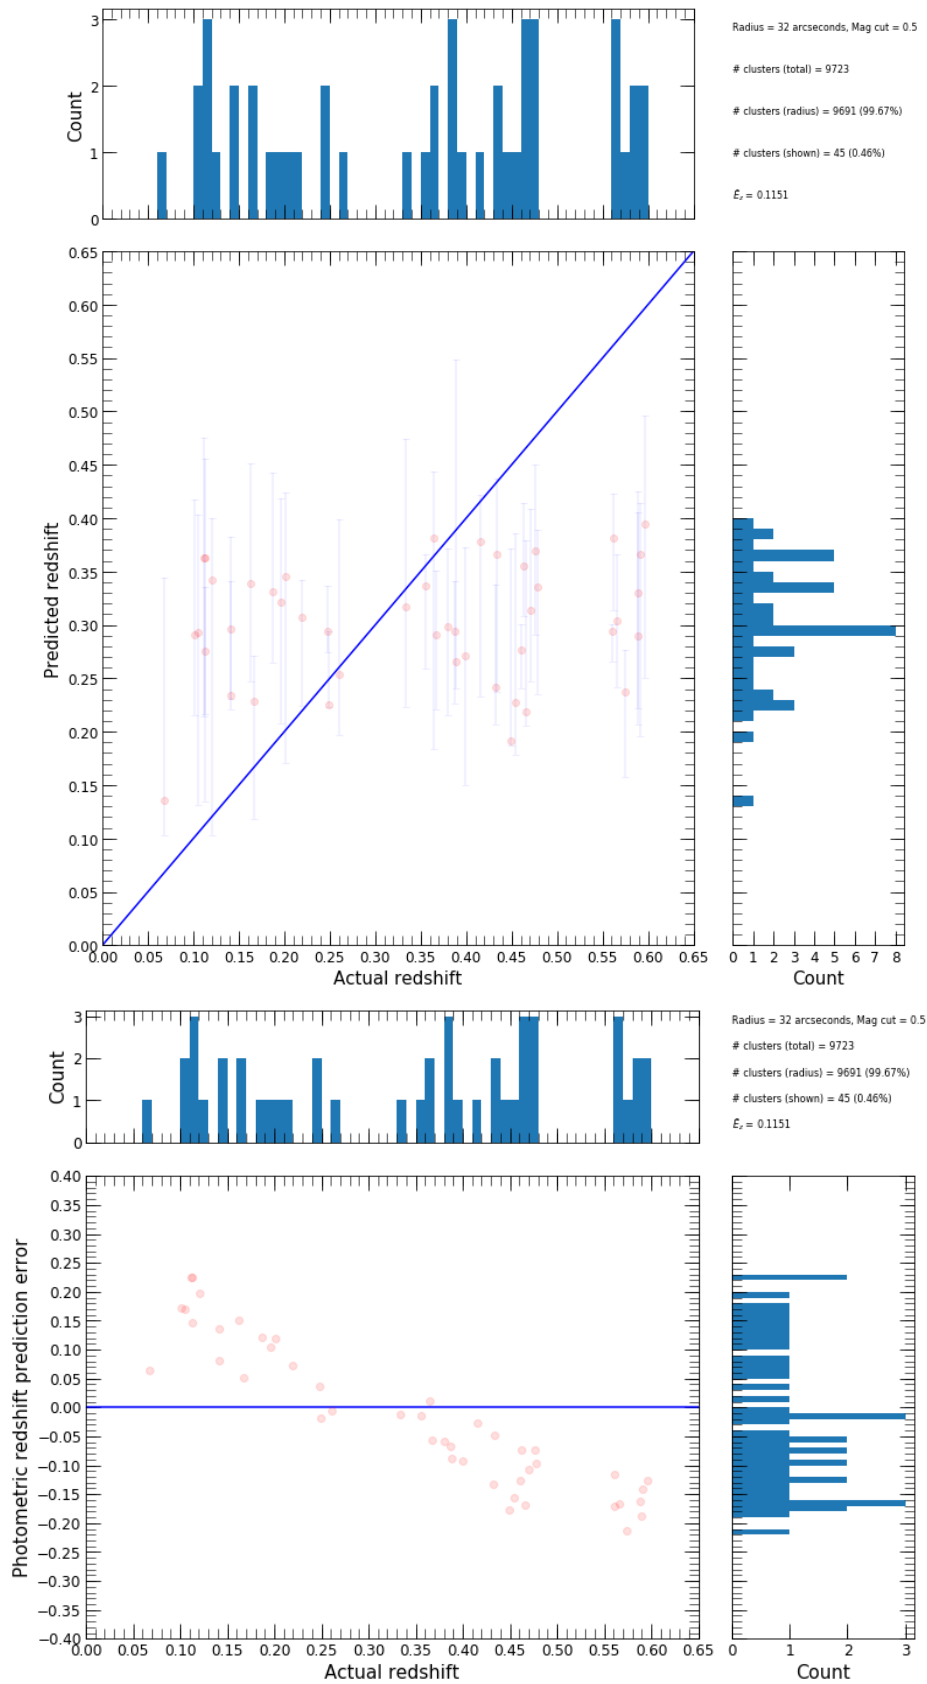

**Figure S4.** Plots displaying the performance of photometric redshift predictions of clusters for the WNMR dataset that had partial bootstrap resamples returned within a 32 arcseconds search radius. Top row: Predicted versus 'actual' photometric redshift of tested clusters with frequency histograms of the distributions. Bottom row: Non-absolute photometric redshift prediction error versus 'actual' redshift of tested clusters with frequency histograms of the distributions. Other: '# clusters (total)' represents the total number of clusters in the WNMR dataset, '# clusters (radius)' represents the number of clusters in the WNMR test set that have observed galaxies within a 32 arcseconds search radius, '# clusters (shown)' represents the number of clusters in the WNMR test set that have observed galaxies within a 32 arcseconds search radius with partial bootstrap resamples returned,  $\bar{E}_z$  represents the median of photometric redshift prediction errors across all tested clusters within a 32 arcseconds search radius with partial bootstrap resamples returned.



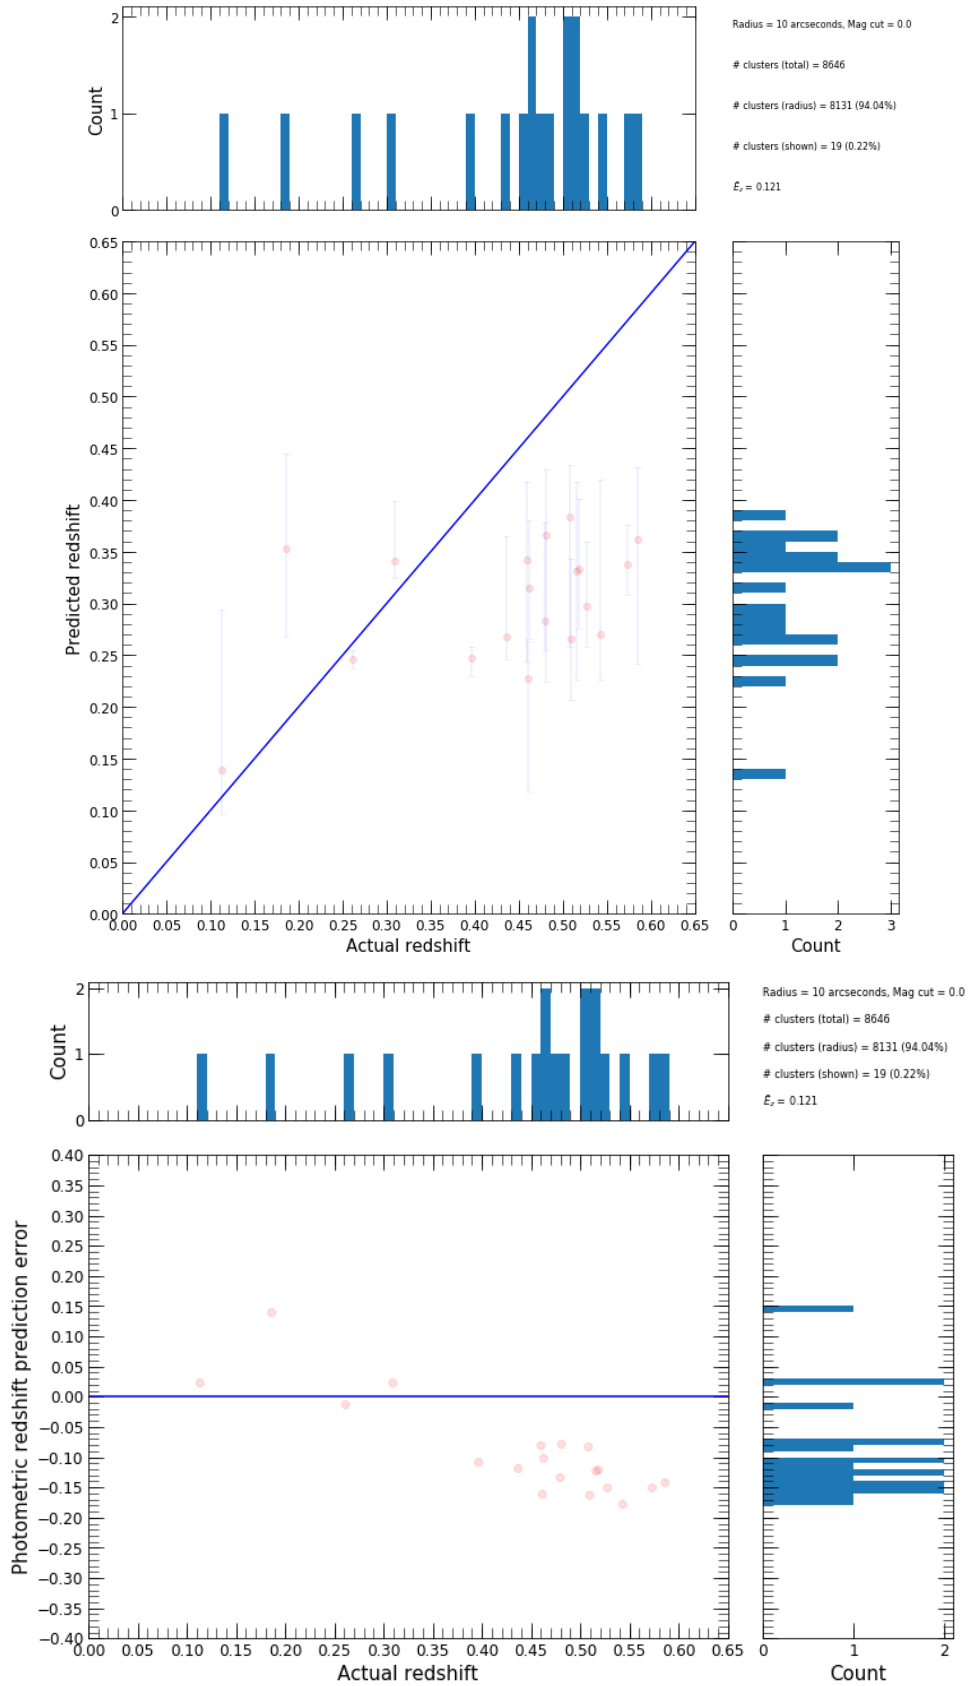

**Figure S5.** Plots displaying the performance of photometric redshift predictions of clusters for the RNMW dataset that had partial bootstrap resamples returned within a 10 arcseconds search radius. Top row: Predicted versus 'actual' photometric redshift of tested clusters with frequency histograms of the distributions. Bottom row: Non-absolute photometric redshift prediction error versus 'actual' redshift of tested clusters with frequency histograms of the distributions. Other: '# clusters (total)' represents the total number of clusters in the RNMW dataset, '# clusters (radius)' represents the number of clusters in the RNMW test set that have observed galaxies within a 10 arcseconds search radius, '# clusters (shown)' represents the number of clusters in the RNMW test set that have observed galaxies within a 10 arcseconds search radius with partial bootstrap resamples returned,  $\bar{E}_z$  represents the median of photometric redshift prediction errors across all tested clusters within a 10 arcseconds search radius with partial bootstrap resamples returned.

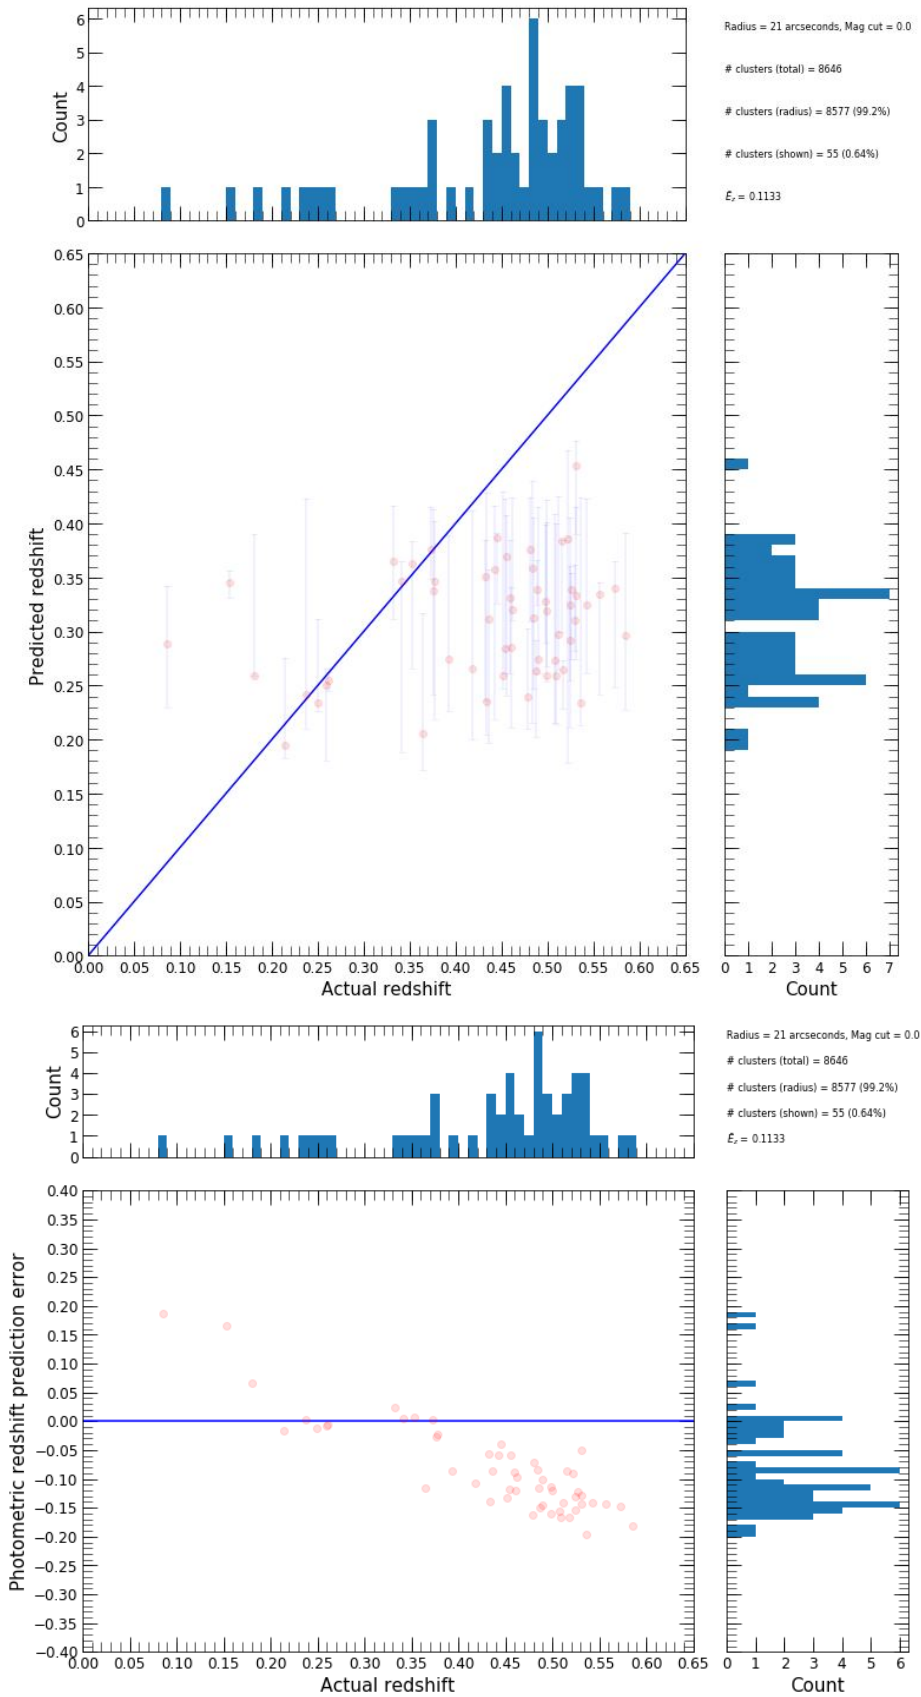

**Figure S6.** Plots displaying the performance of photometric redshift predictions of clusters for the RNMW dataset that had partial bootstrap resamples returned within a 21 arcseconds search radius. Top row: Predicted versus 'actual' photometric redshift of tested clusters with frequency histograms of the distributions. Bottom row: Non-absolute photometric redshift prediction error versus 'actual' redshift of tested clusters with frequency histograms of the distributions. Other: '# clusters (total)' represents the total number of clusters in the RNMW dataset, '# clusters (radius)' represents the number of clusters in the RNMW test set that have observed galaxies within a 21 arcseconds search radius, '# clusters (shown)' represents the number of clusters in the RNMW test set that have observed galaxies within a 21 arcseconds search radius with partial bootstrap resamples returned,  $\bar{E}_z$  represents the median of photometric redshift prediction errors across all tested clusters within a 21 arcseconds search radius with partial bootstrap resamples returned.

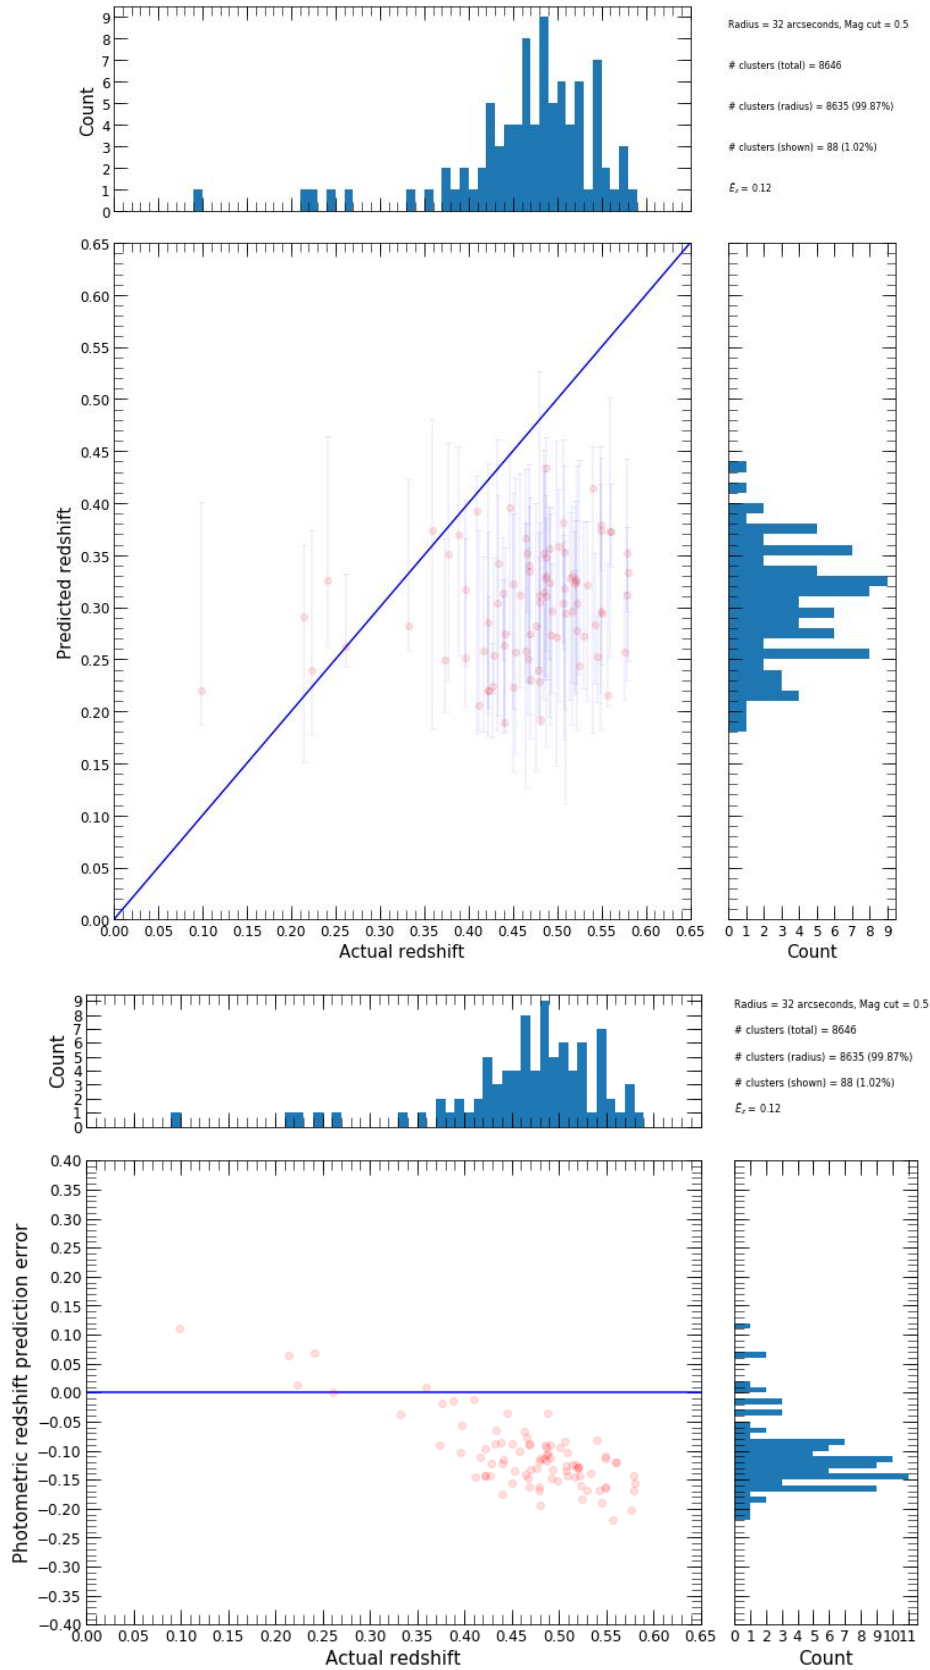

**Figure S7.** Plots displaying the performance of photometric redshift predictions of clusters for the RNMW dataset that had partial bootstrap resamples returned within a 32 arcseconds search radius. Top row: Predicted versus 'actual' photometric redshift of tested clusters with frequency histograms of the distributions. Bottom row: Non-absolute photometric redshift prediction error versus 'actual' redshift of tested clusters with frequency histograms of the distributions. Other: '# clusters (total)' represents the total number of clusters in the RNMW dataset, '# clusters (radius)' represents the number of clusters in the RNMW test set that have observed galaxies within a 32 arcseconds search radius, '# clusters (shown)' represents the number of clusters in the RNMW test set that have observed galaxies within a 32 arcseconds search radius with partial bootstrap resamples returned,  $\bar{E}_z$  represents the median of photometric redshift prediction errors across all tested clusters within a 32 arcseconds search radius with partial bootstrap resamples returned.

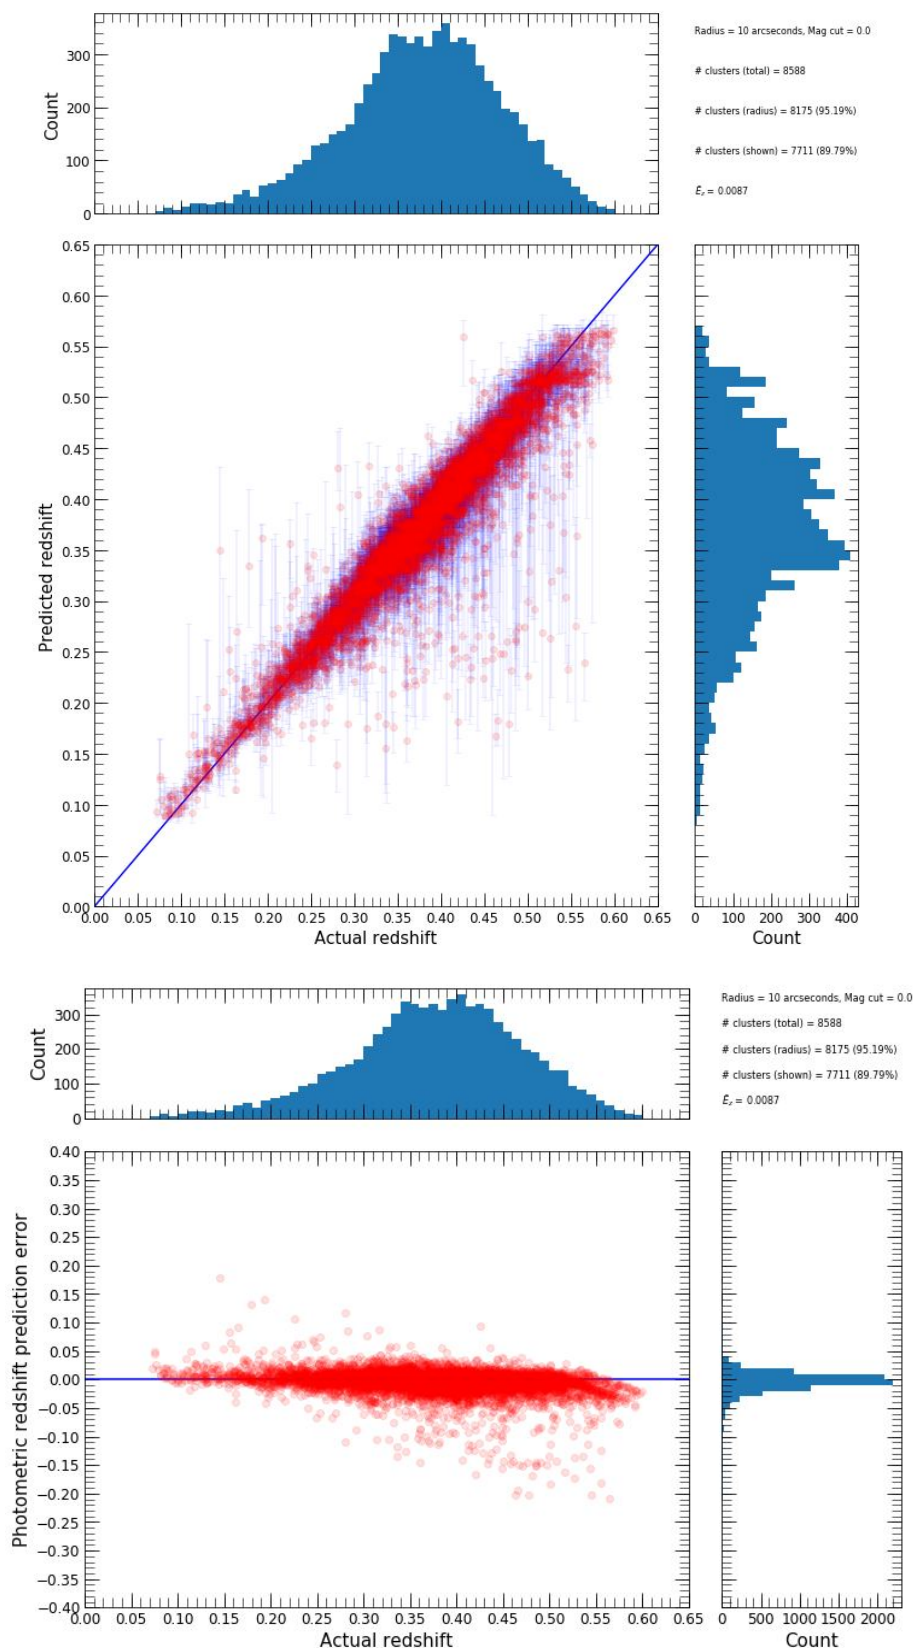

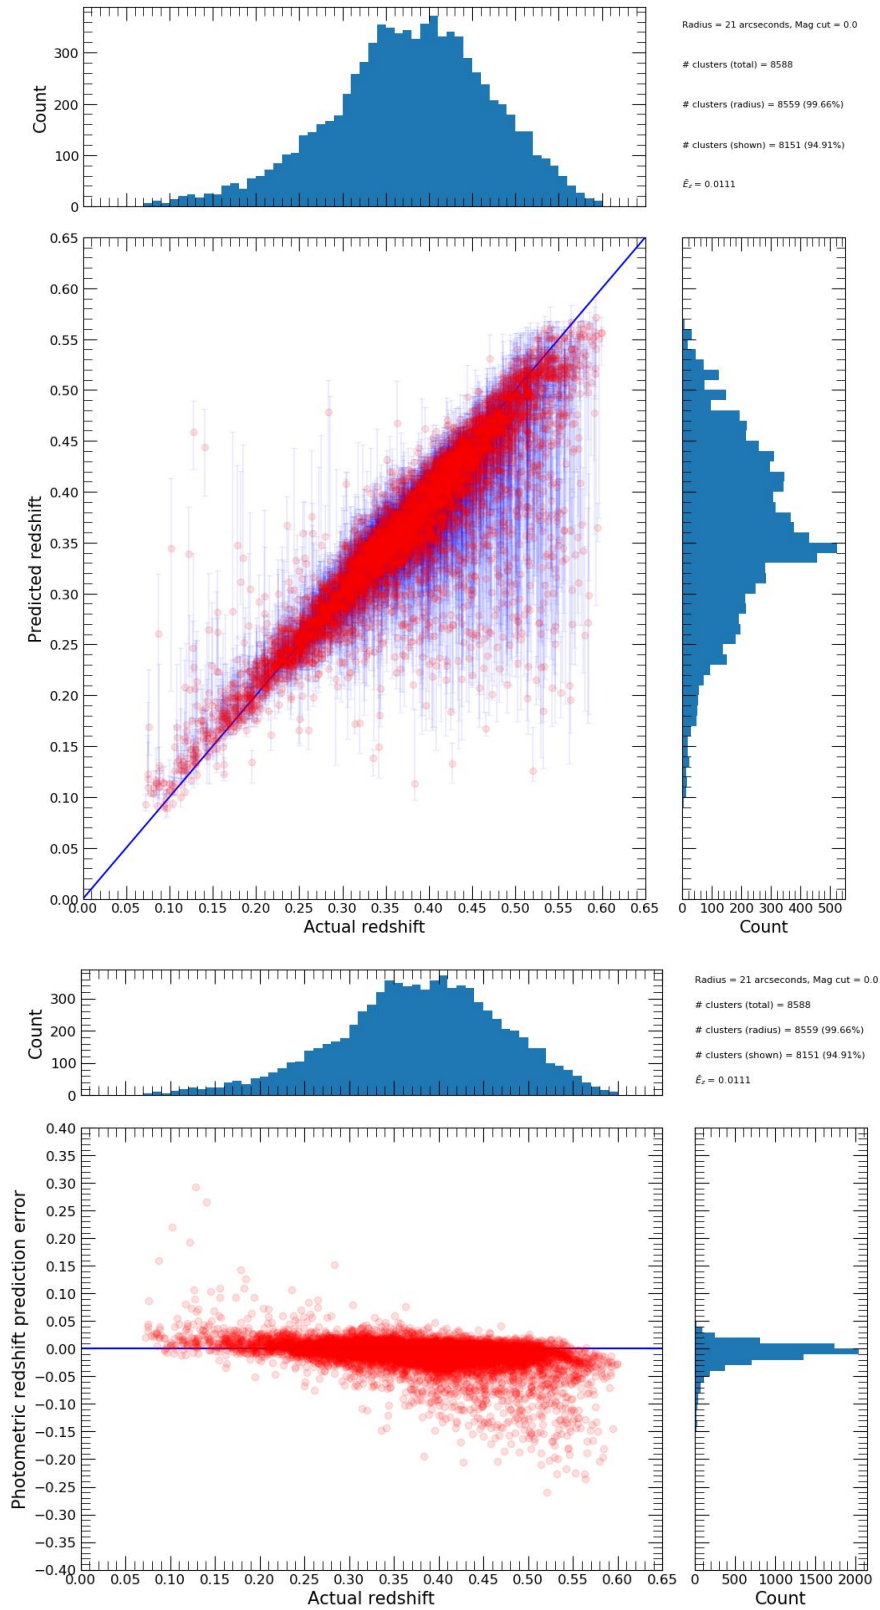

**Figure S9.** Plots displaying the performance of photometric redshift predictions of clusters with low richness, which did not qualify for the MWAR dataset, that had full bootstrap resamples returned within a 21 arcseconds search radius. Top row: Predicted versus ‘actual’ photometric redshift of tested clusters with frequency histograms of the distributions. Bottom row: Non-absolute photometric redshift prediction error versus ‘actual’ redshift of tested clusters with frequency histograms of the distributions. Other: ‘# clusters (total)’ represents the total number of clusters with low richness which did not qualify for the MWAR dataset, ‘# clusters (radius)’ represents the number of clusters with low richness which did not qualify for the MWAR dataset that have observed galaxies within a 21 arcseconds search radius, ‘# clusters (shown)’ represents the number of clusters with low richness which did not qualify for the MWAR dataset that have observed galaxies within a 21 arcseconds search radius with full bootstrap resamples returned,  $\bar{E}_z$  represents the median of photometric redshift prediction errors across all tested clusters within a 21 arcseconds search radius with full bootstrap resamples returned.



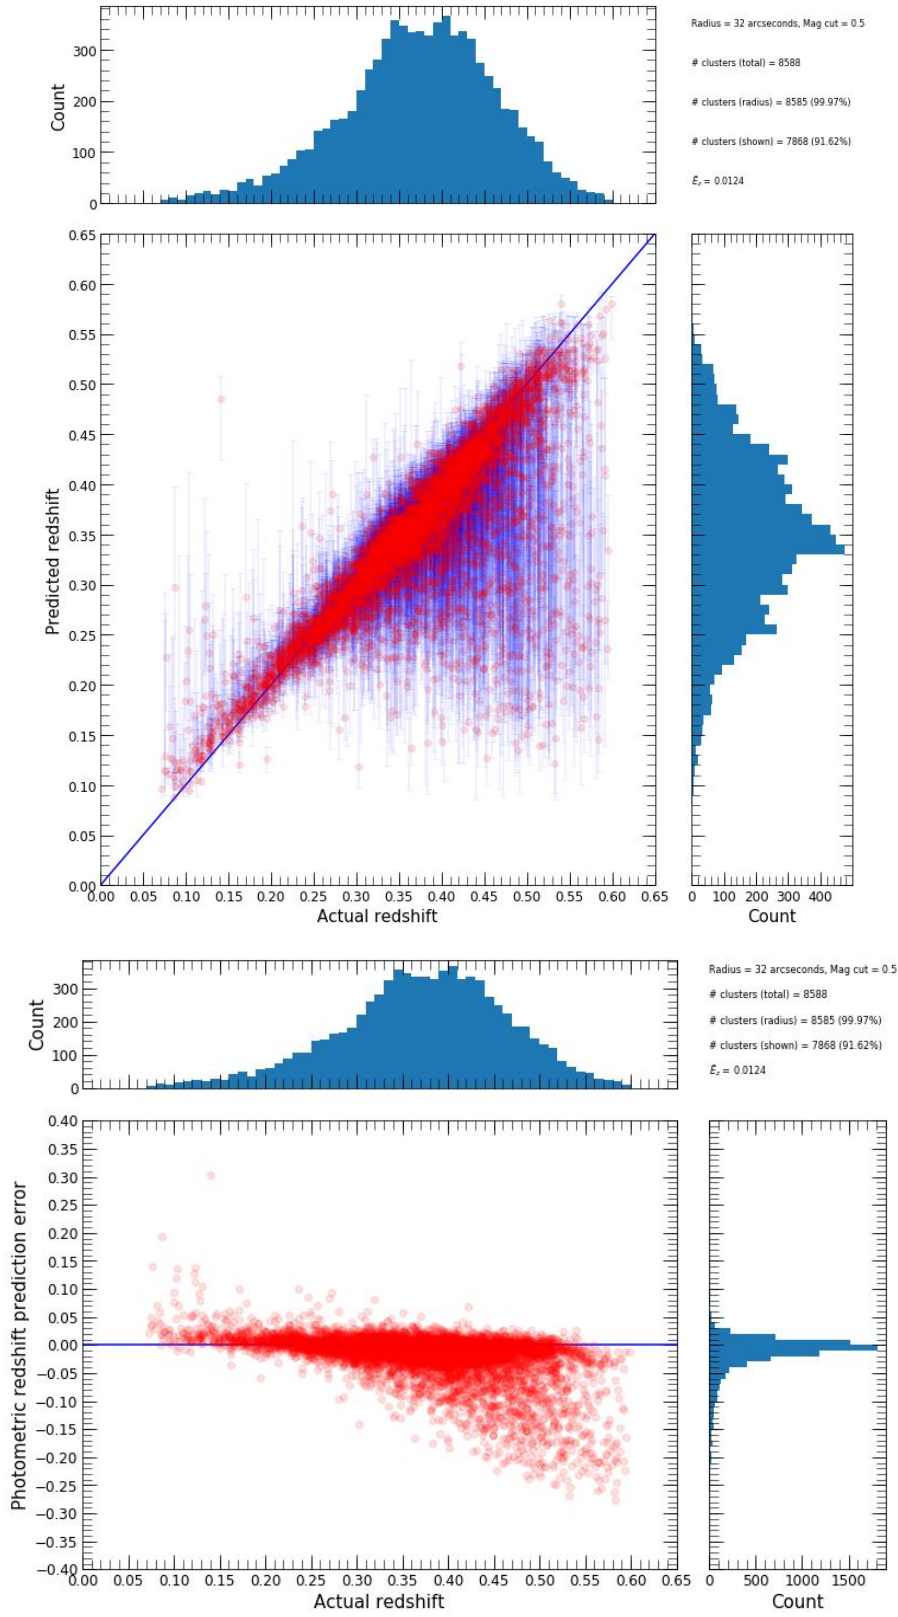

**Figure S10.** Plots displaying the performance of photometric redshift predictions of clusters with low richness, which did not qualify for the MWAR dataset, that had full bootstrap resamples returned within a 32 arcseconds search radius. Top row: Predicted versus 'actual' photometric redshift of tested clusters with frequency histograms of the distributions. Bottom row: Non-absolute photometric redshift prediction error versus 'actual' redshift of tested clusters with frequency histograms of the distributions. Other: '# clusters (total)' represents the total number of clusters with low richness which did not qualify for the MWAR dataset, '# clusters (radius)' represents the number of clusters with low richness which did not qualify for the MWAR dataset that have observed galaxies within a 32 arcseconds search radius, '# clusters (shown)' represents the number of clusters with low richness which did not qualify for the MWAR dataset that have observed galaxies within a 32 arcseconds search radius with full bootstrap resamples returned,  $\bar{E}_z$  represents the median of photometric redshift prediction errors across all tested clusters within a 32 arcseconds search radius with full bootstrap resamples returned.

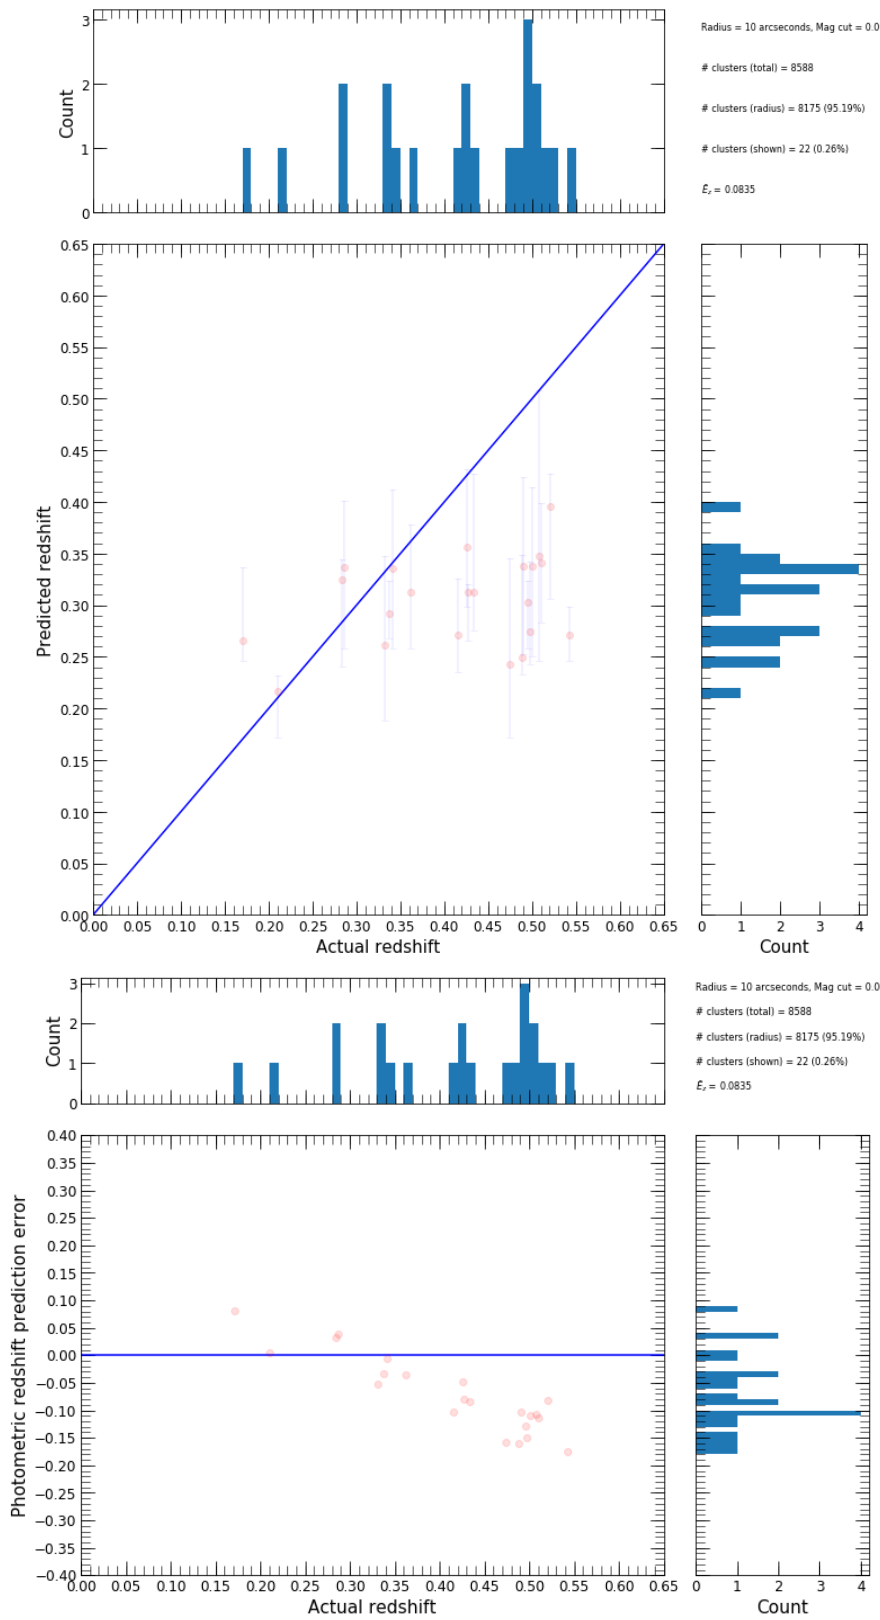

**Figure S11.** Plots displaying the performance of photometric redshift predictions of clusters with low richness, which did not qualify for the MWAR dataset, that had partial bootstrap resamples returned within a 10 arcseconds search radius. Top row: Predicted versus 'actual' photometric redshift of tested clusters with frequency histograms of the distributions. Bottom row: Non-absolute photometric redshift prediction error versus 'actual' redshift of tested clusters with frequency histograms of the distributions. Other: '# clusters (total)' represents the total number of clusters with low richness which did not qualify for the MWAR dataset, '# clusters (radius)' represents the number of clusters with low richness which did not qualify for the MWAR dataset that have observed galaxies within a 10 arcseconds search radius, '# clusters (shown)' represents the number of clusters with low richness which did not qualify for the MWAR dataset that have observed galaxies within a 10 arcseconds search radius with partial bootstrap resamples returned,  $\bar{E}_z$  represents the median of photometric redshift prediction errors across all tested clusters within a 10 arcseconds search radius with partial bootstrap resamples returned.

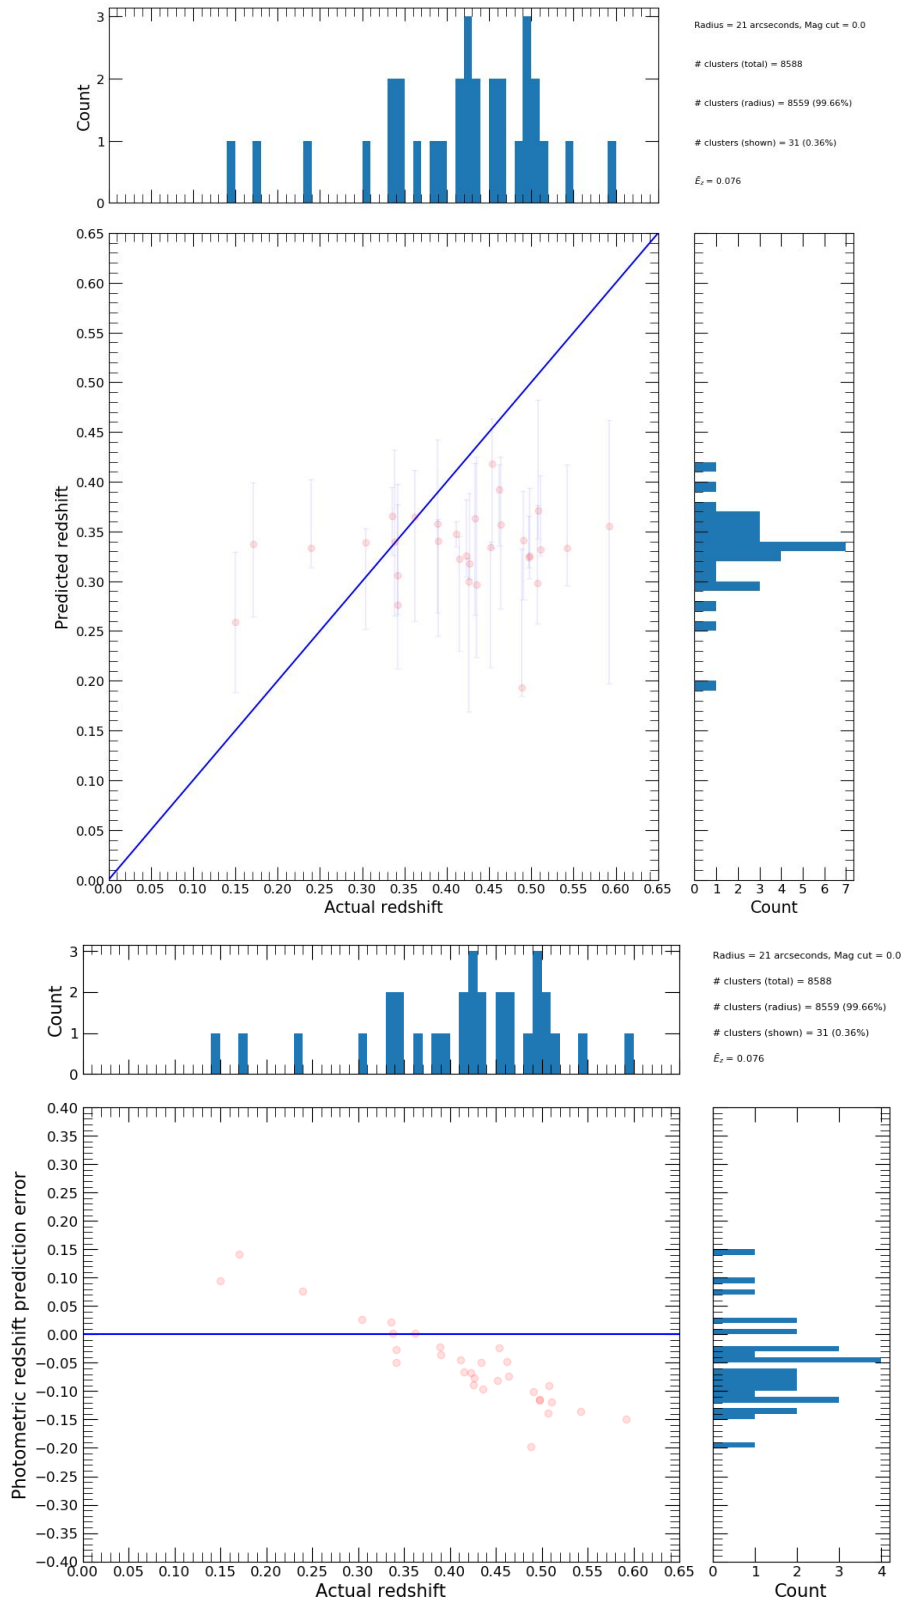

**Figure S12.** Plots displaying the performance of photometric redshift predictions of clusters with low richness, which did not qualify for the MWAR dataset, that had partial bootstrap resamples returned within a 21 arcseconds search radius. Top row: Predicted versus 'actual' photometric redshift of tested clusters with frequency histograms of the distributions. Bottom row: Non-absolute photometric redshift prediction error versus 'actual' redshift of tested clusters with frequency histograms of the distributions. Other: '# clusters (total)' represents the total number of clusters with low richness which did not qualify for the MWAR dataset, '# clusters (radius)' represents the number of clusters with low richness which did not qualify for the MWAR dataset that have observed galaxies within a 21 arcseconds search radius, '# clusters (shown)' represents the number of clusters with low richness which did not qualify for the MWAR dataset that have observed galaxies within a 21 arcseconds search radius with partial bootstrap resamples returned,  $\bar{E}_z$  represents the median of photometric redshift prediction errors across all tested clusters within a 21 arcseconds search radius with partial bootstrap resamples returned.





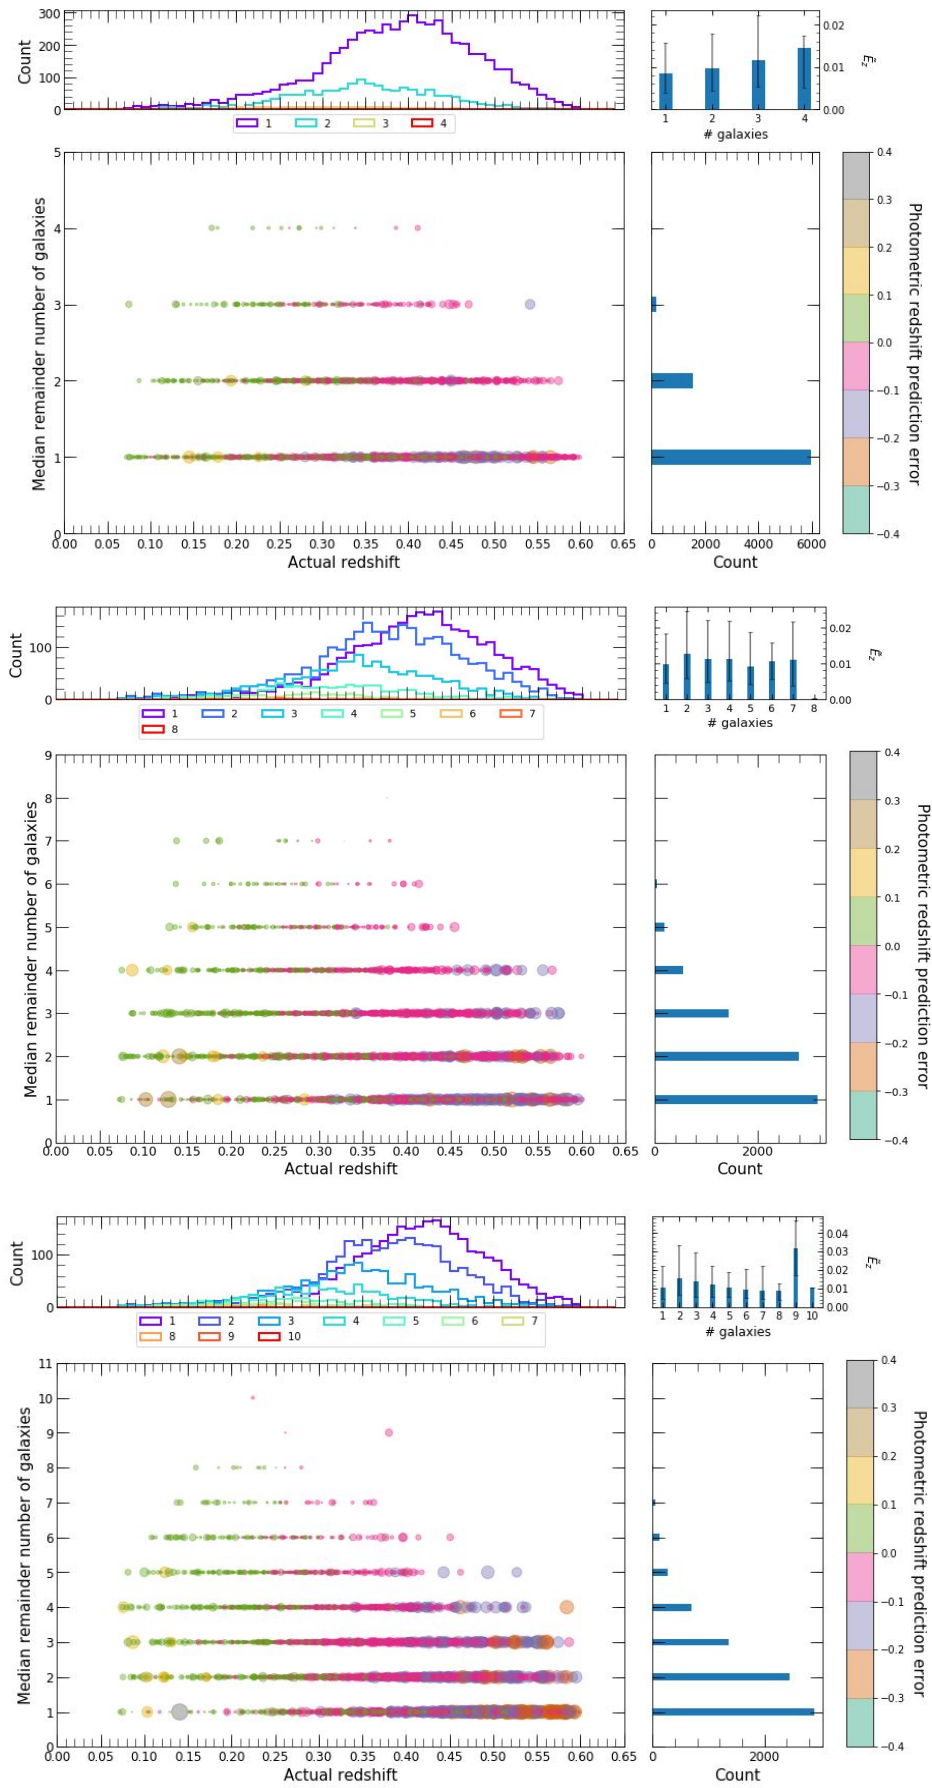

**Figure S14.** Plots displaying the number of galaxies used in photometric redshift predictions of clusters with low richness versus 'actual' redshift of tested galaxies, which did not qualify for the MWAR dataset, where predictions had full bootstrap resamples returned within a 10 (top row), 21 (middle row) and 32 (bottom row) arcseconds search radius. It should be noted that the size of individual points change in relation to the value of the non-absolute photometric redshift prediction error. Frequency histograms of the distributions are also shown.  $\bar{E}_z$  represents the median of photometric redshift prediction errors across all tested clusters for each number of galaxies bin.

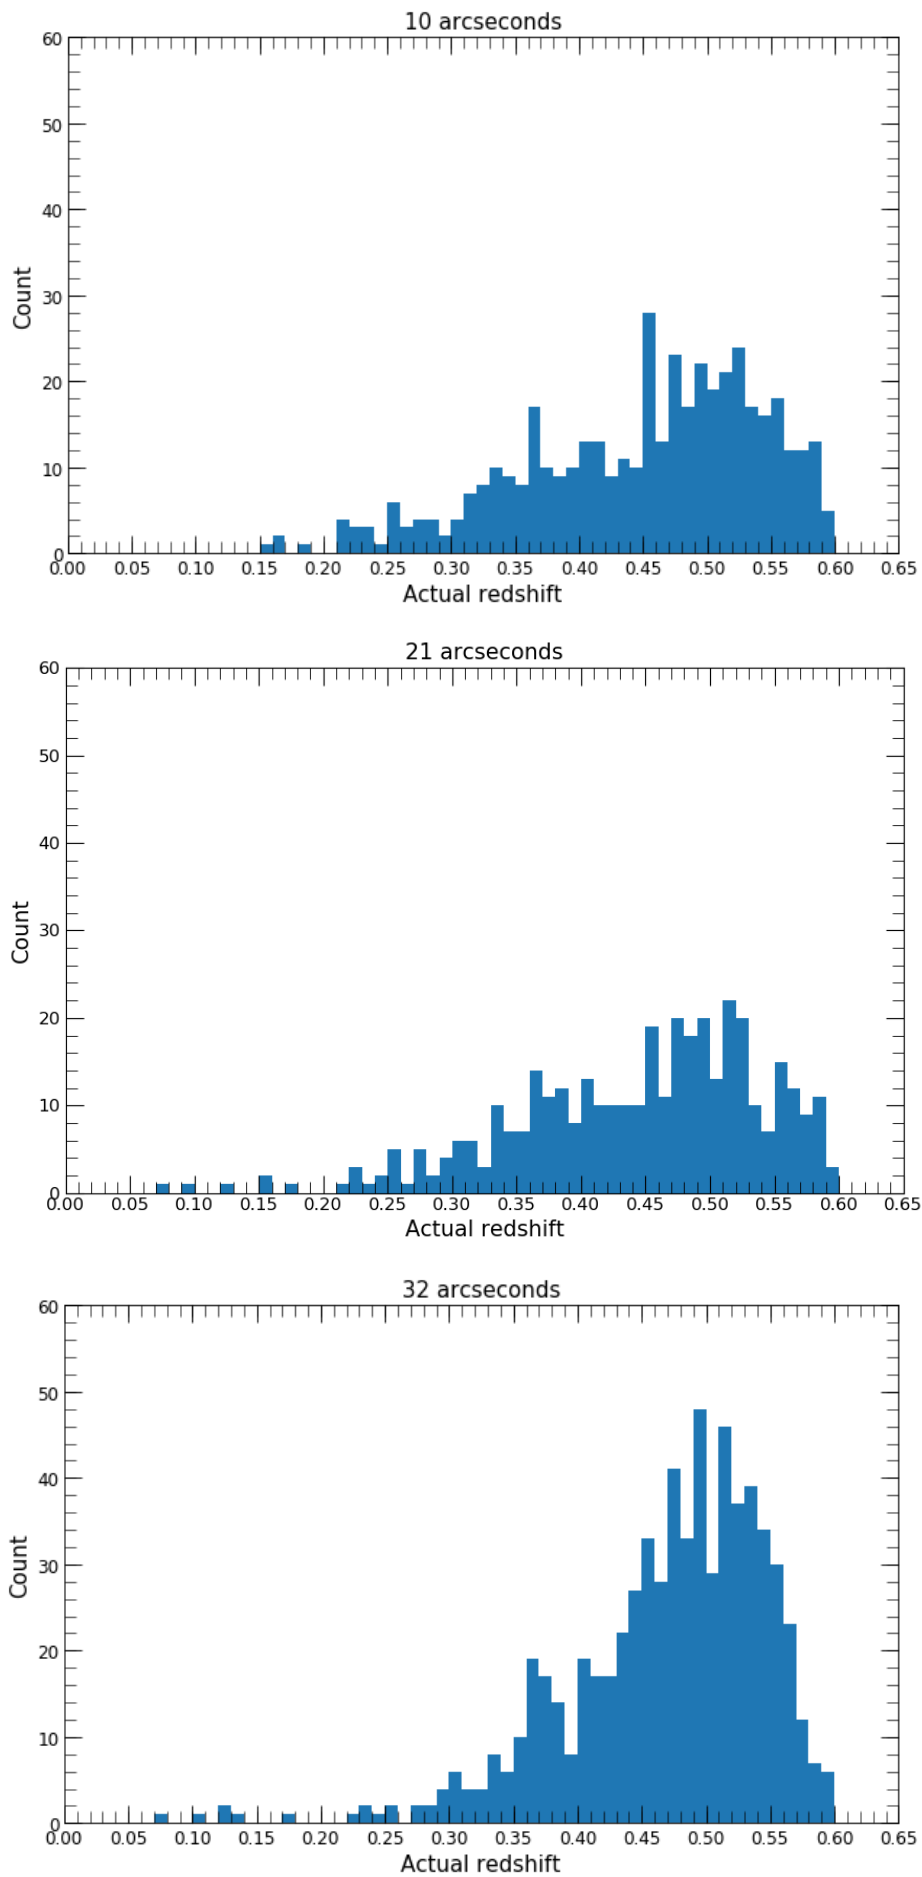

**Figure S15.** Frequency histograms displaying the ‘actual’ redshift distributions of clusters with low richness, which did not qualify for the MWAR dataset, that had no bootstrap resamples returned within a 10 (top row), 21 (middle row) and 32 (bottom row) arcseconds search radius.

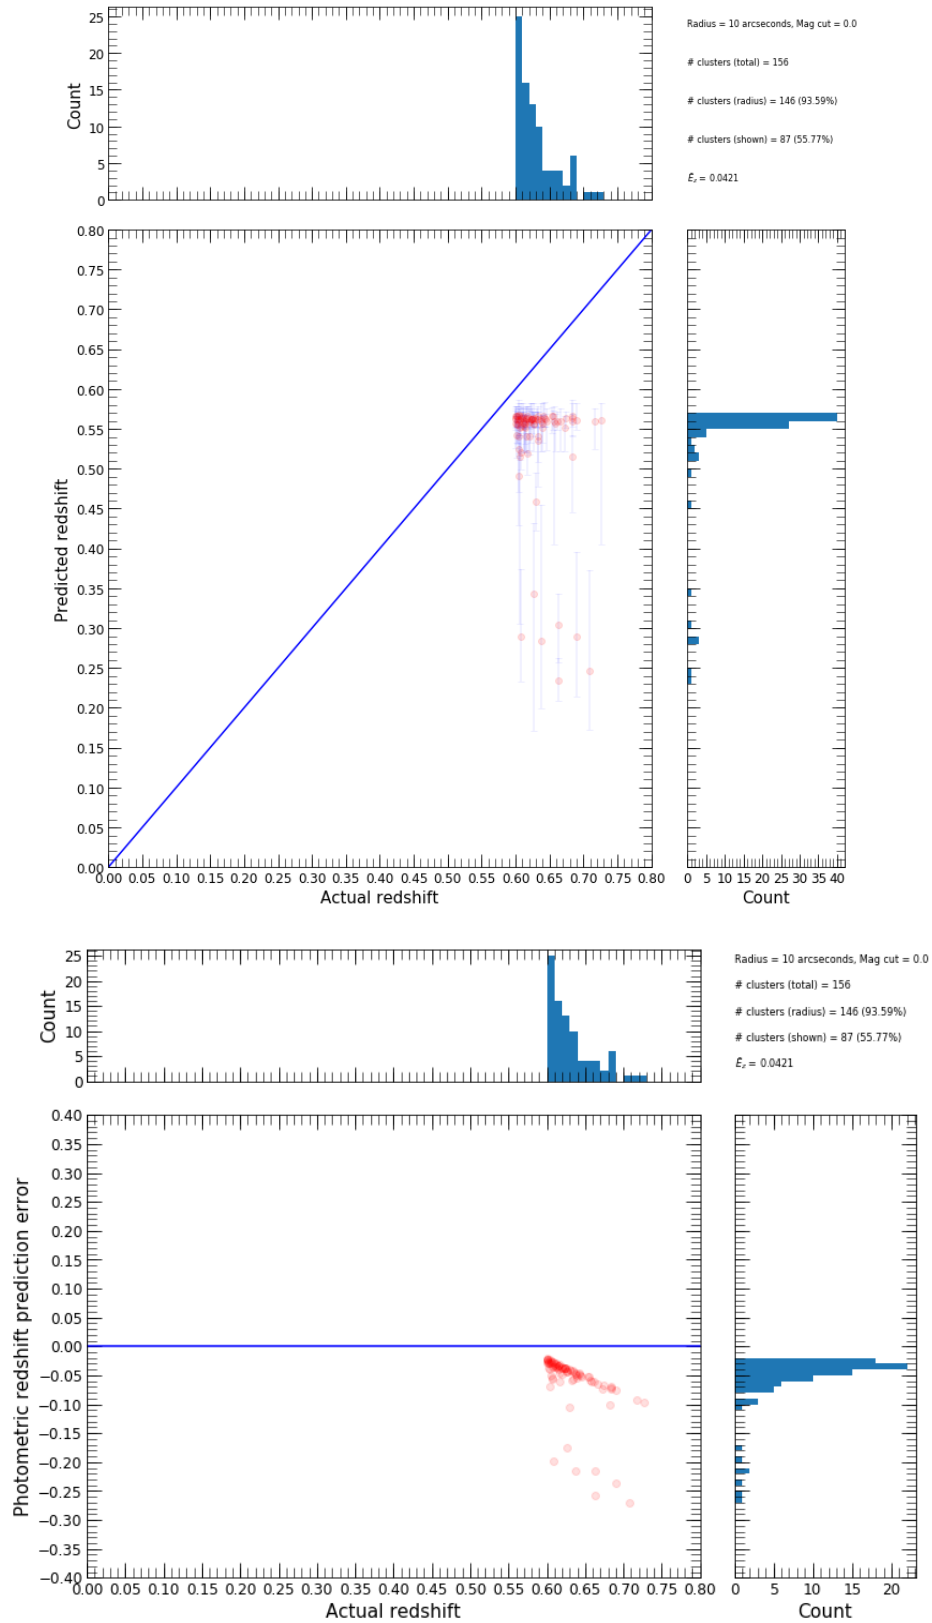

**Figure S16.** Plots displaying the performance of photometric redshift predictions of clusters at high redshift, which did not qualify for the WNMR dataset, that had full bootstrap resamples returned within a 10 arcseconds search radius. Top row: Predicted versus 'actual' photometric redshift of tested clusters with frequency histograms of the distributions. Bottom row: Non-absolute photometric redshift prediction error versus 'actual' redshift of tested clusters with frequency histograms of the distributions. Other: '# clusters (total)' represents the total number of clusters at high redshift which did not qualify for the WNMR dataset, '# clusters (radius)' represents the number of clusters at high redshift which did not qualify for the WNMR dataset that have observed galaxies within a 10 arcseconds search radius, '# clusters (shown)' represents the number of clusters at high redshift which did not qualify for the WNMR dataset that have observed galaxies within a 10 arcseconds search radius with full bootstrap resamples returned,  $\bar{E}_z$  represents the median of photometric redshift prediction errors across all tested clusters within a 10 arcseconds search radius with full bootstrap resamples returned.

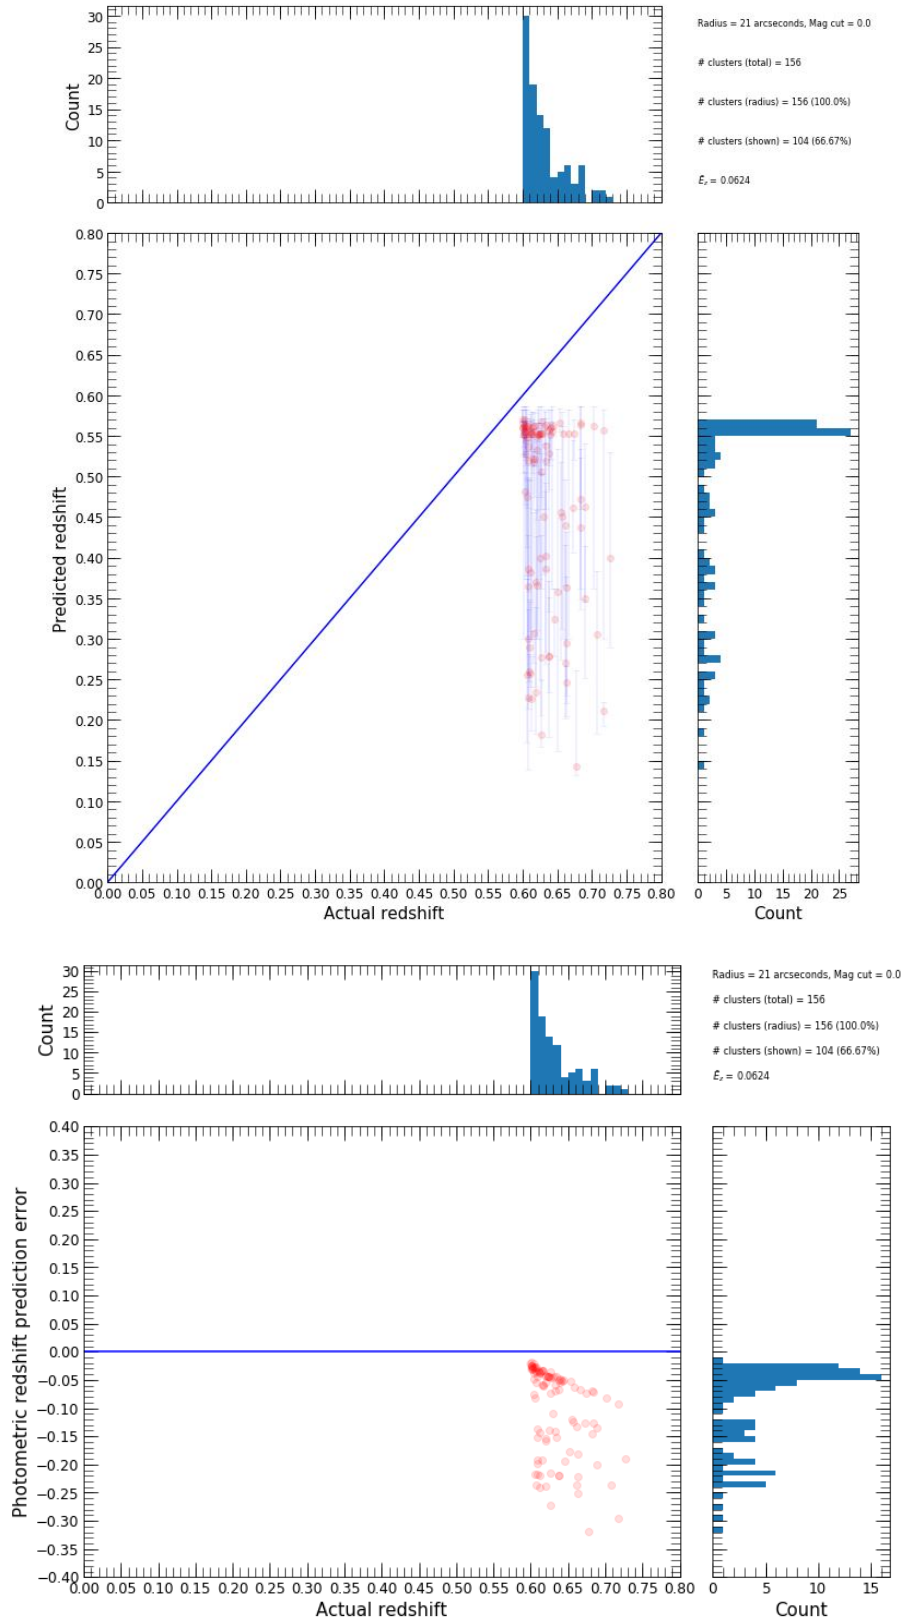

**Figure S17.** Plots displaying the performance of photometric redshift predictions of clusters at high redshift, which did not qualify for the WNMR dataset, that had full bootstrap resamples returned within a 21 arcseconds search radius. Top row: Predicted versus 'actual' photometric redshift of tested clusters with frequency histograms of the distributions. Bottom row: Non-absolute photometric redshift prediction error versus 'actual' redshift of tested clusters with frequency histograms of the distributions. Other: '# clusters (total)' represents the total number of clusters at high redshift which did not qualify for the WNMR dataset, '# clusters (radius)' represents the number of clusters at high redshift which did not qualify for the WNMR dataset that have observed galaxies within a 21 arcseconds search radius, '# clusters (shown)' represents the number of clusters at high redshift which did not qualify for the WNMR dataset that have observed galaxies within a 21 arcseconds search radius with full bootstrap resamples returned,  $\bar{E}_z$  represents the median of photometric redshift prediction errors across all tested clusters within a 21 arcseconds search radius with full bootstrap resamples returned.

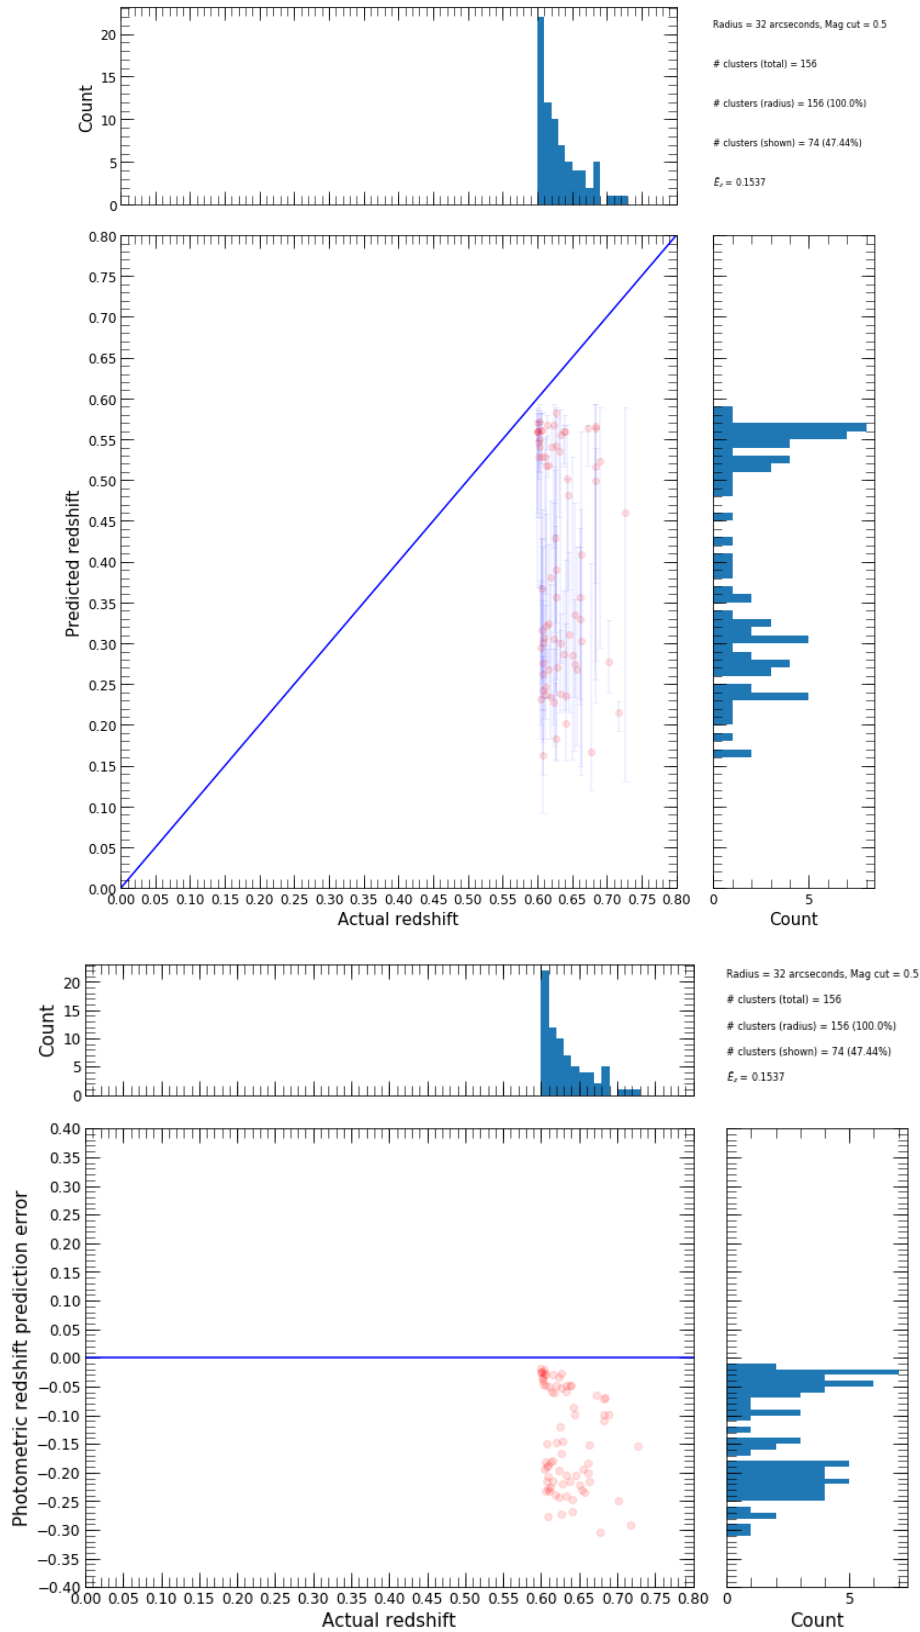

**Figure S18.** Plots displaying the performance of photometric redshift predictions of clusters at high redshift, which did not qualify for the WNMR dataset, that had full bootstrap resamples returned within a 32 arcseconds search radius. Top row: Predicted versus 'actual' photometric redshift of tested clusters with frequency histograms of the distributions. Bottom row: Non-absolute photometric redshift prediction error versus 'actual' redshift of tested clusters with frequency histograms of the distributions. Other: '# clusters (total)' represents the total number of clusters at high redshift which did not qualify for the WNMR dataset, '# clusters (radius)' represents the number of clusters at high redshift which did not qualify for the WNMR dataset that have observed galaxies within a 32 arcseconds search radius, '# clusters (shown)' represents the number of clusters at high redshift which did not qualify for the WNMR dataset that have observed galaxies within a 32 arcseconds search radius with full bootstrap resamples returned,  $\bar{E}_z$  represents the median of photometric redshift prediction errors across all tested clusters within a 32 arcseconds search radius with full bootstrap resamples returned.

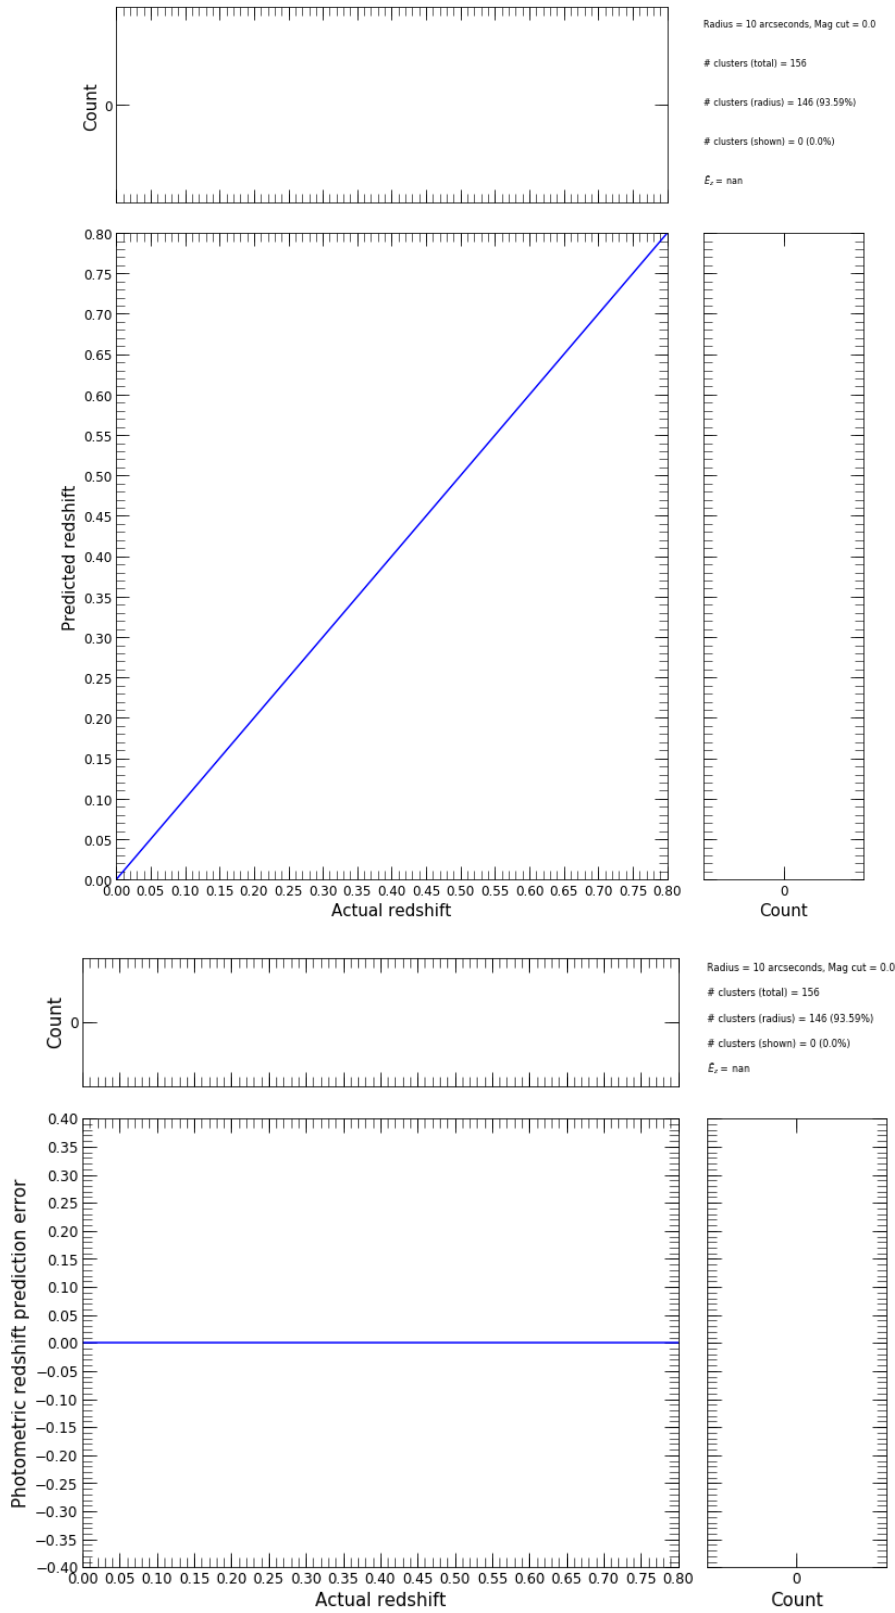

**Figure S19.** Plots displaying the performance of photometric redshift predictions of clusters at high redshift, which did not qualify for the WNMN dataset, that had partial bootstrap resamples returned within a 10 arcseconds search radius. It should be noted that in this figure there were no resultant predictions made by the tuned model, as none of the clusters met the conditions. Top row: Predicted versus 'actual' photometric redshift of tested clusters with frequency histograms of the distributions. Bottom row: Non-absolute photometric redshift prediction error versus 'actual' redshift of tested clusters with frequency histograms of the distributions. Other: '# clusters (total)' represents the total number of clusters at high redshift which did not qualify for the WNMN dataset, '# clusters (radius)' represents the number of clusters at high redshift which did not qualify for the WNMN dataset that have observed galaxies within a 10 arcseconds search radius, '# clusters (shown)' represents the number of clusters at high redshift which did not qualify for the WNMN dataset that have observed galaxies within a 10 arcseconds search radius with partial bootstrap resamples returned,  $E_z$  represents the median of photometric redshift prediction errors across all tested clusters within a 10 arcseconds search radius with partial bootstrap resamples returned.



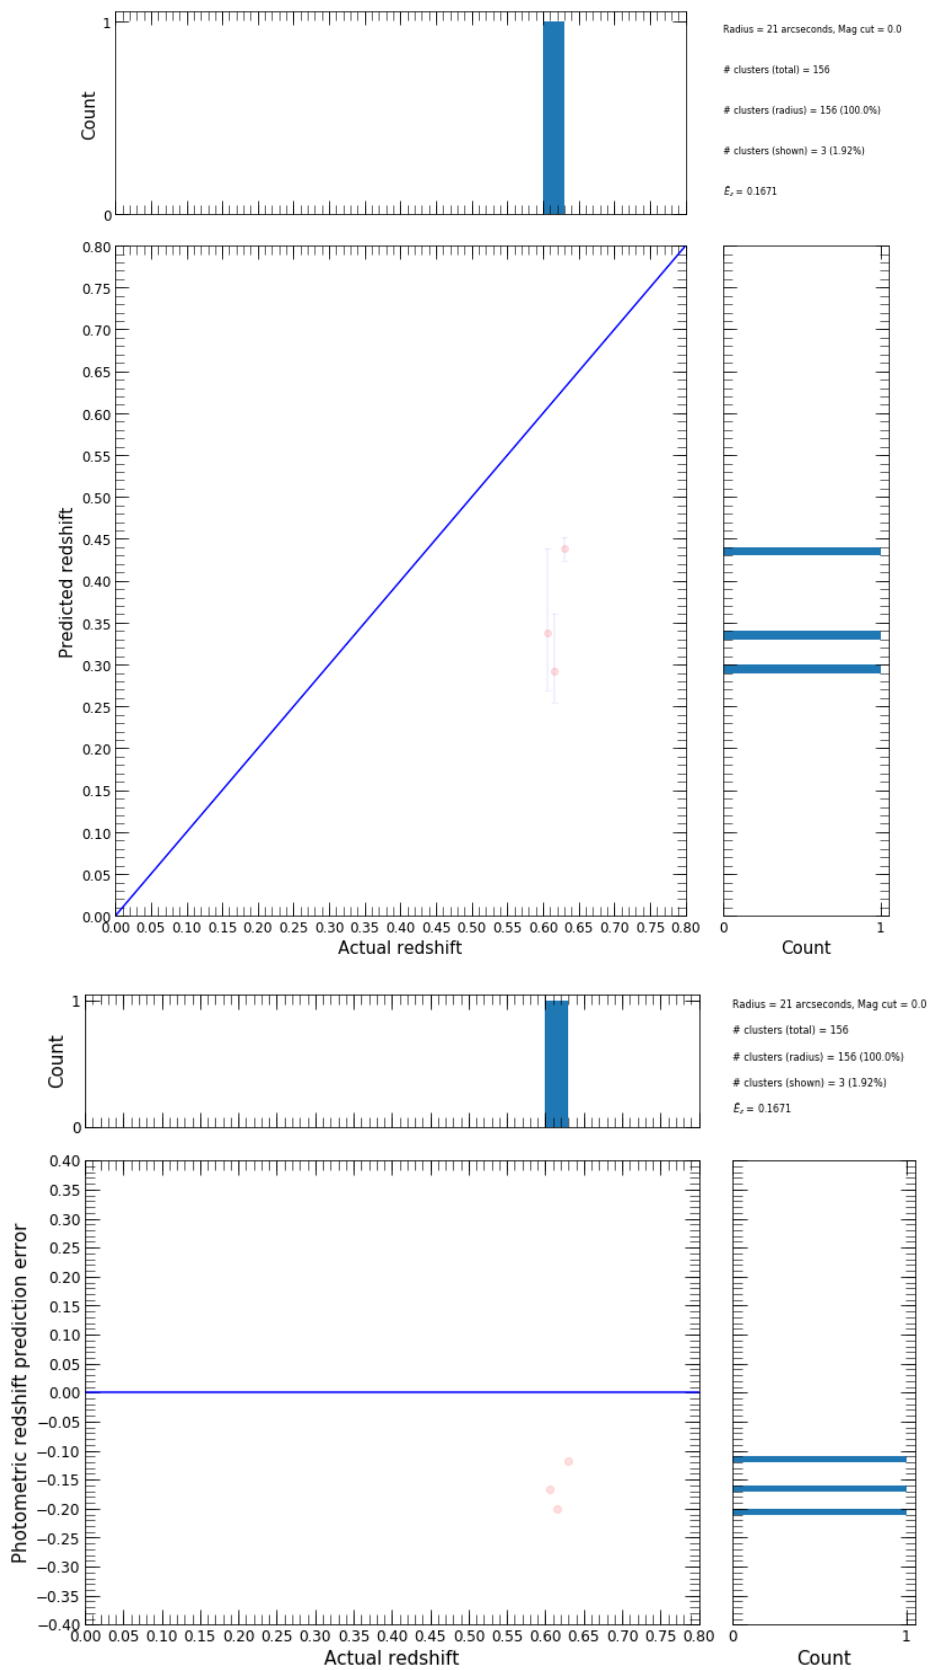

**Figure S20.** Plots displaying the performance of photometric redshift predictions of clusters at high redshift, which did not qualify for the WNMN dataset, that had partial bootstrap resamples returned within a 21 arcseconds search radius. Top row: Predicted versus 'actual' photometric redshift of tested clusters with frequency histograms of the distributions. Bottom row: Non-absolute photometric redshift prediction error versus 'actual' redshift of tested clusters with frequency histograms of the distributions. Other: '# clusters (total)' represents the total number of clusters at high redshift which did not qualify for the WNMN dataset, '# clusters (radius)' represents the number of clusters at high redshift which did not qualify for the WNMN dataset that have observed galaxies within a 21 arcseconds search radius, '# clusters (shown)' represents the number of clusters at high redshift which did not qualify for the WNMN dataset that have observed galaxies within a 21 arcseconds search radius with partial bootstrap resamples returned,  $\bar{E}_z$  represents the median of photometric redshift prediction errors across all tested clusters within a 21 arcseconds search radius with partial bootstrap resamples returned.



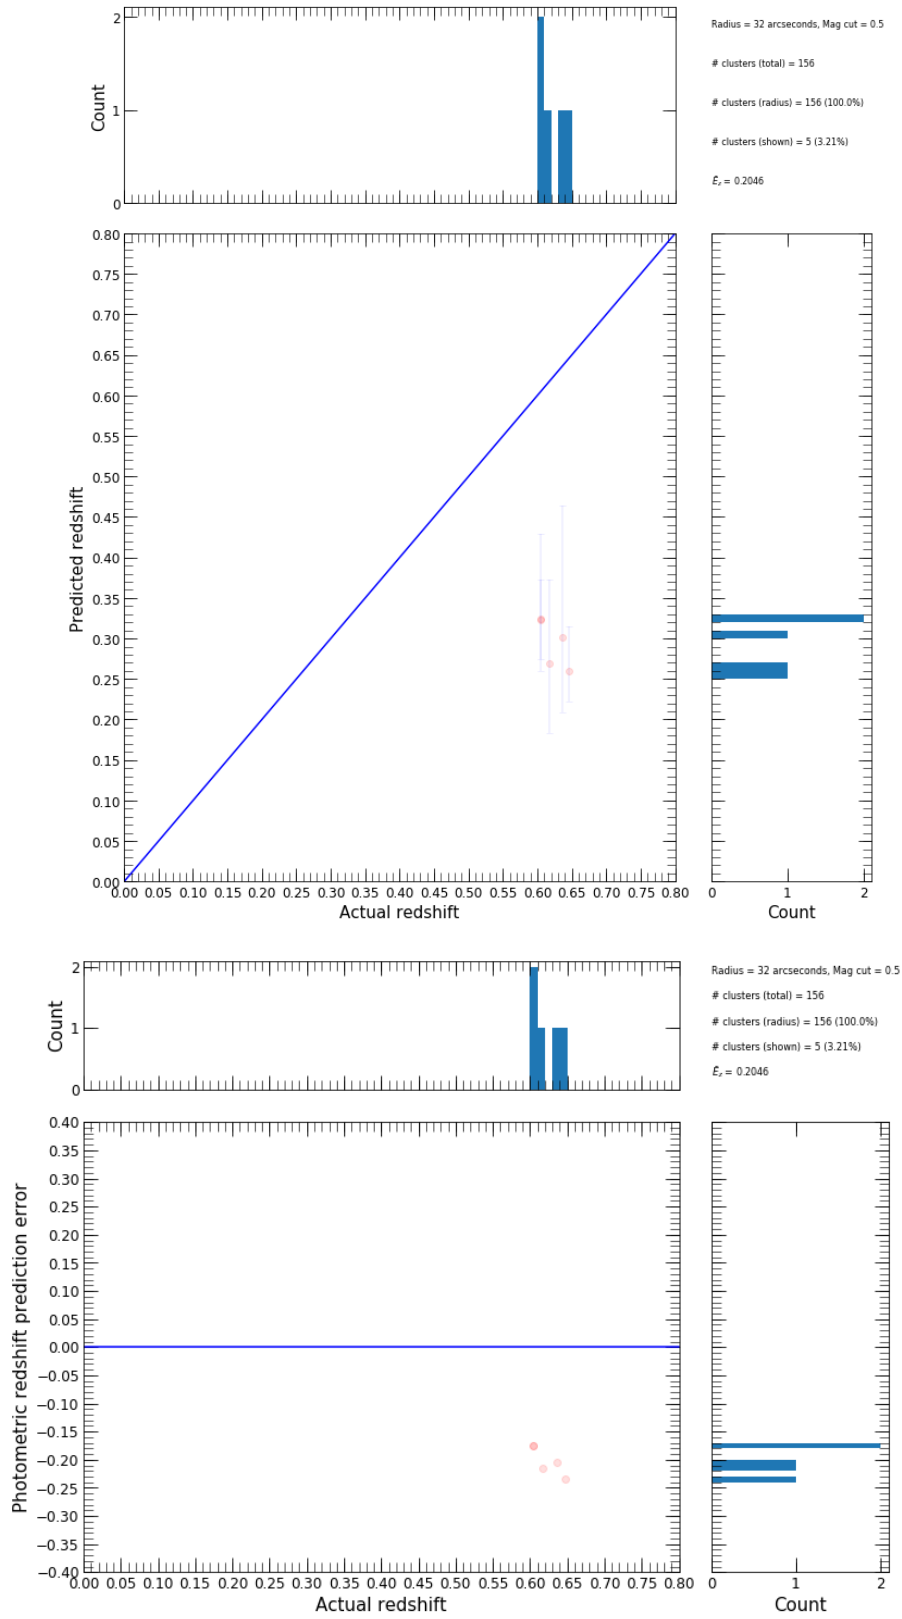

**Figure S21.** Plots displaying the performance of photometric redshift predictions of clusters at high redshift, which did not qualify for the WNMR dataset, that had partial bootstrap resamples returned within a 32 arcseconds search radius. Top row: Predicted versus 'actual' photometric redshift of tested clusters with frequency histograms of the distributions. Bottom row: Non-absolute photometric redshift prediction error versus 'actual' redshift of tested clusters with frequency histograms of the distributions. Other: '# clusters (total)' represents the total number of clusters at high redshift which did not qualify for the WNMR dataset, '# clusters (radius)' represents the number of clusters at high redshift which did not qualify for the WNMR dataset that have observed galaxies within a 32 arcseconds search radius, '# clusters (shown)' represents the number of clusters at high redshift which did not qualify for the WNMR dataset that have observed galaxies within a 32 arcseconds search radius with partial bootstrap resamples returned,  $\bar{E}_z$  represents the median of photometric redshift prediction errors across all tested clusters within a 32 arcseconds search radius with partial bootstrap resamples returned.

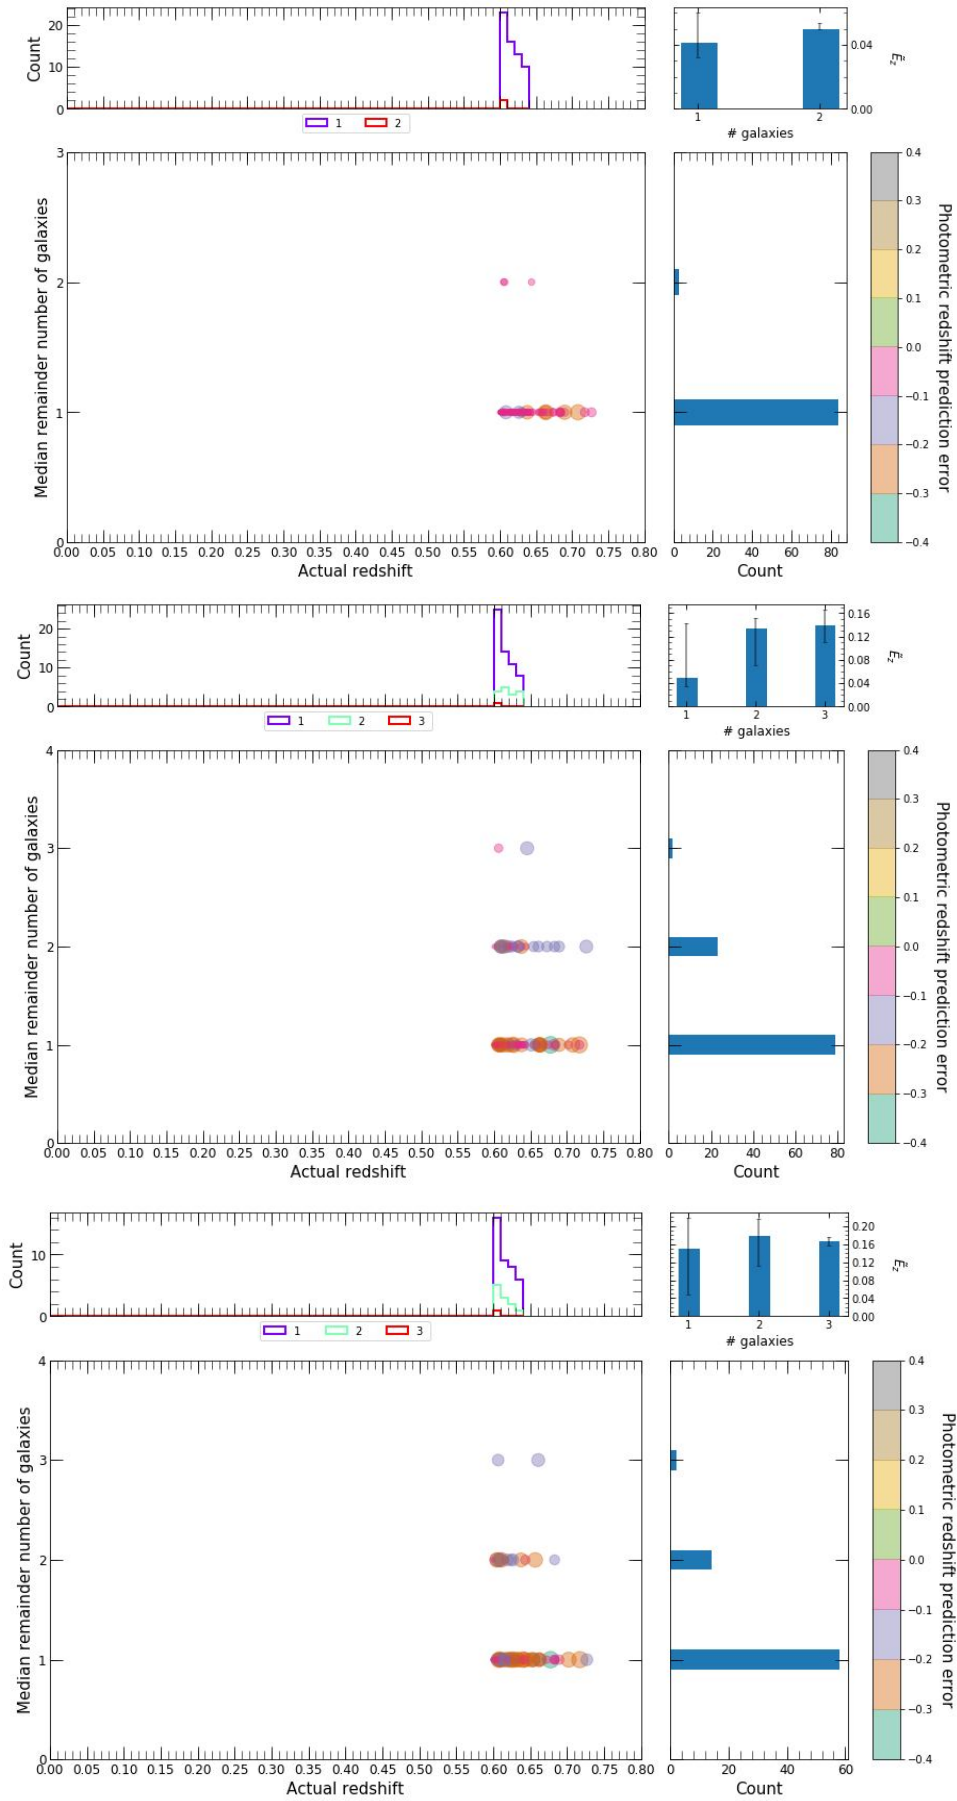

**Figure S22.** Plots displaying the number of galaxies used in photometric redshift predictions of clusters at high redshift versus 'actual' redshift of tested clusters, which did not qualify for the WNMR dataset, where predictions had full bootstrap resamples returned within a 10 (top row), 21 (middle row) and 32 (bottom row) arcseconds search radius. It should be noted that the size of individual points change in relation to the value of the non-absolute photometric redshift prediction error. Frequency histograms of the distributions are also shown.  $\bar{E}_z$  represents the median of photometric redshift prediction errors across all tested clusters for each number of galaxies bin.

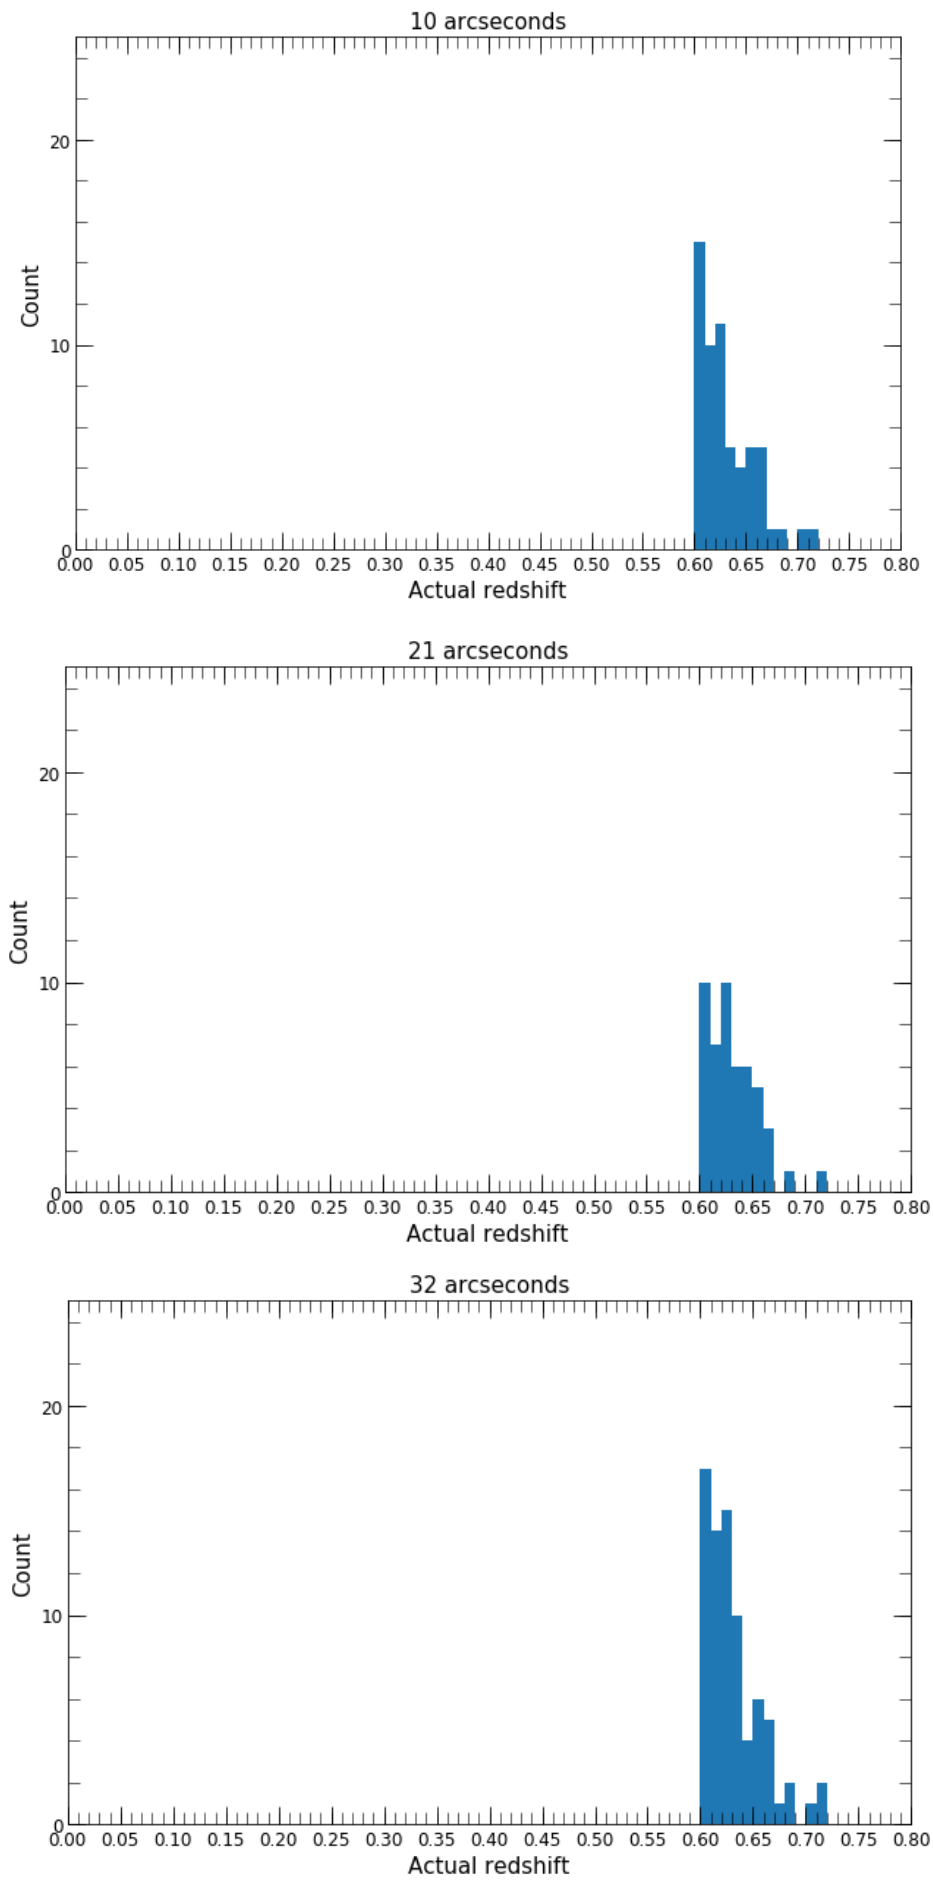

**Figure S23.** Frequency histograms displaying the ‘actual’ redshift distributions of clusters at high redshift, which did not qualify for the WNMR dataset, that had no bootstrap resamples returned within a 10 (top row), 21 (middle row) and 32 (bottom row) arcseconds search radius.

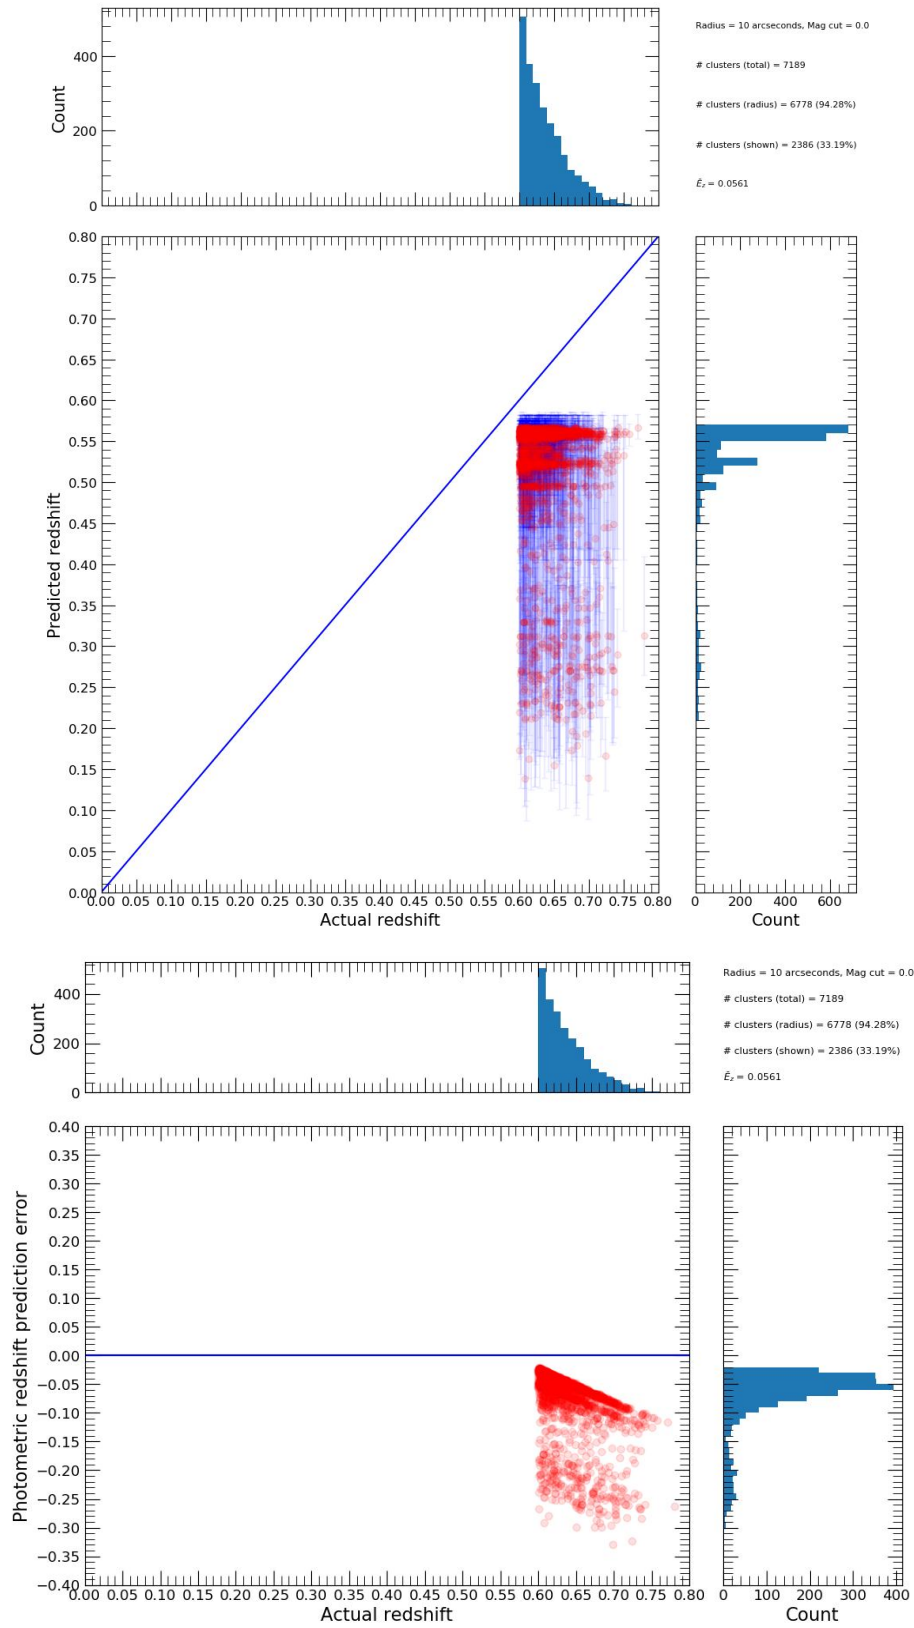

**Figure S24.** Plots displaying the performance of photometric redshift predictions of clusters at high redshift with low richness, which did not qualify for the WNMN dataset, that had full bootstrap resamples returned within a 10 arcseconds search radius. Top row: Predicted versus 'actual' photometric redshift of tested clusters with frequency histograms of the distributions. Bottom row: Non-absolute photometric redshift prediction error versus 'actual' redshift of tested clusters with frequency histograms of the distributions. Other: '# clusters (total)' represents the total number of clusters at high redshift with low richness which did not qualify for the WNMN dataset, '# clusters (radius)' represents the number of clusters at high redshift with low richness which did not qualify for the WNMN dataset that have observed galaxies within a 10 arcseconds search radius, '# clusters (shown)' represents the number of clusters at high redshift with low richness which did not qualify for the WNMN dataset that have observed galaxies within a 10 arcseconds search radius with full bootstrap resamples returned,  $\bar{E}_z$  represents the median of photometric redshift prediction errors across all tested clusters within a 10 arcseconds search radius with full bootstrap resamples returned.

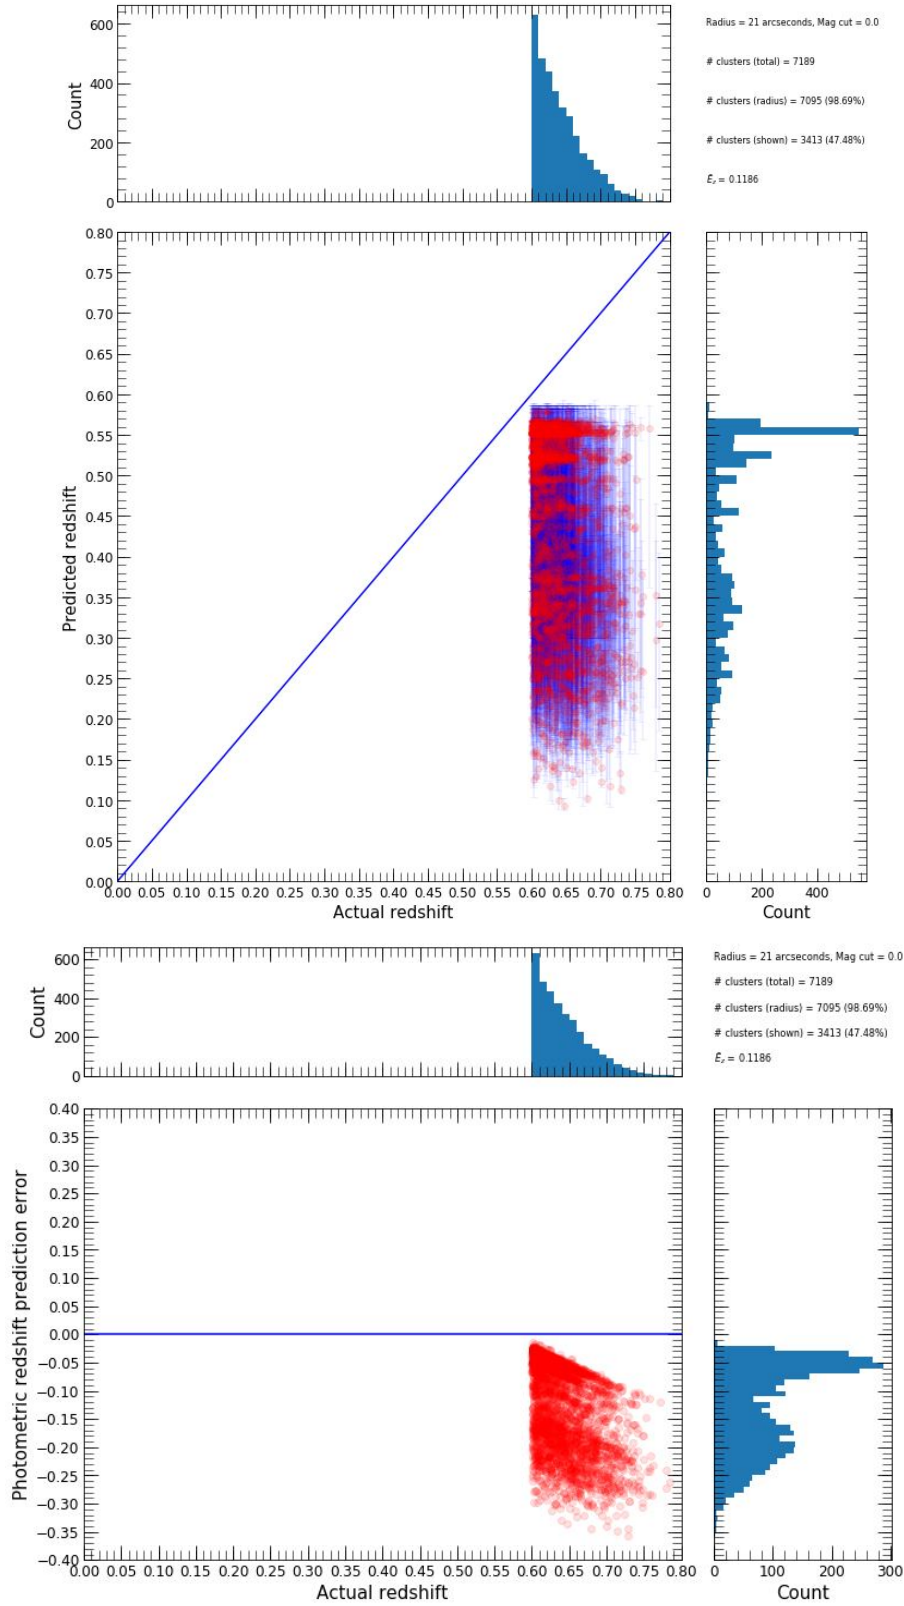

**Figure S25.** Plots displaying the performance of photometric redshift predictions of clusters at high redshift with low richness, which did not qualify for the WNMR dataset, that had full bootstrap resamples returned within a 21 arcseconds search radius. Top row: Predicted versus 'actual' photometric redshift of tested clusters with frequency histograms of the distributions. Bottom row: Non-absolute photometric redshift prediction error versus 'actual' redshift of tested clusters with frequency histograms of the distributions. Other: '# clusters (total)' represents the total number of clusters at high redshift with low richness which did not qualify for the WNMR dataset, '# clusters (radius)' represents the number of clusters at high redshift with low richness which did not qualify for the WNMR dataset that have observed galaxies within a 21 arcseconds search radius, '# clusters (shown)' represents the number of clusters at high redshift with low richness which did not qualify for the WNMR dataset that have observed galaxies within a 21 arcseconds search radius with full bootstrap resamples returned,  $\bar{E}_z$  represents the median of photometric redshift prediction errors across all tested clusters within a 21 arcseconds search radius with full bootstrap resamples returned.

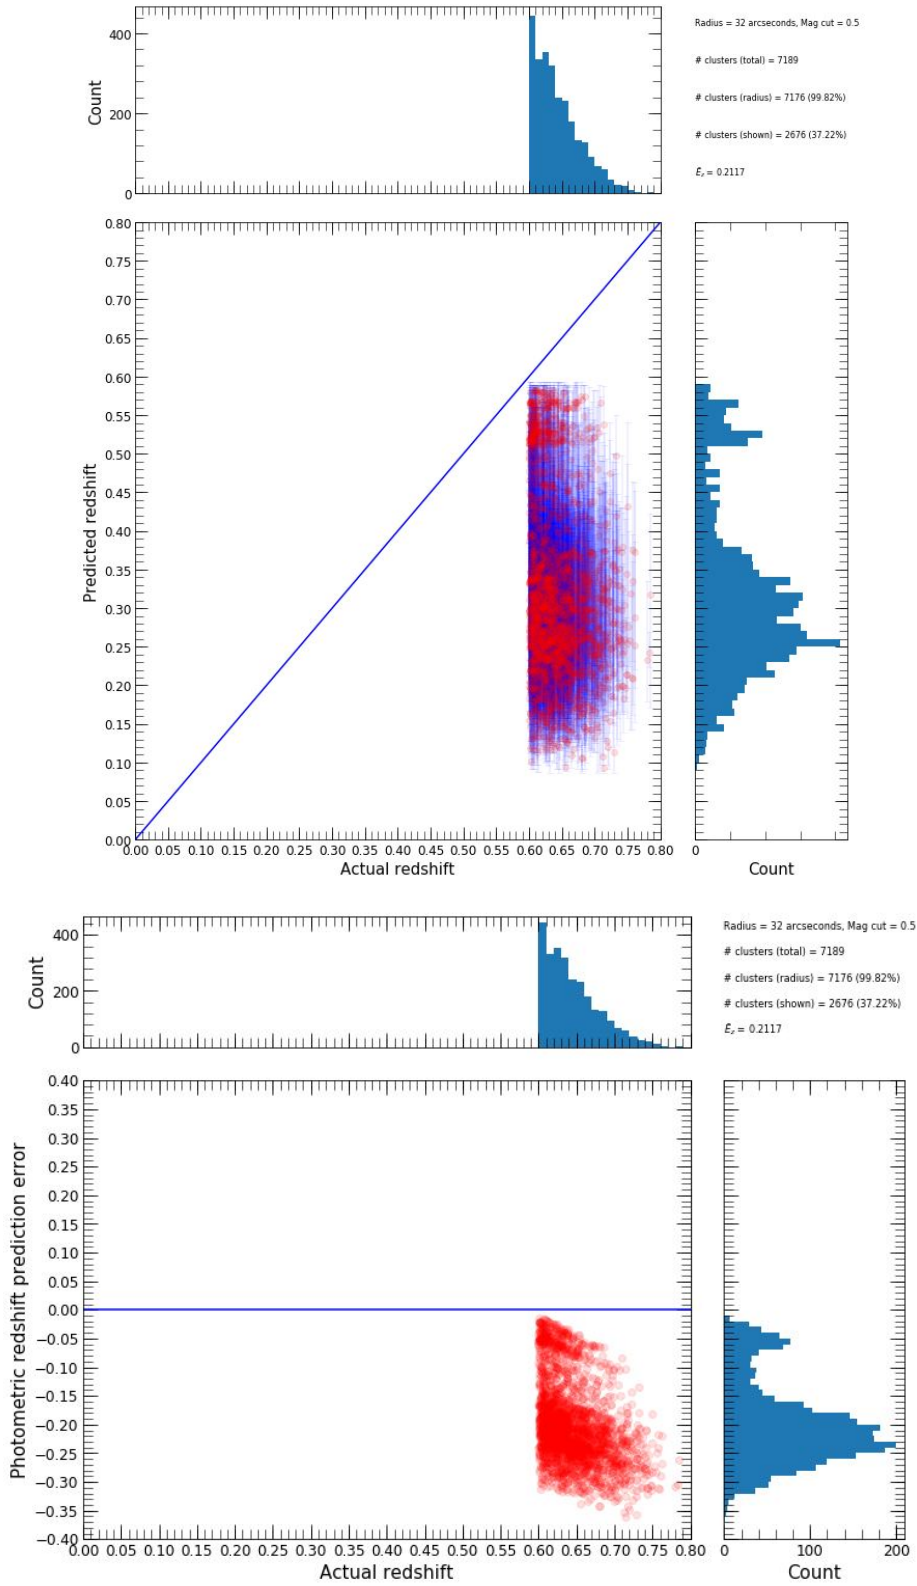

**Figure S26.** Plots displaying the performance of photometric redshift predictions of clusters at high redshift with low richness, which did not qualify for the WNMR dataset, that had full bootstrap resamples returned within a 32 arcseconds search radius. Top row: Predicted versus 'actual' photometric redshift of tested clusters with frequency histograms of the distributions. Bottom row: Non-absolute photometric redshift prediction error versus 'actual' redshift of tested clusters with frequency histograms of the distributions. Other: '# clusters (total)' represents the total number of clusters at high redshift with low richness which did not qualify for the WNMR dataset, '# clusters (radius)' represents the number of clusters at high redshift with low richness which did not qualify for the WNMR dataset that have observed galaxies within a 32 arcseconds search radius, '# clusters (shown)' represents the number of clusters at high redshift with low richness which did not qualify for the WNMR dataset that have observed galaxies within a 32 arcseconds search radius with full bootstrap resamples returned,  $\bar{E}_z$  represents the median of photometric redshift prediction errors across all tested clusters within a 32 arcseconds search radius with full bootstrap resamples returned.



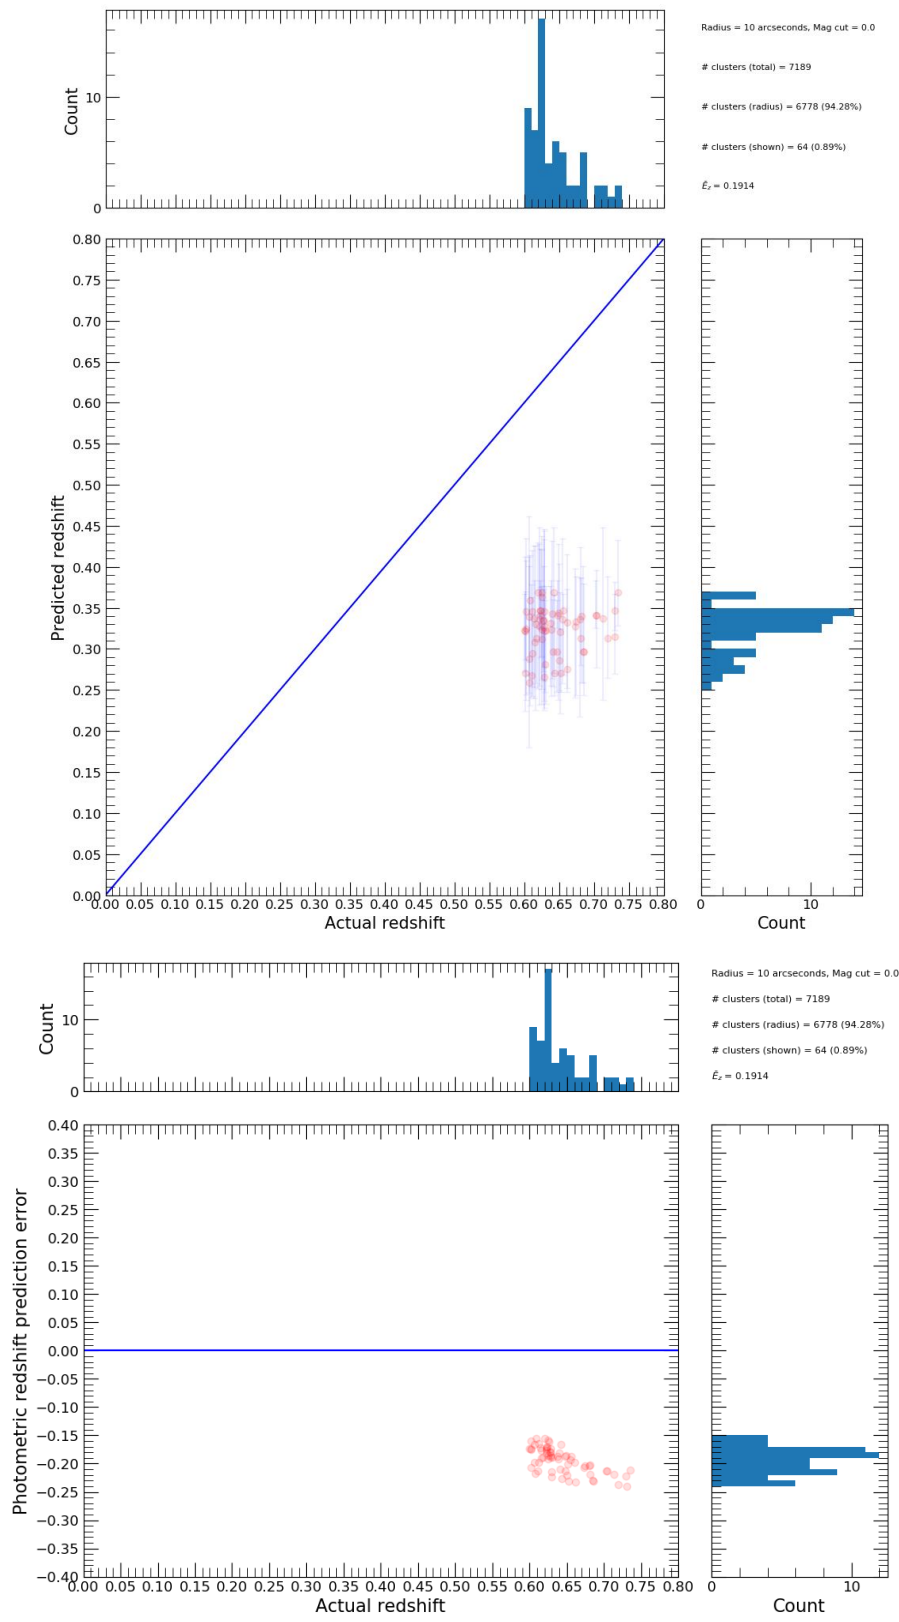

**Figure S27.** Plots displaying the performance of photometric redshift predictions of clusters at high redshift with low richness, which did not qualify for the WNMR dataset, that had partial bootstrap resamples returned within a 10 arcseconds search radius. Top row: Predicted versus 'actual' photometric redshift of tested clusters with frequency histograms of the distributions. Bottom row: Non-absolute photometric redshift prediction error versus 'actual' redshift of tested clusters with frequency histograms of the distributions. Other: '# clusters (total)' represents the total number of clusters at high redshift with low richness which did not qualify for the WNMR dataset, '# clusters (radius)' represents the number of clusters at high redshift with low richness which did not qualify for the WNMR dataset that have observed galaxies within a 10 arcseconds search radius, '# clusters (shown)' represents the number of clusters at high redshift with low richness which did not qualify for the WNMR dataset that have observed galaxies within a 10 arcseconds search radius with partial bootstrap resamples returned,  $\bar{E}_z$  represents the median of photometric redshift prediction errors across all tested clusters within a 10 arcseconds search radius with partial bootstrap resamples returned.

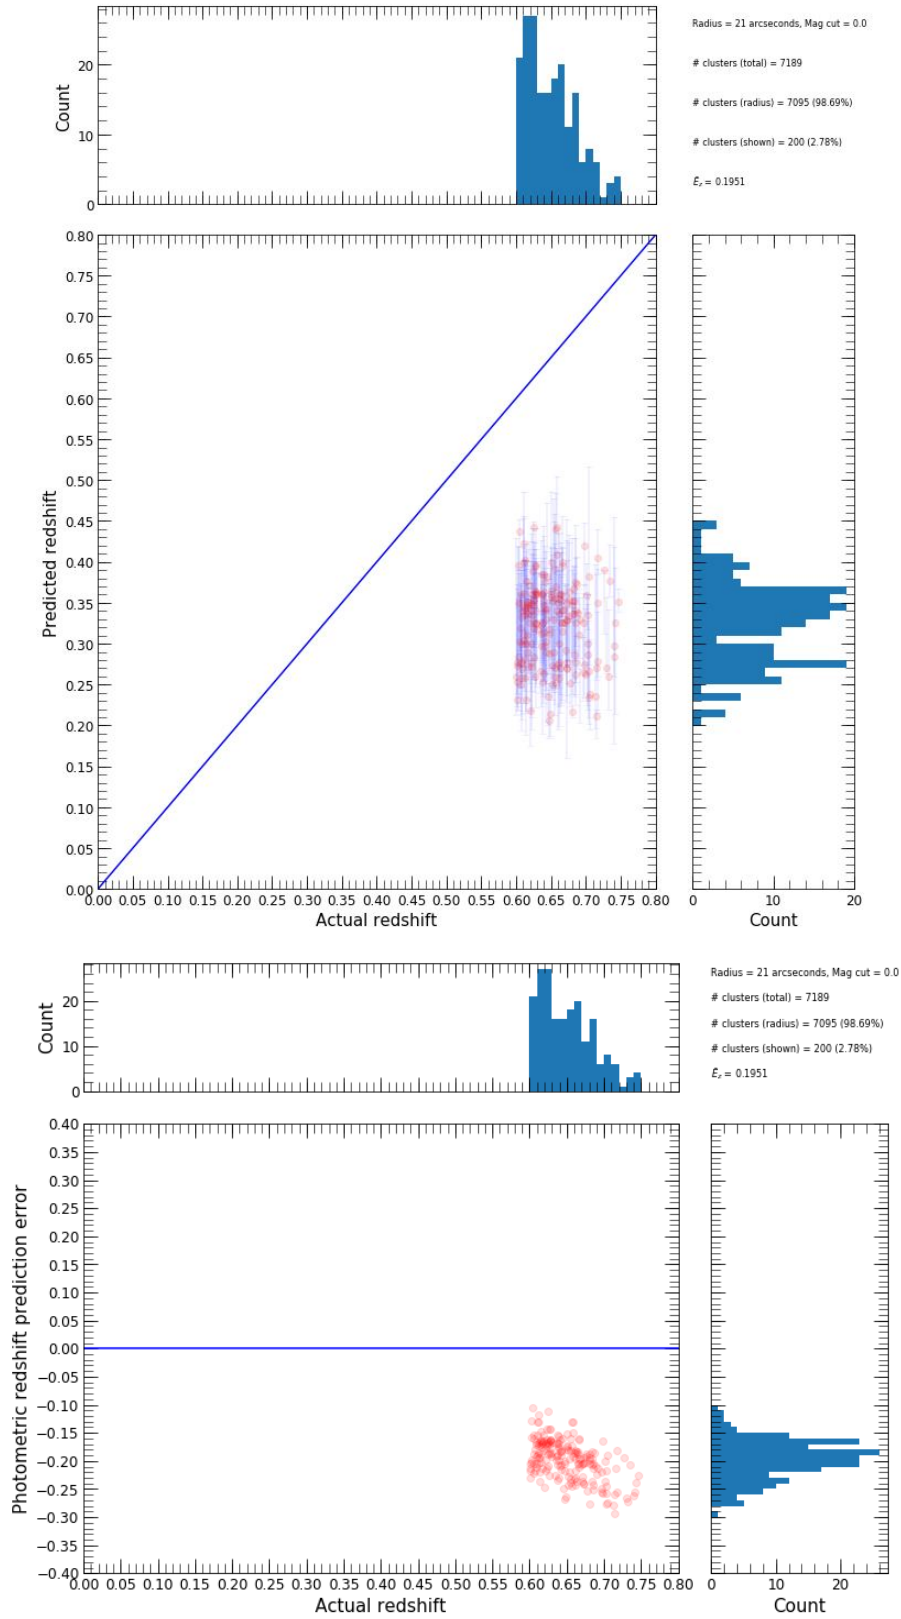

**Figure S28.** Plots displaying the performance of photometric redshift predictions of clusters at high redshift with low richness, which did not qualify for the WNMR dataset, that had partial bootstrap resamples returned within a 21 arcseconds search radius. Top row: Predicted versus 'actual' photometric redshift of tested clusters with frequency histograms of the distributions. Bottom row: Non-absolute photometric redshift prediction error versus 'actual' redshift of tested clusters with frequency histograms of the distributions. Other: '# clusters (total)' represents the total number of clusters at high redshift with low richness which did not qualify for the WNMR dataset, '# clusters (radius)' represents the number of clusters at high redshift with low richness which did not qualify for the WNMR dataset that have observed galaxies within a 21 arcseconds search radius, '# clusters (shown)' represents the number of clusters at high redshift with low richness which did not qualify for the WNMR dataset that have observed galaxies within a 21 arcseconds search radius with partial bootstrap resamples returned,  $\tilde{E}_z$  represents the median of photometric redshift prediction errors across all tested clusters within a 21 arcseconds search radius with partial bootstrap resamples returned.



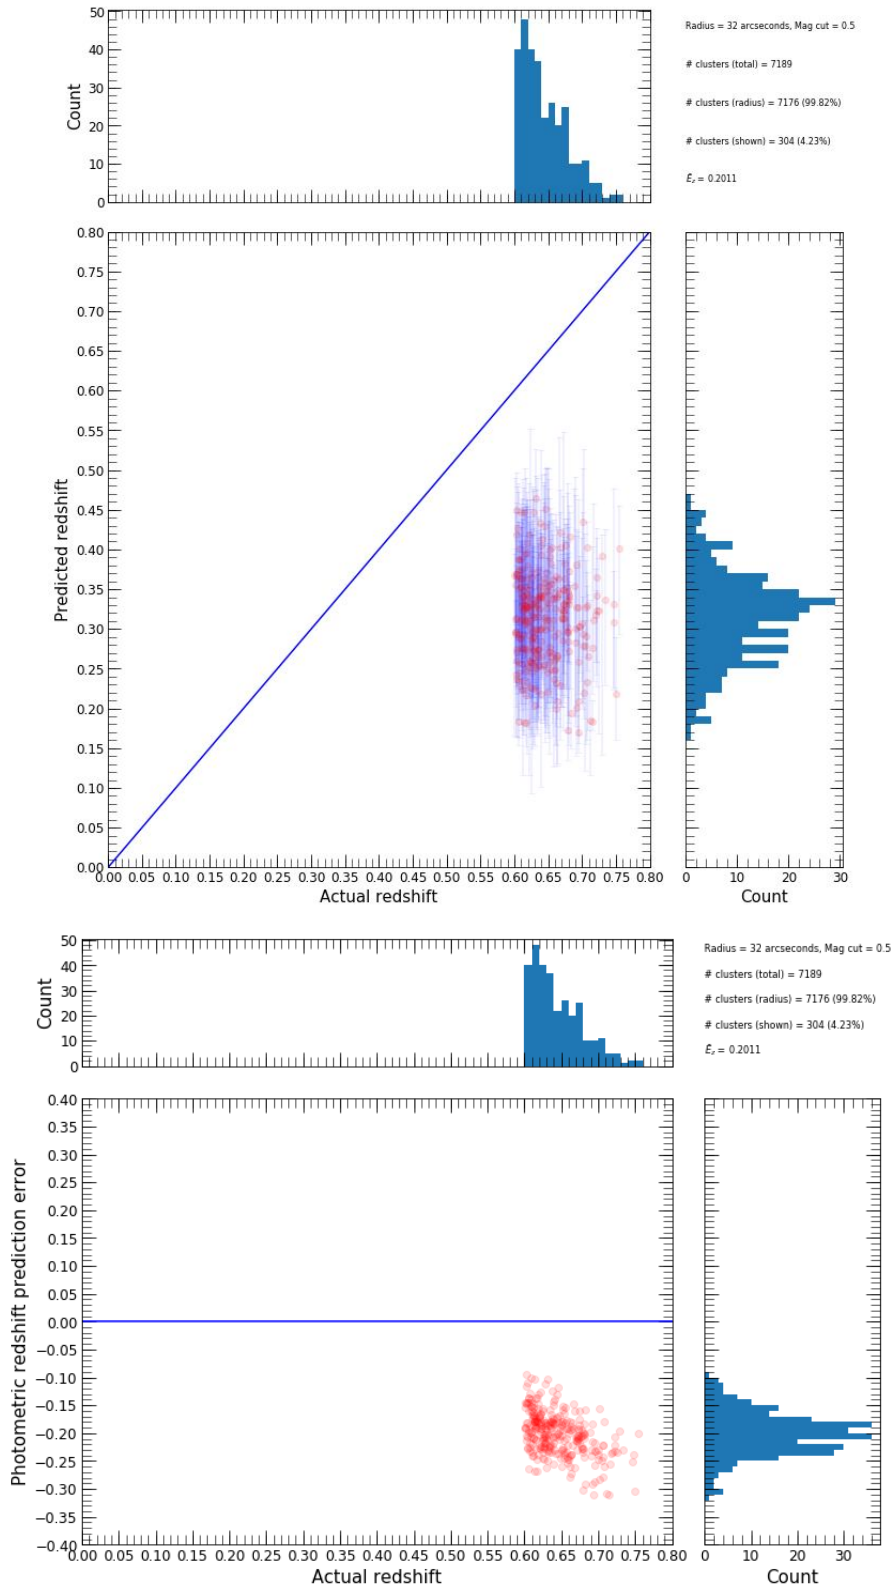

**Figure S29.** Plots displaying the performance of photometric redshift predictions of clusters at high redshift with low richness, which did not qualify for the WNMR dataset, that had partial bootstrap resamples returned within a 32 arcseconds search radius. Top row: Predicted versus 'actual' photometric redshift of tested clusters with frequency histograms of the distributions. Bottom row: Non-absolute photometric redshift prediction error versus 'actual' redshift of tested clusters with frequency histograms of the distributions. Other: '# clusters (total)' represents the total number of clusters at high redshift with low richness which did not qualify for the WNMR dataset, '# clusters (radius)' represents the number of clusters at high redshift with low richness which did not qualify for the WNMR dataset that have observed galaxies within a 32 arcseconds search radius, '# clusters (shown)' represents the number of clusters at high redshift with low richness which did not qualify for the WNMR dataset that have observed galaxies within a 32 arcseconds search radius with partial bootstrap resamples returned,  $\bar{E}_z$  represents the median of photometric redshift prediction errors across all tested clusters within a 32 arcseconds search radius with partial bootstrap resamples returned.

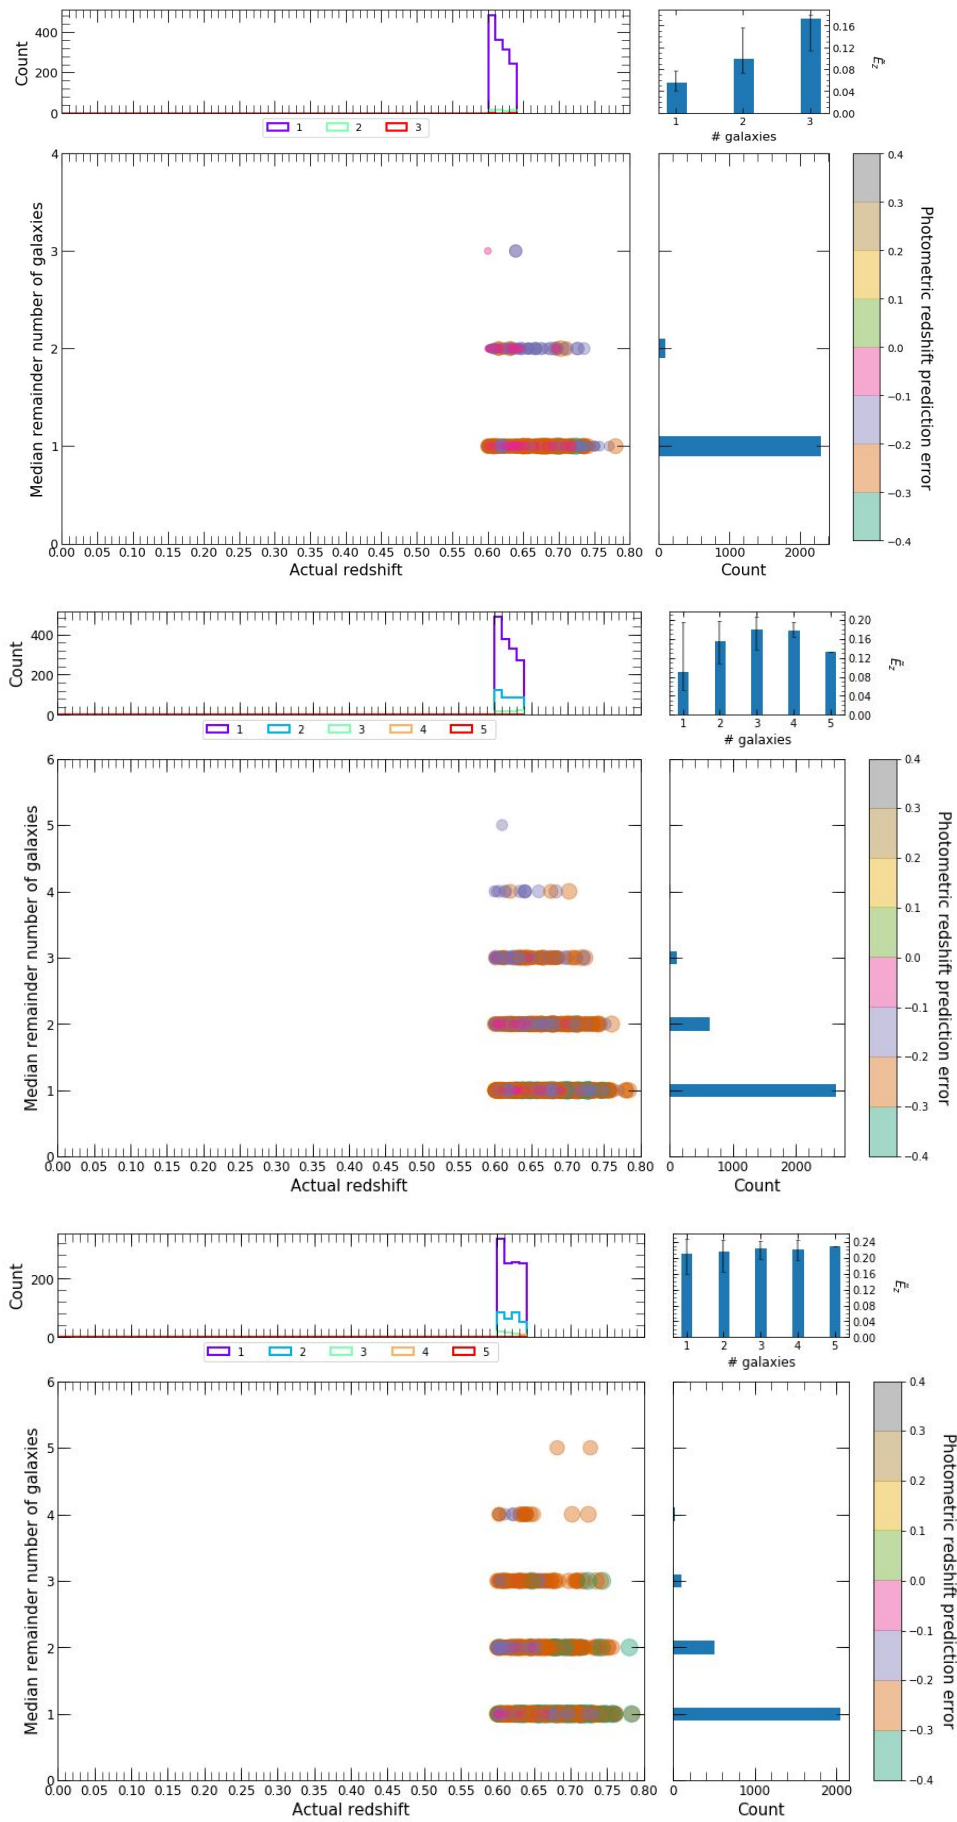

**Figure S30.** Plots displaying the number of galaxies used in photometric redshift predictions of clusters at high redshift with low richness versus ‘actual’ redshift of tested clusters, which did not qualify for the WNMR dataset, where predictions had full bootstrap resamples returned within a 10 (top row), 21 (middle row) and 32 (bottom row) arcseconds search radius. It should be noted that the size of individual points change in relation to the value of the non-absolute photometric redshift prediction error. Frequency histograms of the distributions are also shown.  $\bar{E}_z$  represents the median of photometric redshift prediction errors across all tested clusters for each number of galaxies bin.

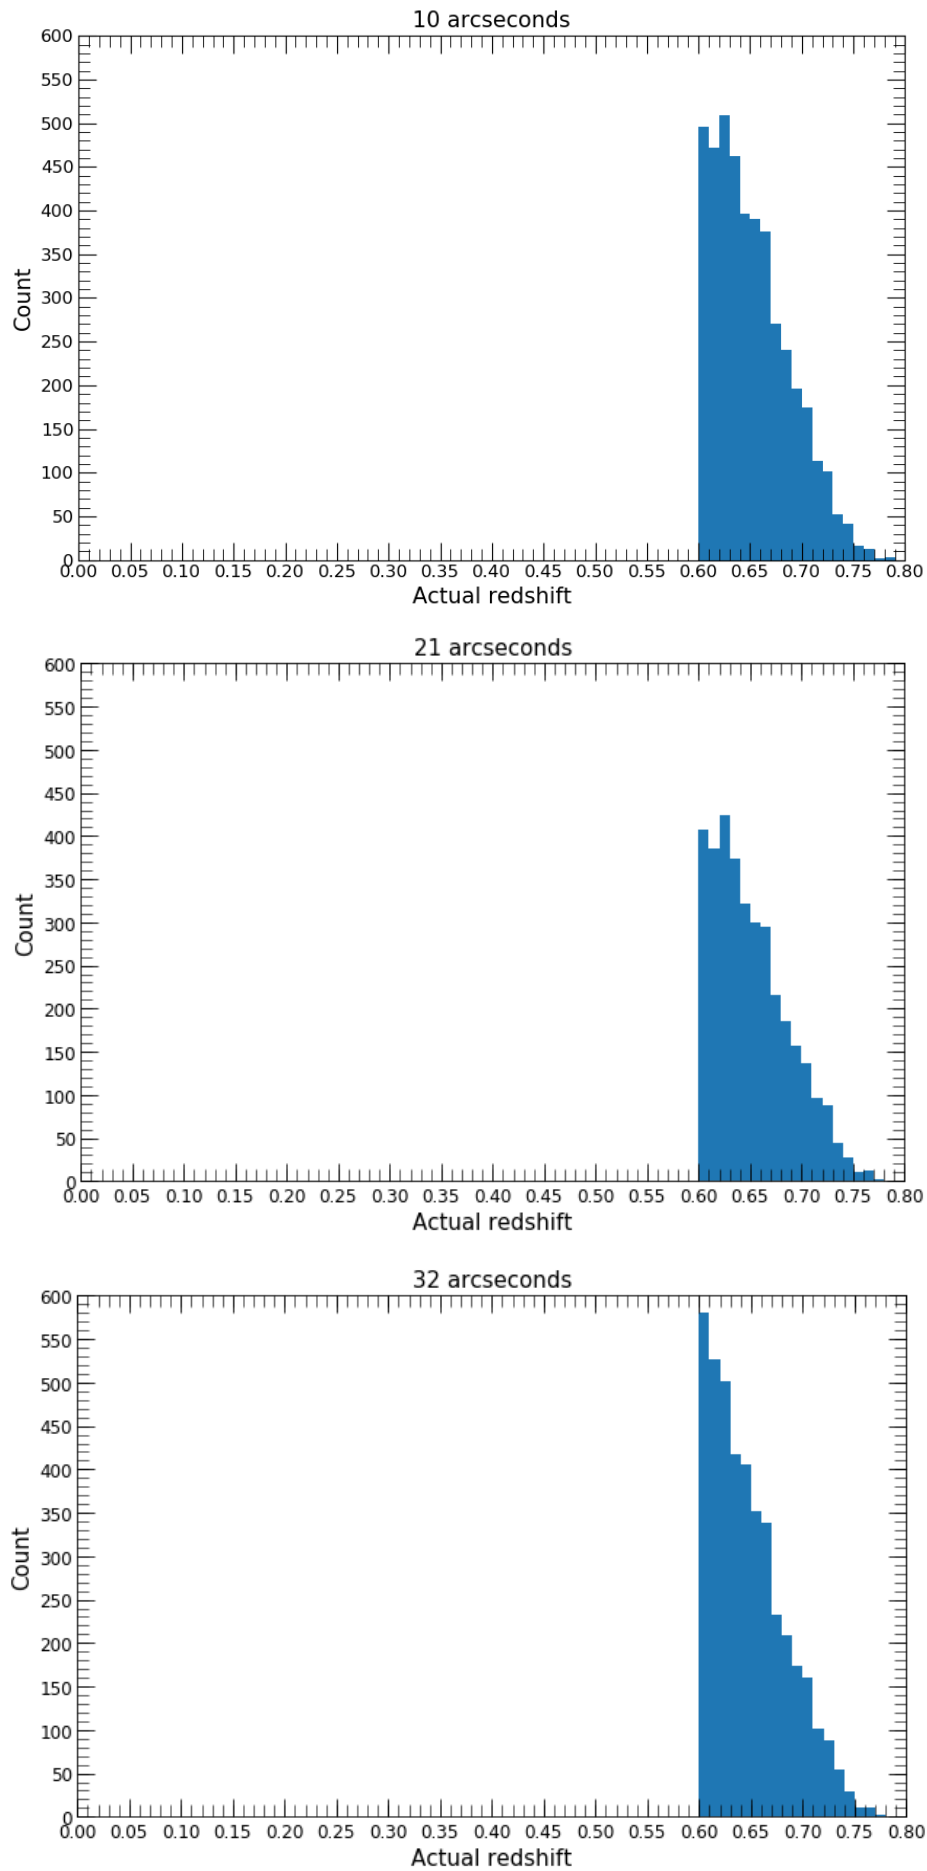

**Figure S31.** Frequency histograms displaying the 'actual' redshift distributions of clusters at high redshift with low richness, which did not qualify for the WNMR dataset, that had no bootstrap resamples returned within a 10 (top row), 21 (middle row) and 32 (bottom row) arcseconds search radius.

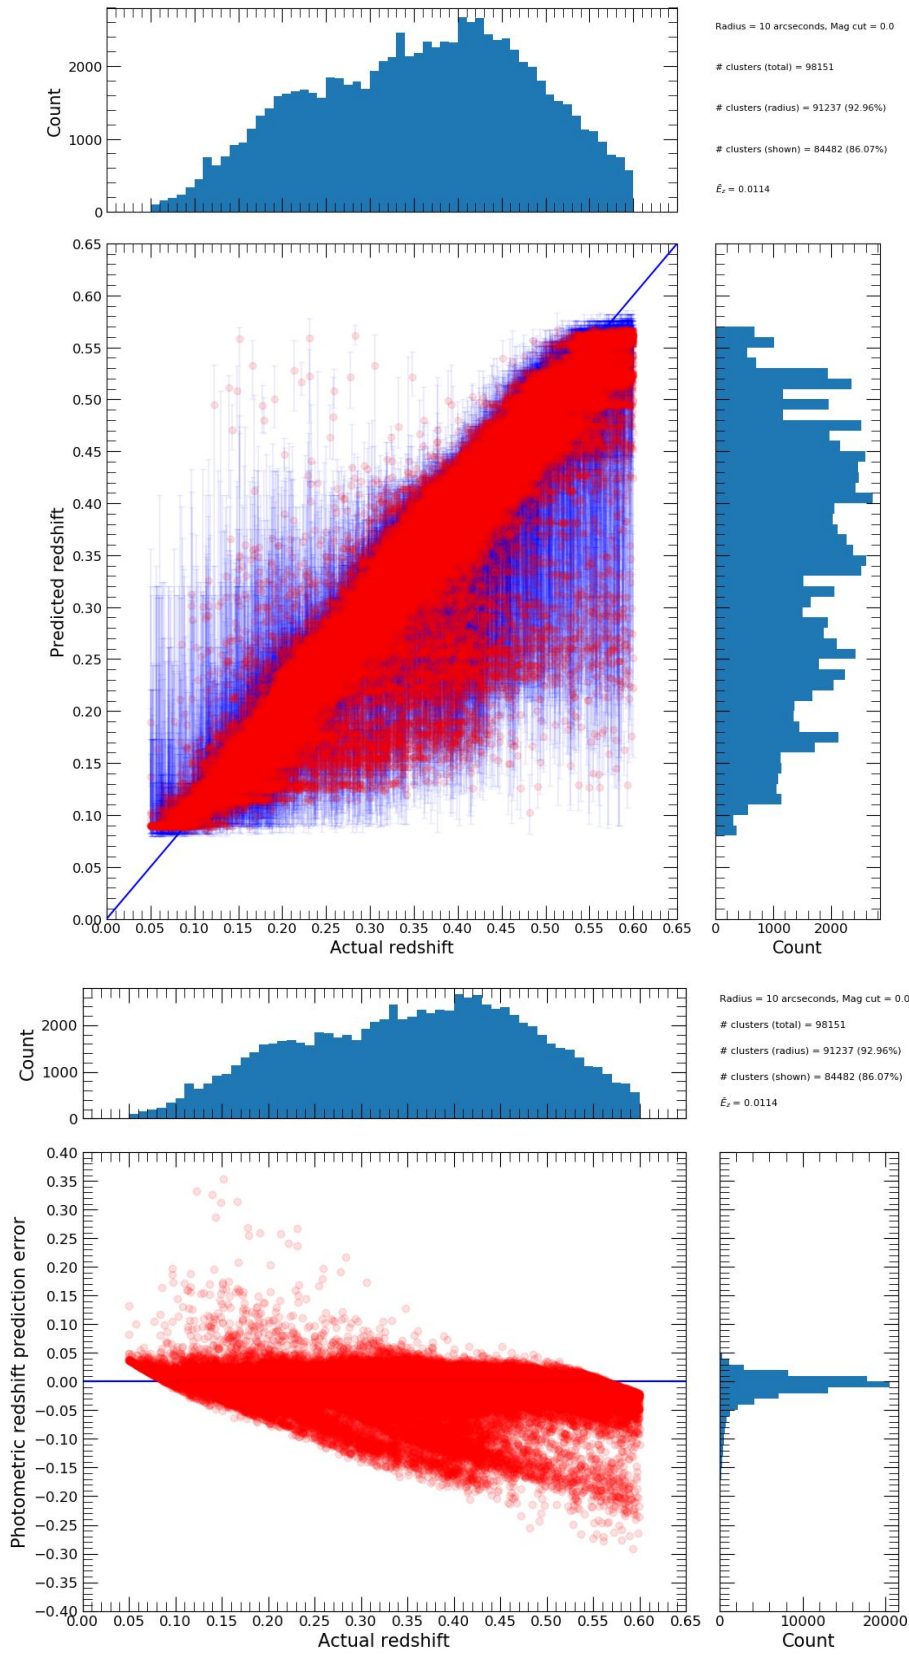

**Figure S32.** Plots displaying the performance of photometric redshift predictions of clusters with low richness, which did not qualify for the WNMR dataset, that had full bootstrap resamples returned within a 10 arcseconds search radius. Top row: Predicted versus 'actual' photometric redshift of tested clusters with frequency histograms of the distributions. Bottom row: Non-absolute photometric redshift prediction error versus 'actual' redshift of tested clusters with frequency histograms of the distributions. Other: '# clusters (total)' represents the total number of clusters with low richness which did not qualify for the WNMR dataset, '# clusters (radius)' represents the number of clusters with low richness which did not qualify for the WNMR dataset that have observed galaxies within a 10 arcseconds search radius, '# clusters (shown)' represents the number of clusters with low richness which did not qualify for the WNMR dataset that have observed galaxies within a 10 arcseconds search radius with full bootstrap resamples returned,  $\tilde{E}_z$  represents the median of photometric redshift prediction errors across all tested clusters within a 10 arcseconds search radius with full bootstrap resamples returned.

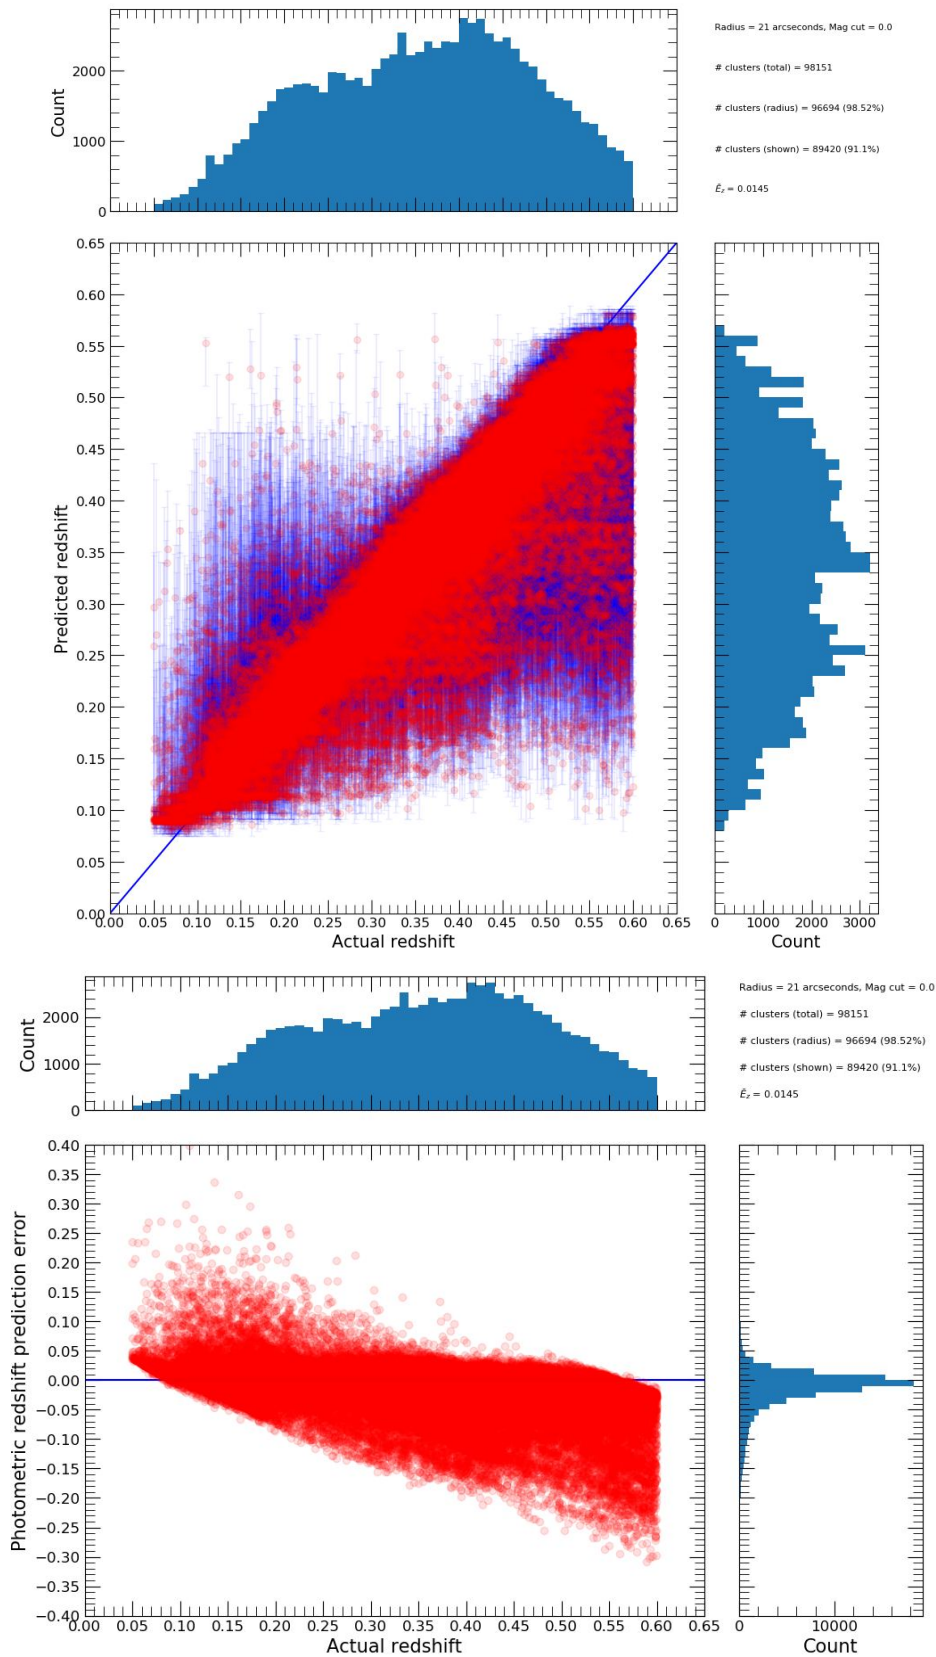

**Figure S33.** Plots displaying the performance of photometric redshift predictions of clusters with low richness, which did not qualify for the WNMR dataset, that had full bootstrap resamples returned within a 21 arcseconds search radius. Top row: Predicted versus 'actual' photometric redshift of tested clusters with frequency histograms of the distributions. Bottom row: Non-absolute photometric redshift prediction error versus 'actual' redshift of tested clusters with frequency histograms of the distributions. Other: '# clusters (total)' represents the total number of clusters with low richness which did not qualify for the WNMR dataset, '# clusters (radius)' represents the number of clusters with low richness which did not qualify for the WNMR dataset that have observed galaxies within a 21 arcseconds search radius, '# clusters (shown)' represents the number of clusters with low richness which did not qualify for the WNMR dataset that have observed galaxies within a 21 arcseconds search radius with full bootstrap resamples returned,  $\bar{E}_z$  represents the median of photometric redshift prediction errors across all tested clusters within a 21 arcseconds search radius with full bootstrap resamples returned.



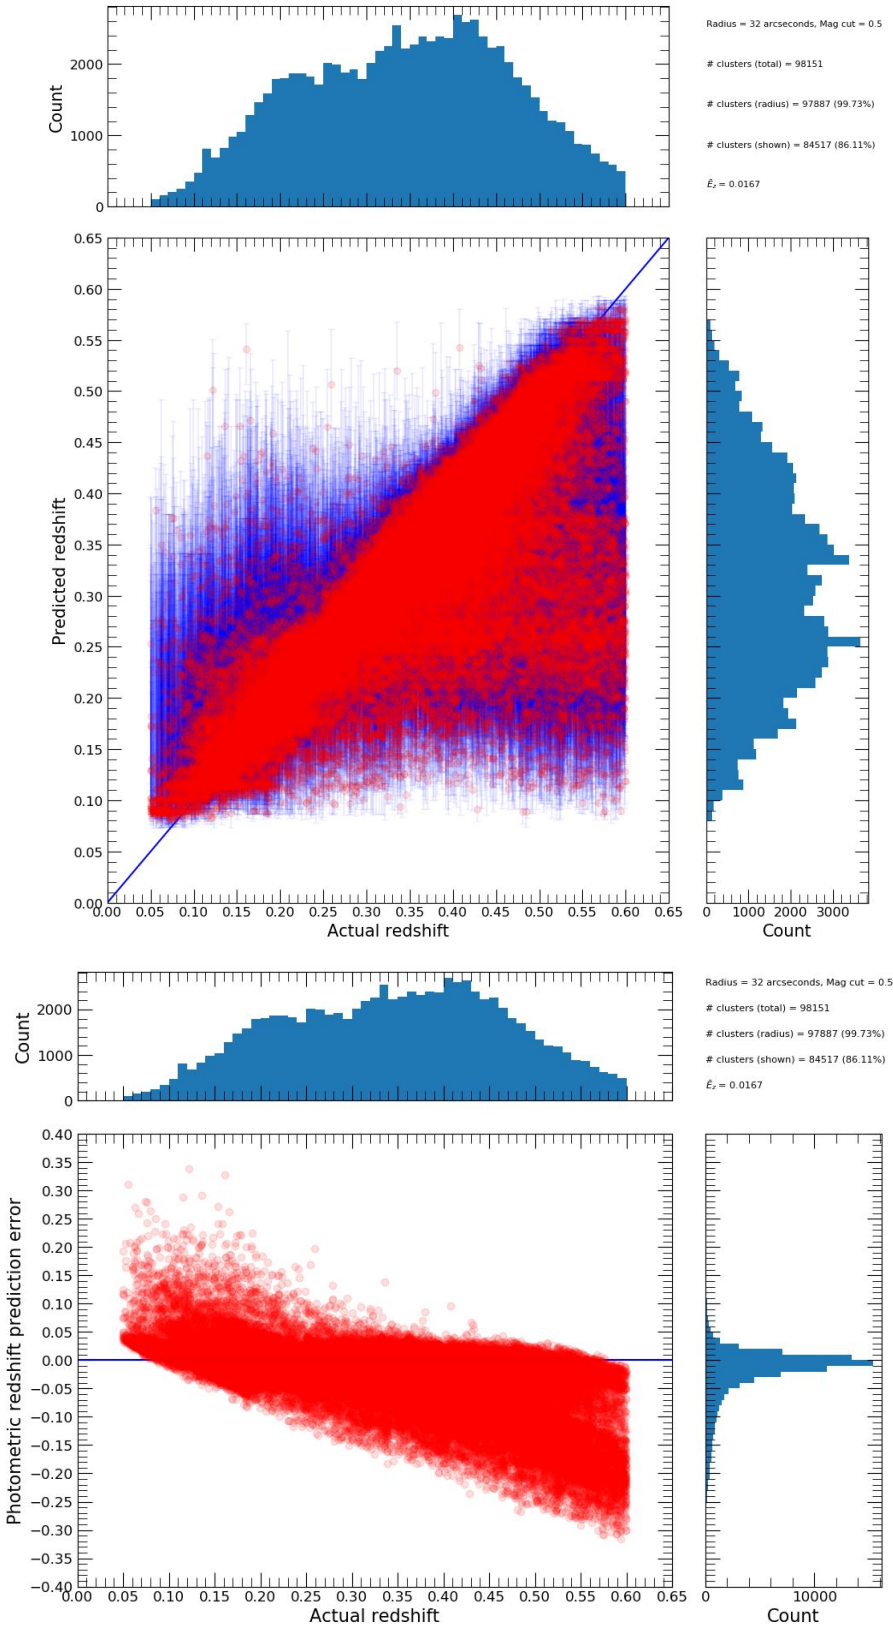

**Figure S34.** Plots displaying the performance of photometric redshift predictions of clusters with low richness, which did not qualify for the WNMR dataset, that had full bootstrap resamples returned within a 32 arcseconds search radius. Top row: Predicted versus 'actual' photometric redshift of tested clusters with frequency histograms of the distributions. Bottom row: Non-absolute photometric redshift prediction error versus 'actual' redshift of tested clusters with frequency histograms of the distributions. Other: '# clusters (total)' represents the total number of clusters with low richness which did not qualify for the WNMR dataset, '# clusters (radius)' represents the number of clusters with low richness which did not qualify for the WNMR dataset that have observed galaxies within a 32 arcseconds search radius, '# clusters (shown)' represents the number of clusters with low richness which did not qualify for the WNMR dataset that have observed galaxies within a 32 arcseconds search radius with full bootstrap resamples returned,  $\tilde{E}_z$  represents the median of photometric redshift prediction errors across all tested clusters within a 32 arcseconds search radius with full bootstrap resamples returned.

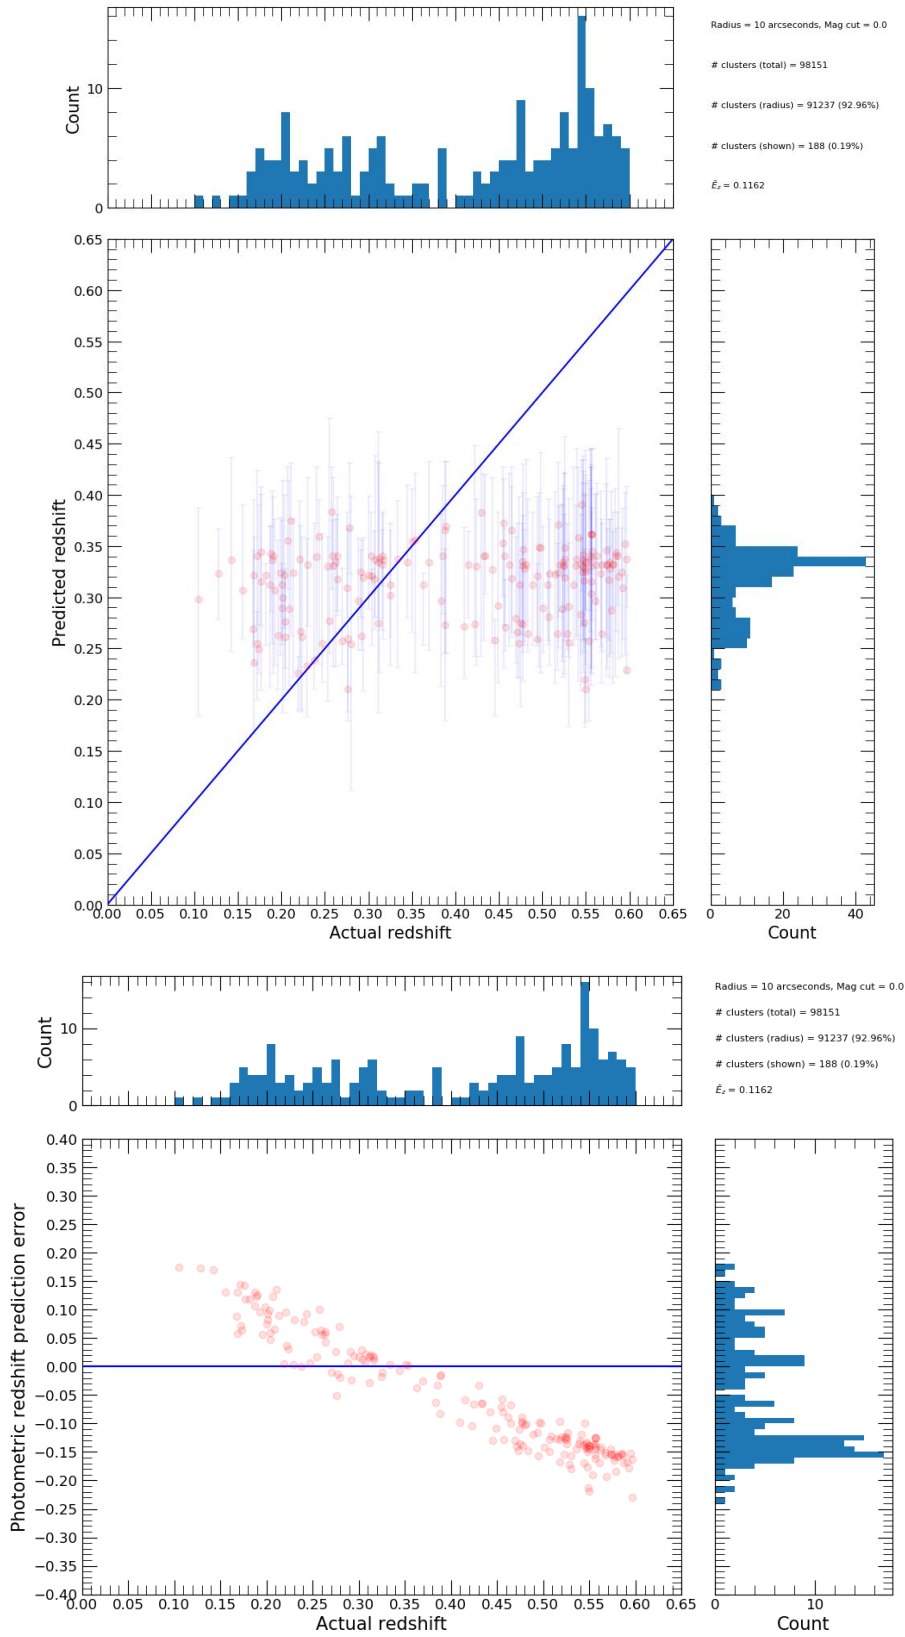

**Figure S35.** Plots displaying the performance of photometric redshift predictions of clusters with low richness, which did not qualify for the WNMN dataset, that had partial bootstrap resamples returned within a 10 arcseconds search radius. Top row: Predicted versus 'actual' photometric redshift of tested clusters with frequency histograms of the distributions. Bottom row: Non-absolute photometric redshift prediction error versus 'actual' redshift of tested clusters with frequency histograms of the distributions. Other: '# clusters (total)' represents the total number of clusters with low richness which did not qualify for the WNMN dataset, '# clusters (radius)' represents the number of clusters with low richness which did not qualify for the WNMN dataset that have observed galaxies within a 10 arcseconds search radius, '# clusters (shown)' represents the number of clusters with low richness which did not qualify for the WNMN dataset that have observed galaxies within a 10 arcseconds search radius with partial bootstrap resamples returned,  $\bar{E}_z$  represents the median of photometric redshift prediction errors across all tested clusters within a 10 arcseconds search radius with partial bootstrap resamples returned.

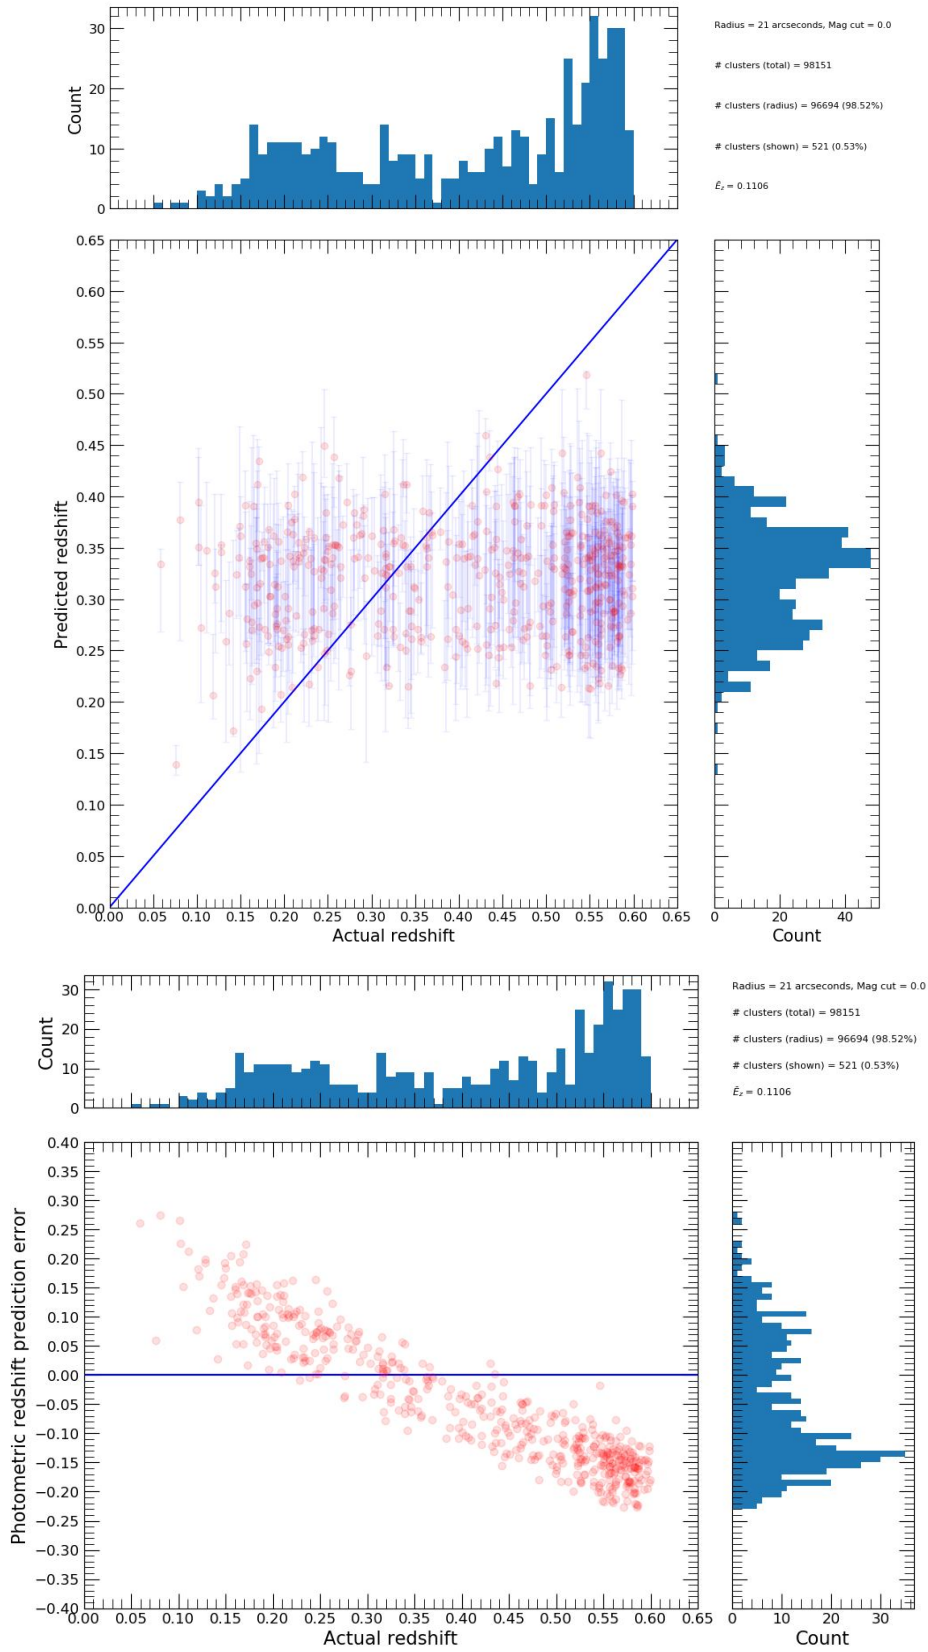

**Figure S36.** Plots displaying the performance of photometric redshift predictions of clusters with low richness, which did not qualify for the WNMR dataset, that had partial bootstrap resamples returned within a 21 arcseconds search radius. Top row: Predicted versus 'actual' photometric redshift of tested clusters with frequency histograms of the distributions. Bottom row: Non-absolute photometric redshift prediction error versus 'actual' redshift of tested clusters with frequency histograms of the distributions. Other: '# clusters (total)' represents the total number of clusters with low richness which did not qualify for the WNMR dataset, '# clusters (radius)' represents the number of clusters with low richness which did not qualify for the WNMR dataset that have observed galaxies within a 21 arcseconds search radius, '# clusters (shown)' represents the number of clusters with low richness which did not qualify for the WNMR dataset that have observed galaxies within a 21 arcseconds search radius with partial bootstrap resamples returned,  $\bar{E}_z$  represents the median of photometric redshift prediction errors across all tested clusters within a 21 arcseconds search radius with partial bootstrap resamples returned.





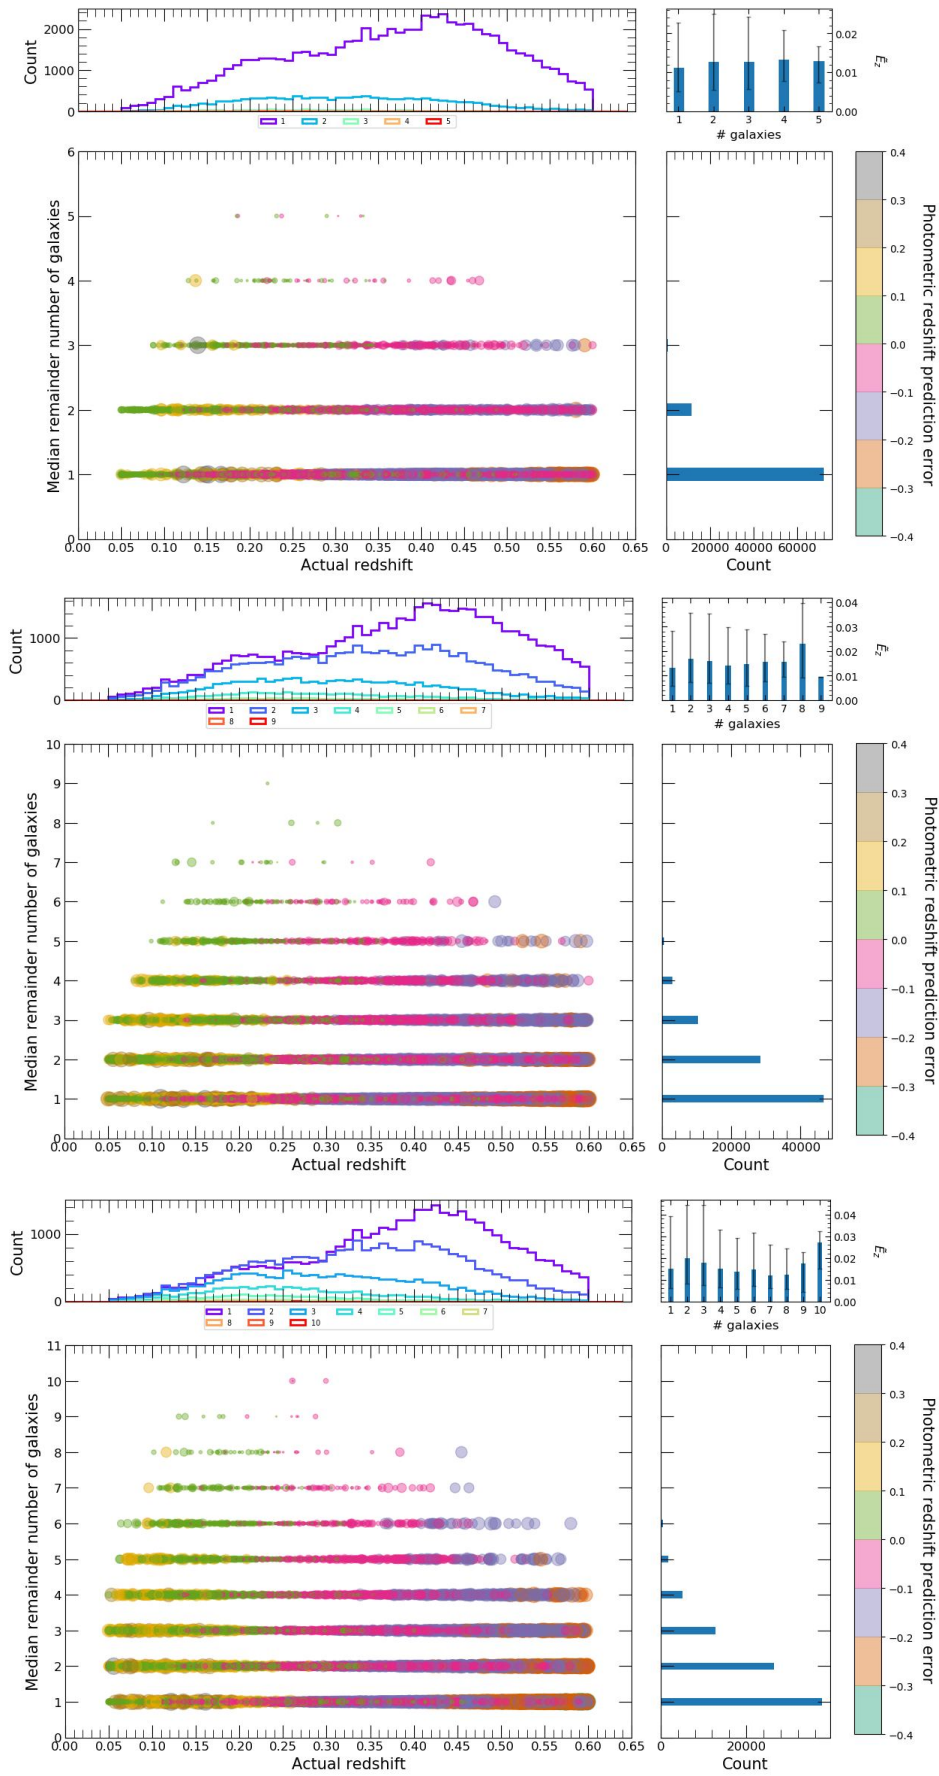

**Figure S38.** Plots displaying the number of galaxies used in photometric redshift predictions of clusters with low richness versus ‘actual’ redshift of tested clusters, which did not qualify for the WNMR dataset, where predictions had full bootstrap resamples returned within a 10 (top row), 21 (middle row) and 32 (bottom row) arcseconds search radius. It should be noted that the size of individual points change in relation to the value of the non-absolute photometric redshift prediction error. Frequency histograms of the distributions are also shown.  $\bar{E}_z$  represents the median of photometric redshift prediction errors across all tested clusters for each number of galaxies bin.

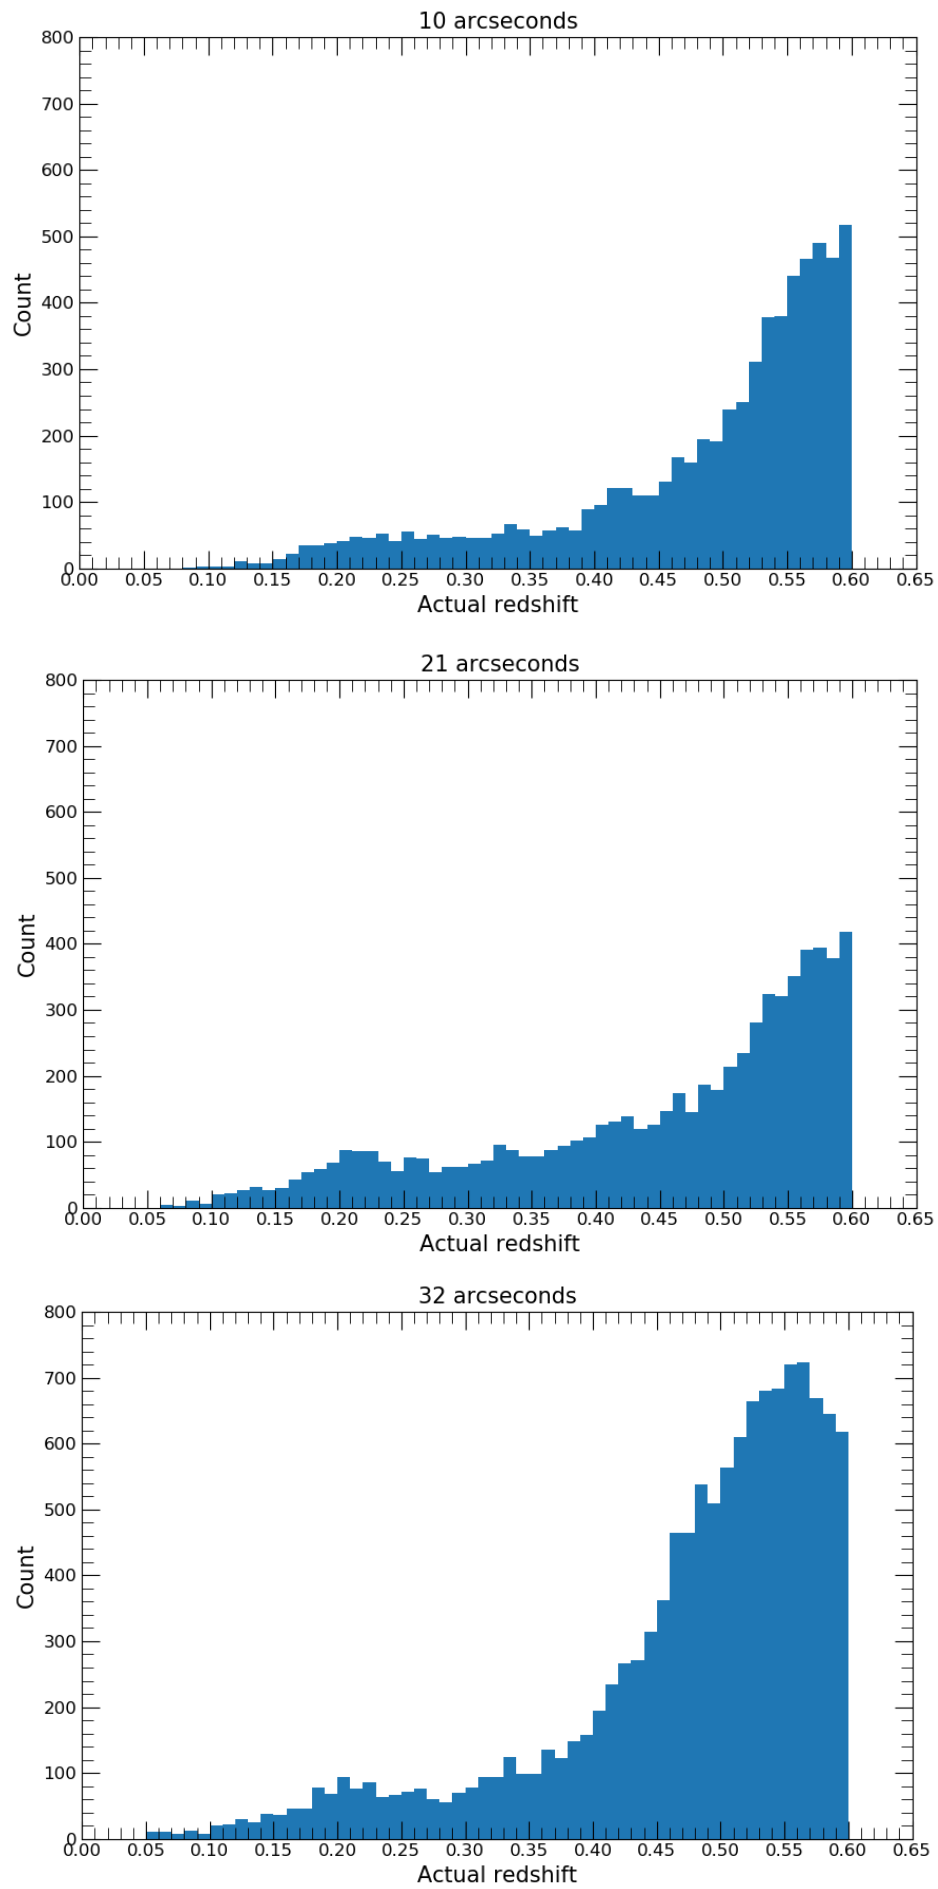

**Figure S39.** Frequency histograms displaying the ‘actual’ redshift distributions of clusters with low richness, which did not qualify for the WNMR dataset, that had no bootstrap resamples returned within a 10 (top row), 21 (middle row) and 32 (bottom row) arcseconds search radius.

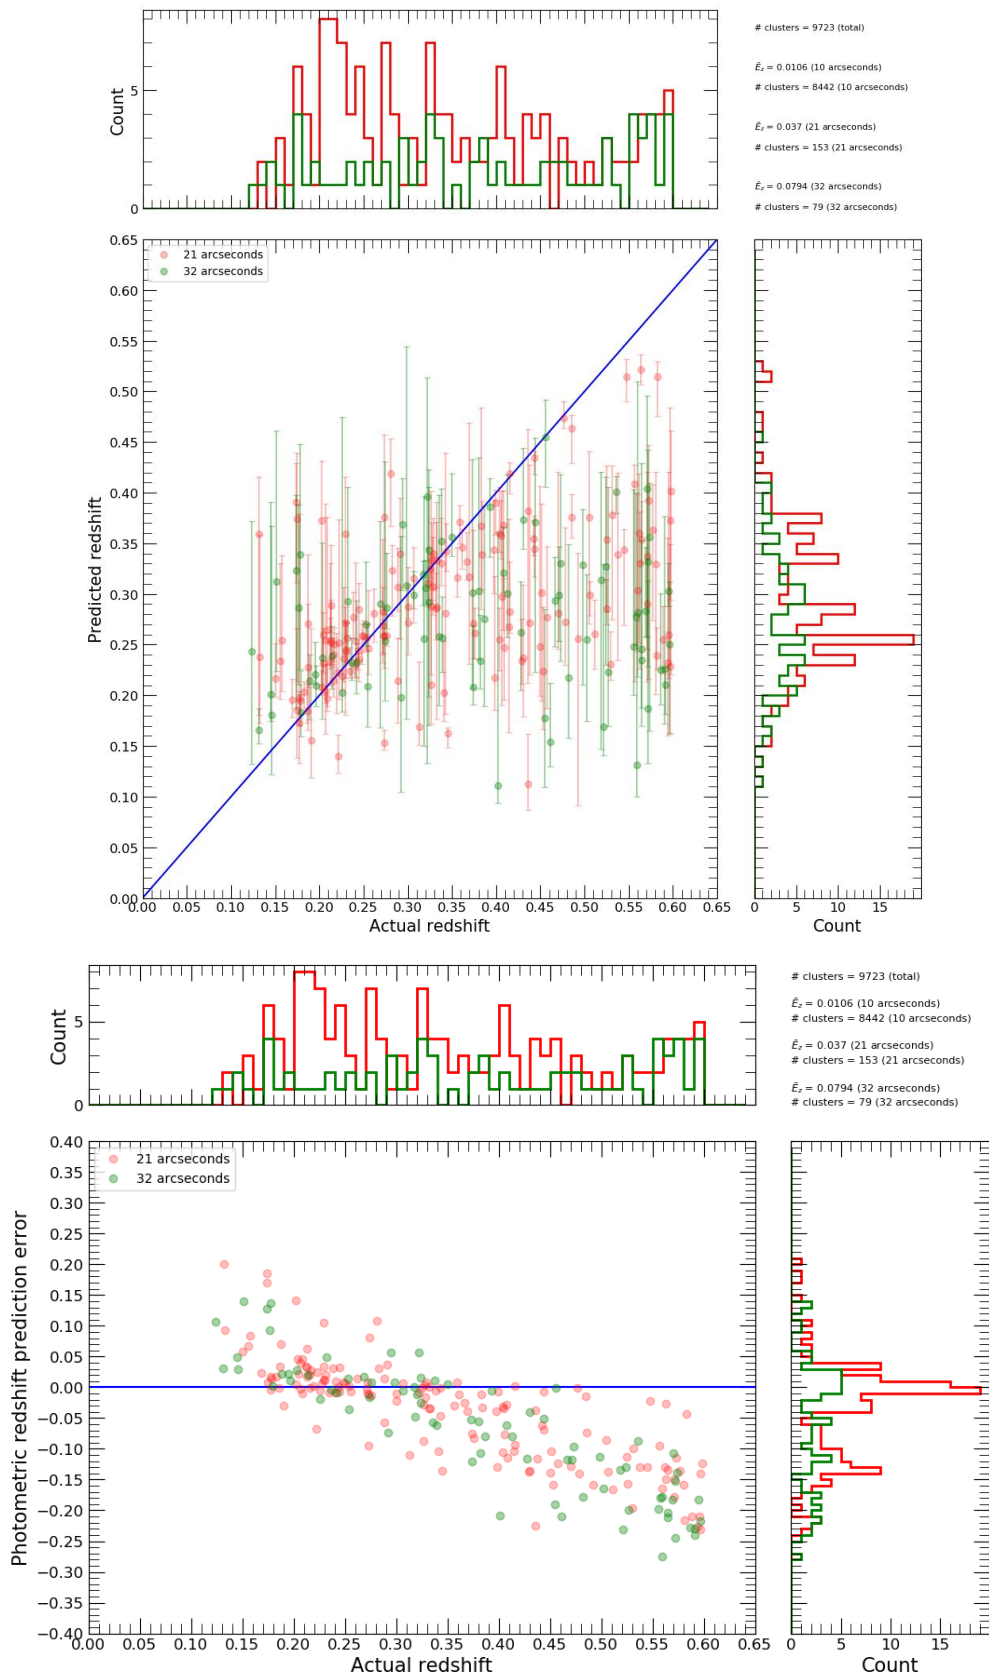

**Figure S40.** Plots displaying the performance of photometric redshift predictions of clusters for the WNMR test set that had full bootstrap resamples returned within a 21 (red) or 32 (green) arcseconds search radius. If a cluster has no or partial bootstrap resamples returned at 10 arcseconds then the search radius is increased until a prediction with full bootstrap resamples returned is obtained. Top row: Predicted versus 'actual' photometric redshift of tested clusters with frequency histograms of the distributions. Bottom row: Non-absolute photometric redshift prediction error versus 'actual' redshift of tested clusters with frequency histograms of the distributions. Other: '# clusters (total)' represents the total number of clusters for the WNMR test set, '# clusters' represents the number of clusters for the WNMR test set that have observed galaxies within a 10, 21 and 32 arcseconds search radii with full bootstrap resamples returned,  $\bar{E}_z$  represents the median of photometric redshift prediction errors across all tested clusters within a 10, 21 and 32 arcseconds search radii with full bootstrap resamples returned.

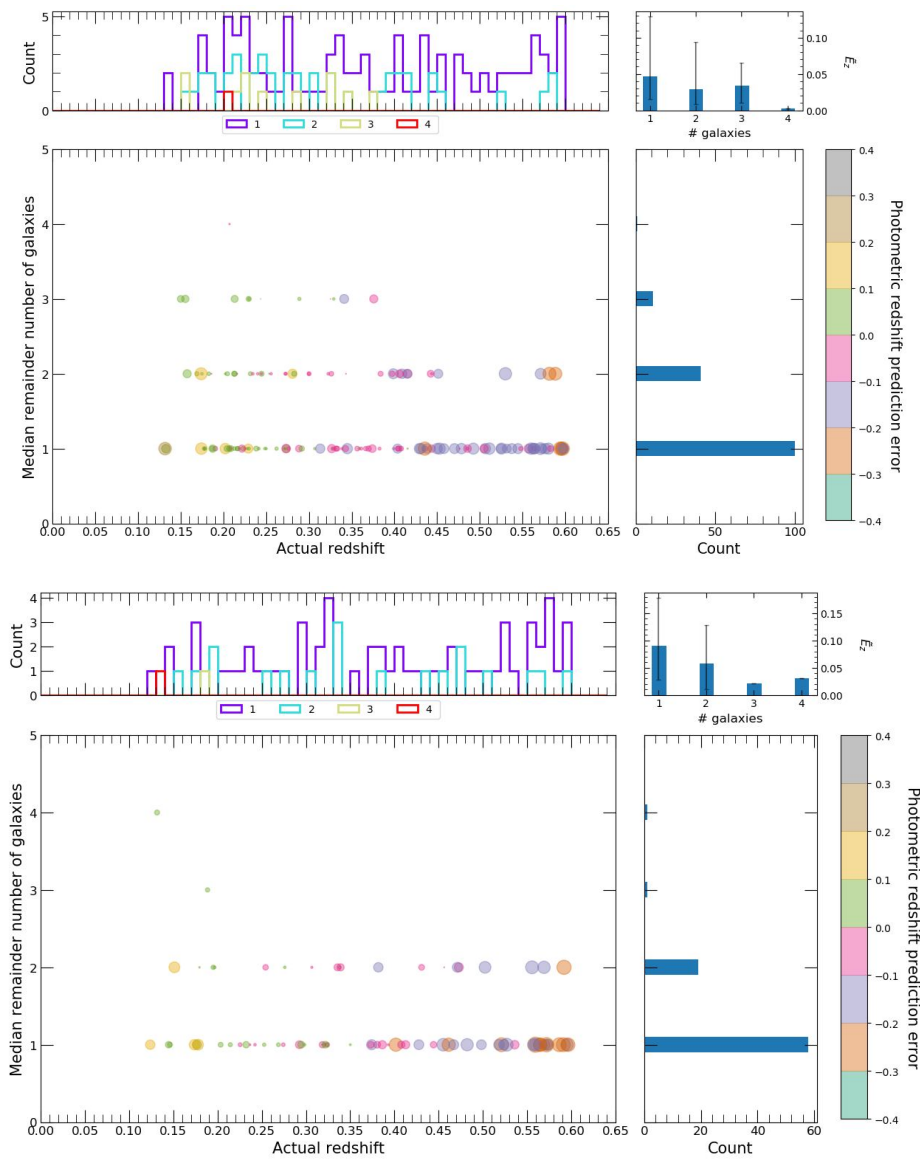

**Figure S41.** Plots displaying the number of galaxies used in photometric redshift predictions versus ‘actual’ redshift of tested clusters for the WNMR test set, where predictions had full bootstrap resamples returned within a 21 (top row) or 32 (bottom row) arcseconds search radius. If a cluster has no or partial bootstrap resamples returned at 10 arcseconds then the search radius is increased until a prediction with full bootstrap resamples returned is obtained. It should be noted that the size of individual points change in relation to the value of the non-absolute photometric redshift prediction error. Frequency histograms of the distributions are also shown.  $\bar{E}_z$  represents the median of photometric redshift prediction errors across all tested clusters for each number of galaxies bin.

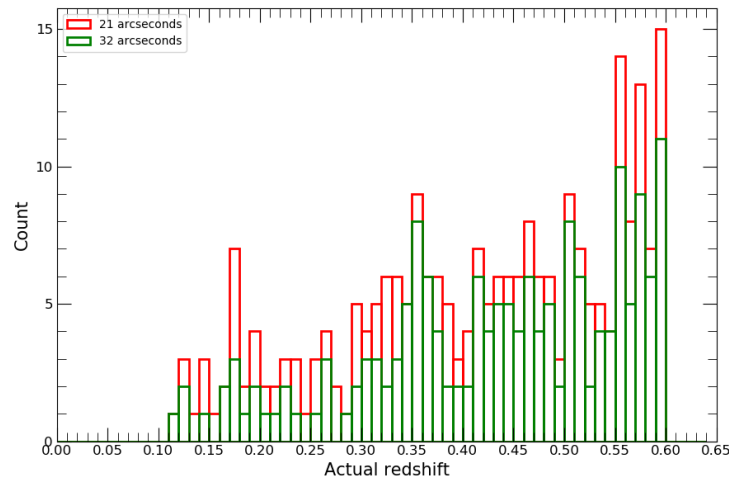

**Figure S42.** Frequency histograms displaying the ‘actual’ redshift distributions of the remaining clusters from the WNMR test set that had no bootstrap resamples returned within a 21 (red) or 32 (green) arcseconds search radius.



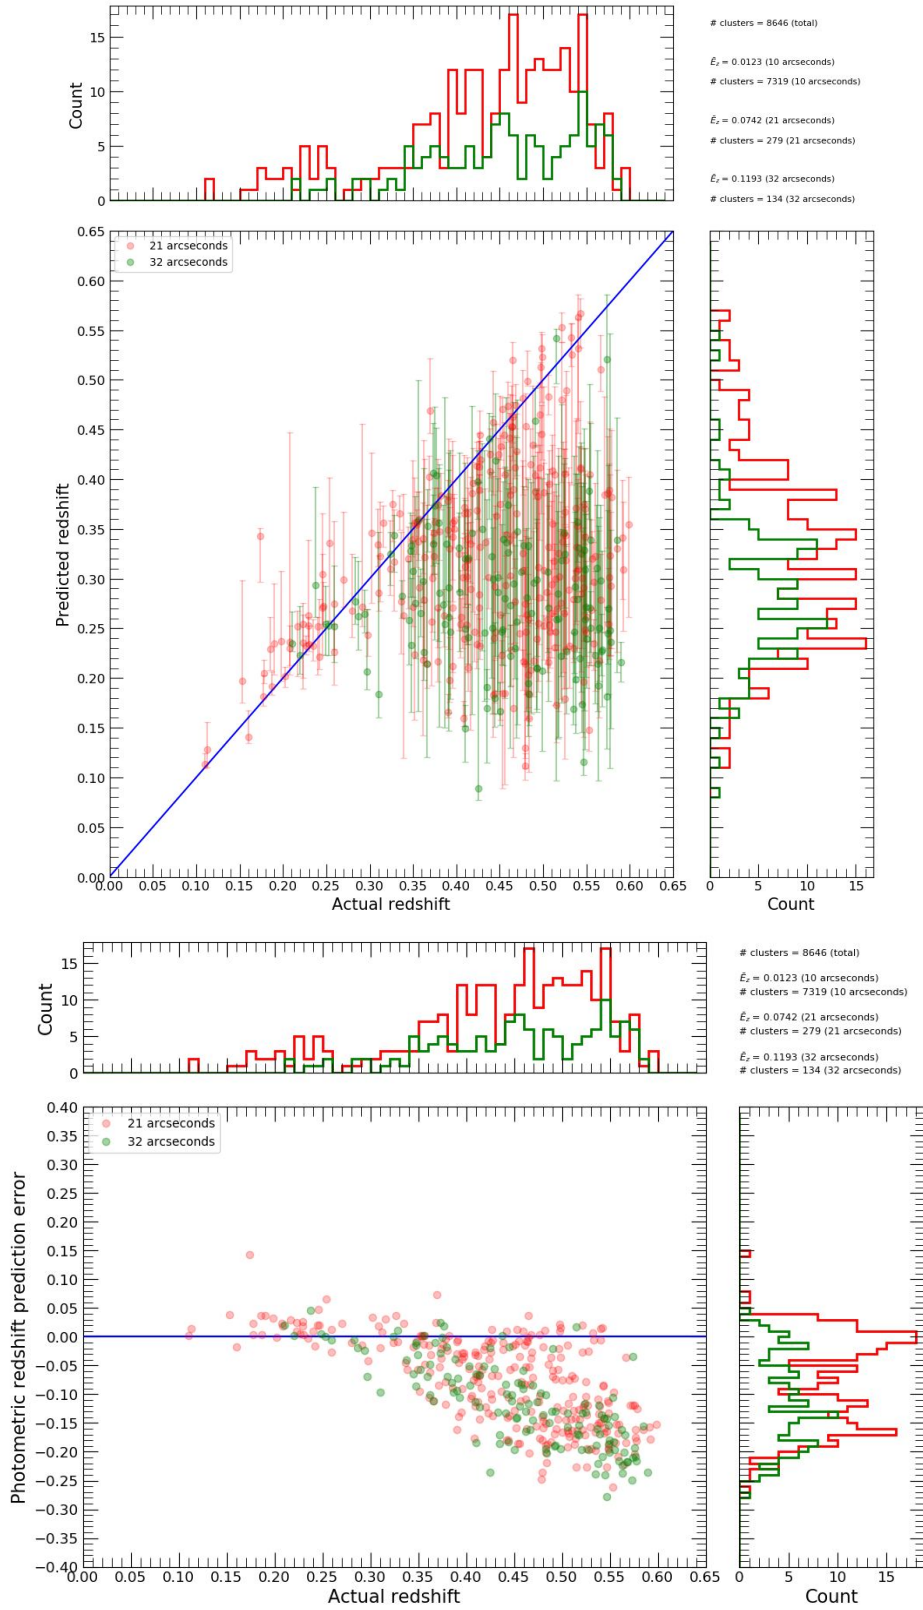

**Figure S43.** Plots displaying the performance of photometric redshift predictions of clusters for the RNMW test set that had full bootstrap resamples returned within a 21 (red) or 32 (green) arcseconds search radii. If a cluster has no or partial bootstrap resamples returned at 10 arcseconds then the search radius is increased until a prediction with full bootstrap resamples returned is obtained. Top row: Predicted versus 'actual' photometric redshift of tested clusters with frequency histograms of the distributions. Bottom row: Non-absolute photometric redshift prediction error versus 'actual' redshift of tested clusters with frequency histograms of the distributions. Other: '# clusters (total)' represents the total number of clusters for the RNMW test set, '# clusters' represents the number of clusters for the RNMW test set that have observed galaxies within a 10, 21 and 32 arcseconds search radii with full bootstrap resamples returned,  $\bar{E}_z$  represents the median of photometric redshift prediction errors across all tested clusters within a 10, 21 and 32 arcseconds search radii with full bootstrap resamples returned.



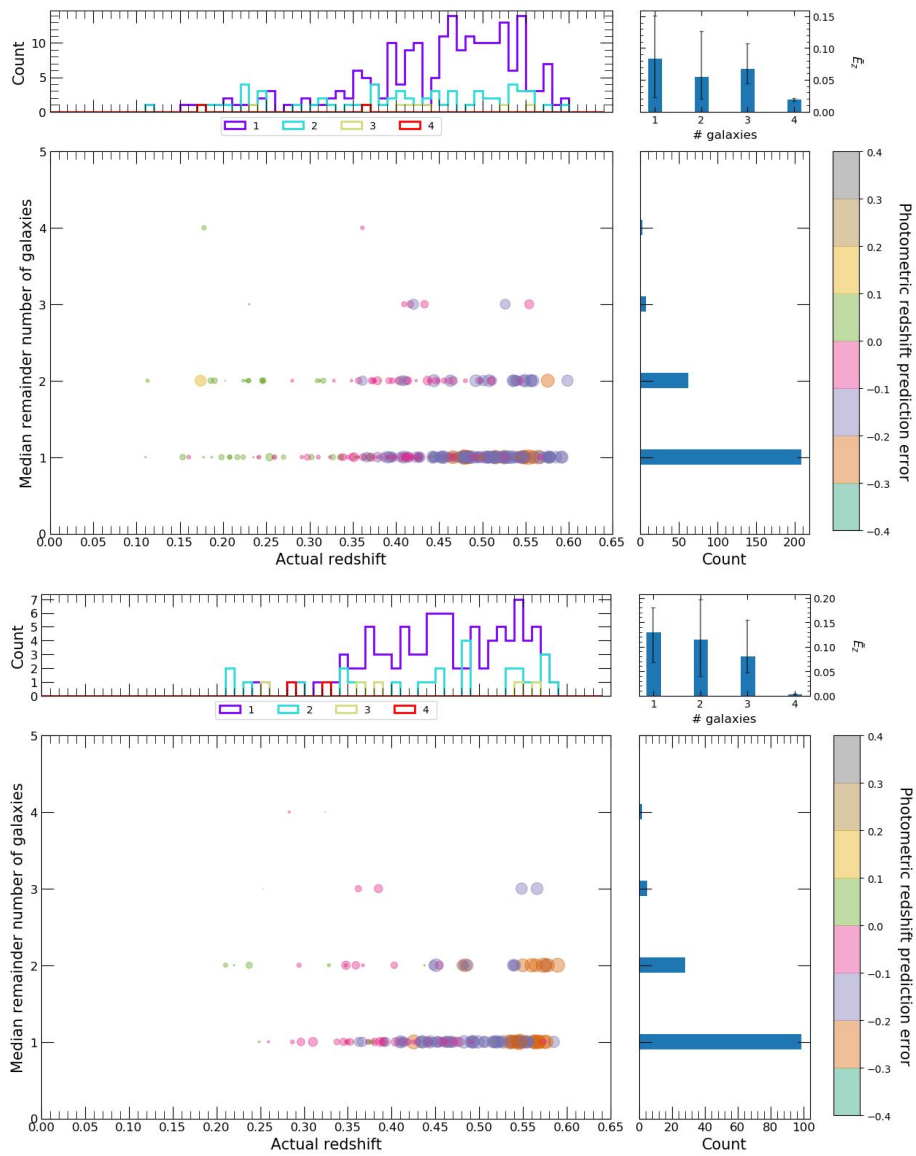

**Figure S44.** Plots displaying the number of galaxies used in photometric redshift predictions versus ‘actual’ redshift of tested clusters for the RNMW test set, where predictions had full bootstrap resamples returned within a 21 (top row) or 32 (bottom row) arcseconds search radius. If a cluster has no or partial bootstrap resamples returned at 10 arcseconds then the search radius is increased until a prediction with full bootstrap resamples returned is obtained. It should be noted that the size of individual points change in relation to the value of the non-absolute photometric redshift prediction error. Frequency histograms of the distributions are also shown.  $\bar{E}_z$  represents the median of photometric redshift prediction errors across all tested clusters for each number of galaxies bin.

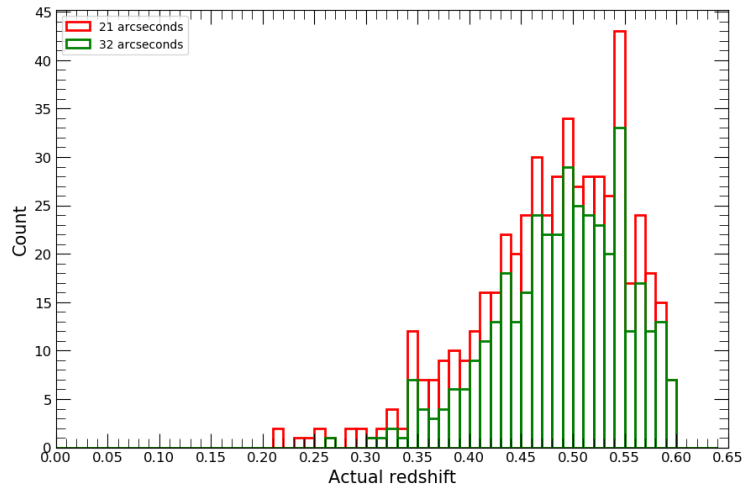

**Figure S45.** Frequency histograms displaying the ‘actual’ redshift distributions of the remaining clusters from the RNMW test set that had no bootstrap resamples returned within a 21 (red) or 32 (green) arcseconds search radius.

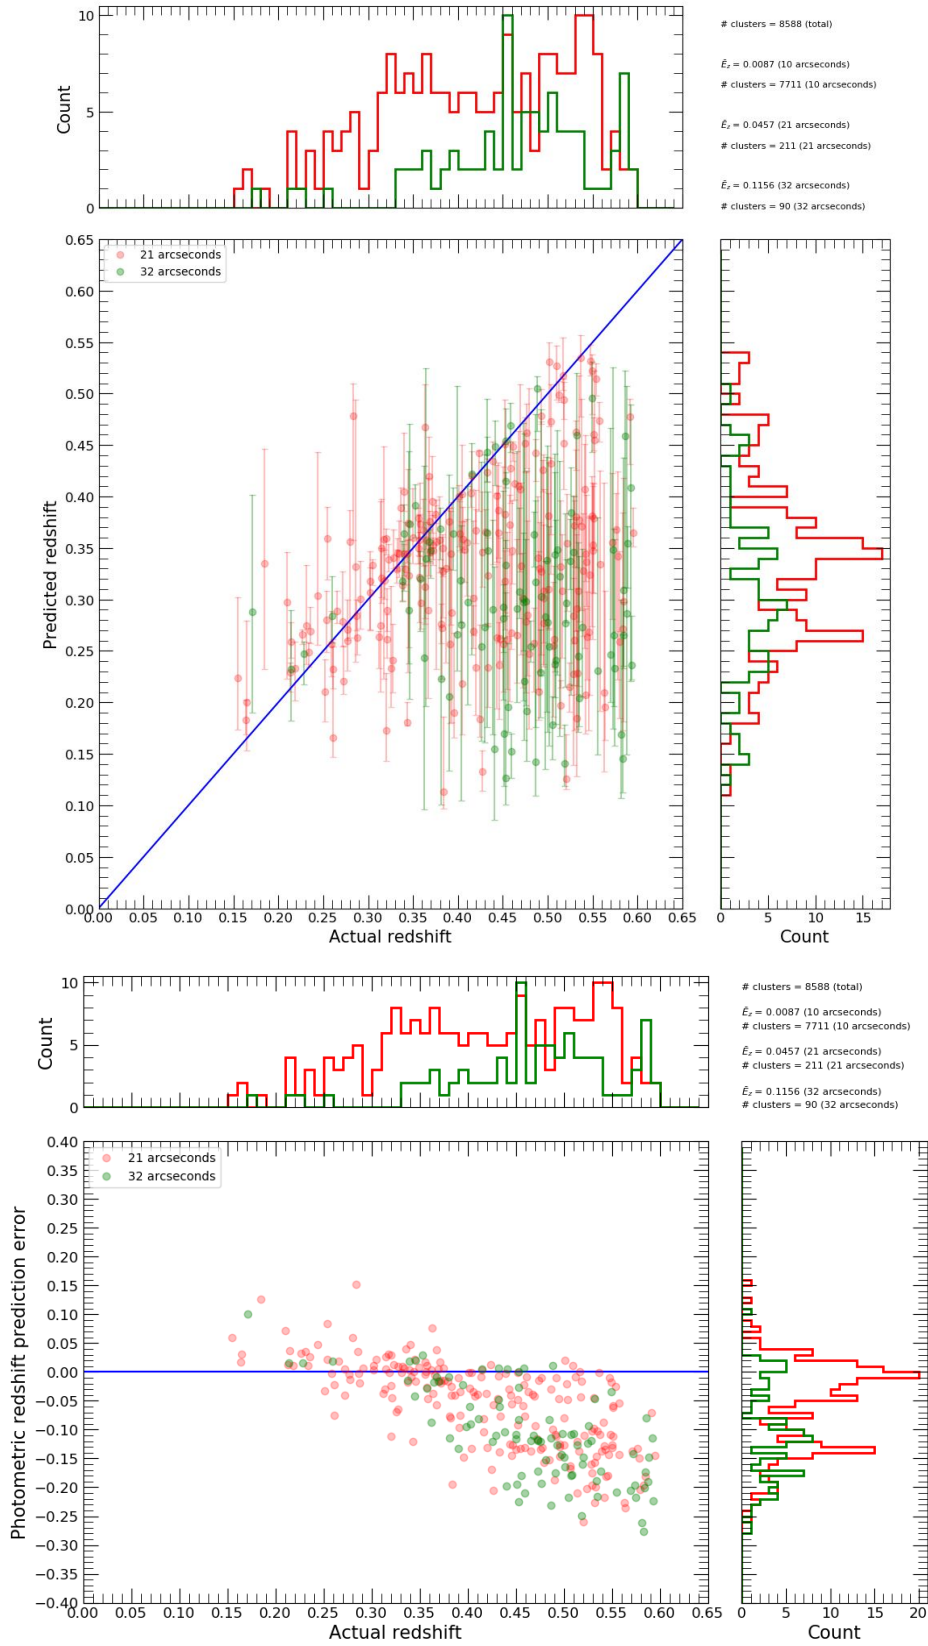

**Figure S46.** Plots displaying the performance of photometric redshift predictions of clusters with low richness, which did not qualify for the MWAR dataset, that had full bootstrap resamples returned within a 21 (red) or 32 (green) arcseconds search radii. If a cluster has no or partial bootstrap resamples returned at 10 arcseconds then the search radius is increased until a prediction with full bootstrap resamples returned is obtained. Top row: Predicted versus 'actual' photometric redshift of tested clusters with frequency histograms of the distributions. Bottom row: Non-absolute photometric redshift prediction error versus 'actual' redshift of tested clusters with frequency histograms of the distributions. Other: '# clusters (total)' represents the total number of clusters with low richness which did not qualify for the MWAR dataset, '# clusters' represents the number of clusters with low richness which did not qualify for the MWAR dataset that have observed galaxies within a 10, 21 and 32 arcseconds search radii with full bootstrap resamples returned,  $\bar{E}_z$  represents the median of photometric redshift prediction errors across all tested clusters within a 10, 21 and 32 arcseconds search radii with full bootstrap resamples returned.

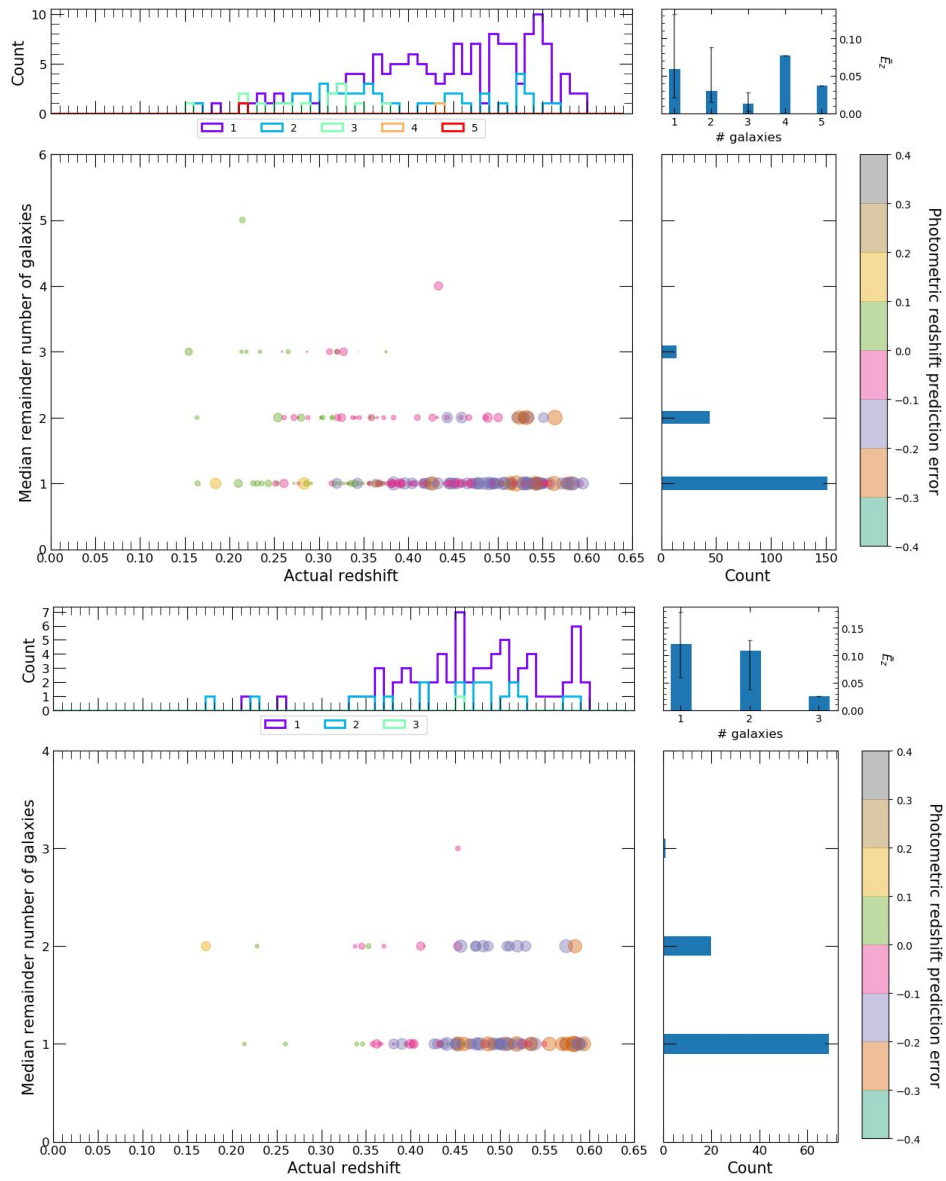

**Figure S47.** Plots displaying the number of galaxies used in photometric redshift predictions of clusters with low richness versus ‘actual’ redshift of tested clusters, which did not qualify for the MWAR dataset, where predictions had full bootstrap resamples returned within a 21 (top row) or 32 (bottom row) arcseconds search radius. If a cluster has no or partial bootstrap resamples returned at 10 arcseconds then the search radius is increased until a prediction with full bootstrap resamples returned is obtained. It should be noted that the size of individual points change in relation to the value of the non-absolute photometric redshift prediction error. Frequency histograms of the distributions are also shown.  $\tilde{E}_z$  represents the median of photometric redshift prediction errors across all tested clusters for each number of galaxies bin.

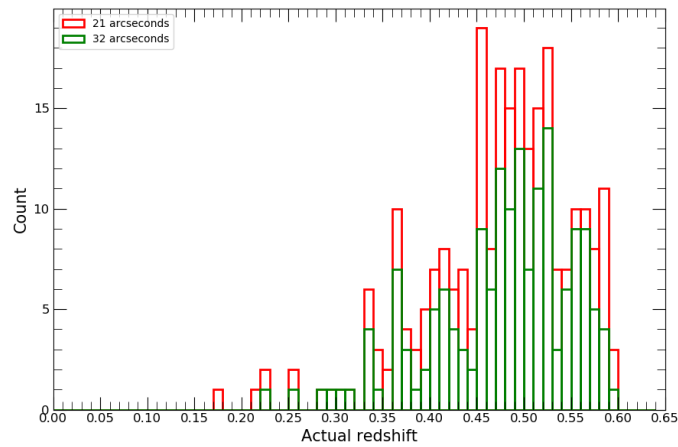

**Figure S48.** Frequency histograms displaying the ‘actual’ redshift distributions of clusters with low richness, which did not qualify for the MWAR dataset, that had no bootstrap resamples returned within a 21 (red) or 32 (green) arcseconds search radius.

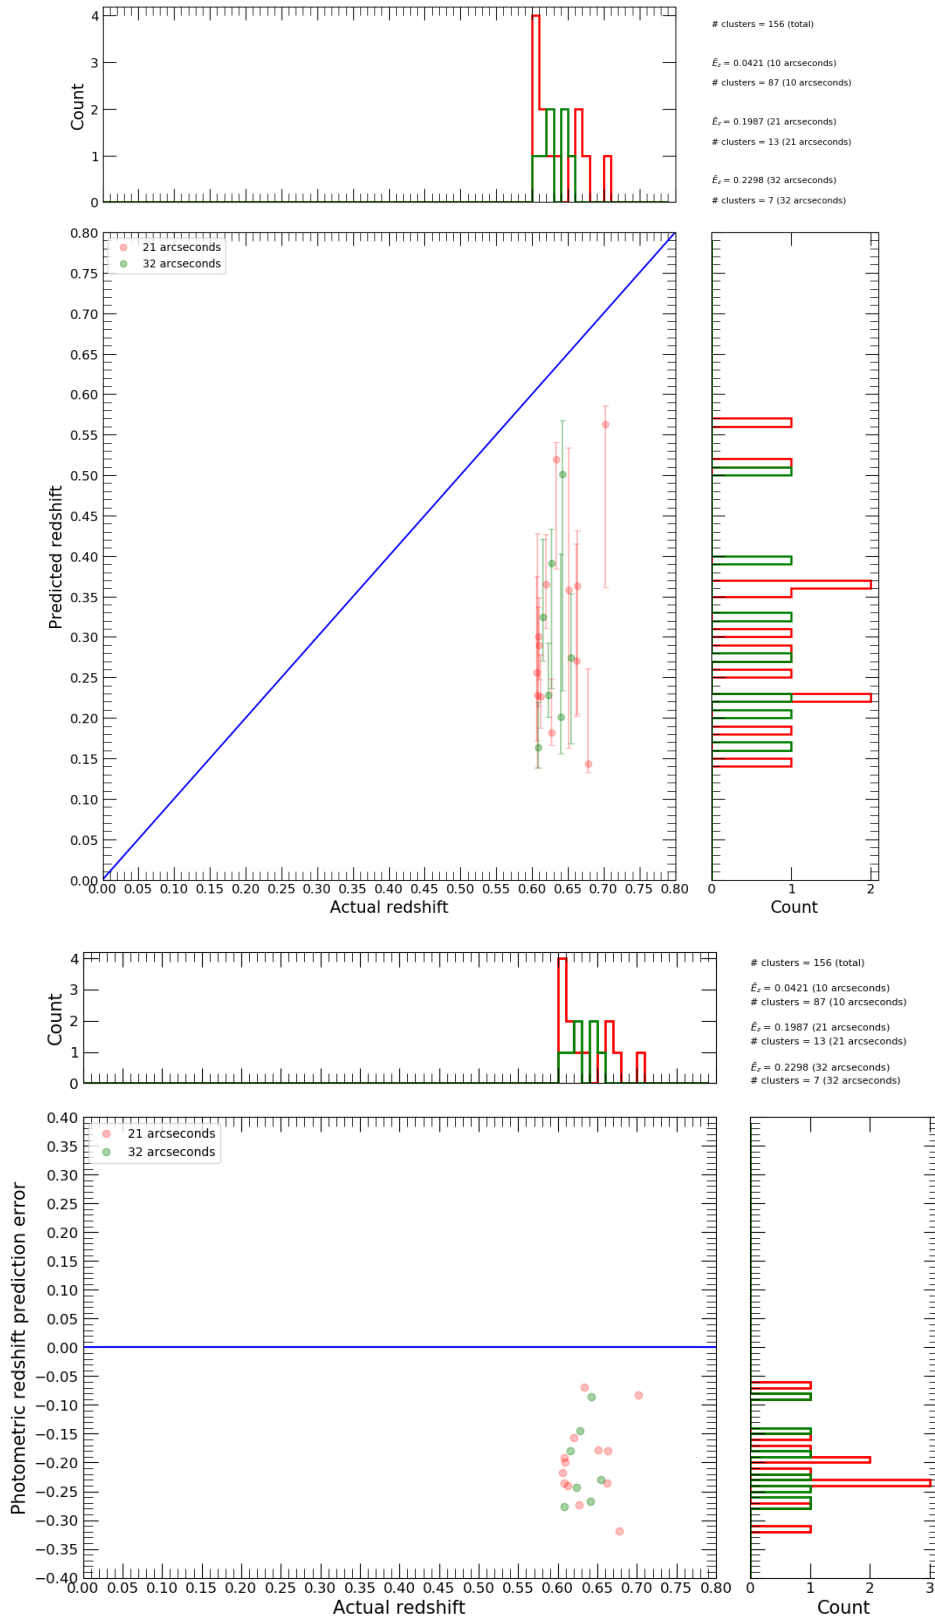

**Figure S49.** Plots displaying the performance of photometric redshift predictions of clusters at high redshift, which did not qualify for the WNMN dataset, that had full bootstrap resamples returned within a 21 (red) or 32 (green) arcseconds search radii. If a cluster has no or partial bootstrap resamples returned at 10 arcseconds then the search radius is increased until a prediction with full bootstrap resamples returned is obtained. Top row: Predicted versus 'actual' photometric redshift of tested clusters with frequency histograms of the distributions. Bottom row: Non-absolute photometric redshift prediction error versus 'actual' redshift of tested clusters with frequency histograms of the distributions. Other: '# clusters (total)' represents the total number of clusters at high redshift which did not qualify for the WNMN dataset, '# clusters' represents the number of clusters at high redshift which did not qualify for the WNMN dataset that have observed galaxies within a 10, 21 and 32 arcseconds search radii with full bootstrap resamples returned,  $\bar{E}_z$  represents the median of photometric redshift prediction errors across all tested clusters within a 10, 21 and 32 arcseconds search radii with full bootstrap resamples returned.

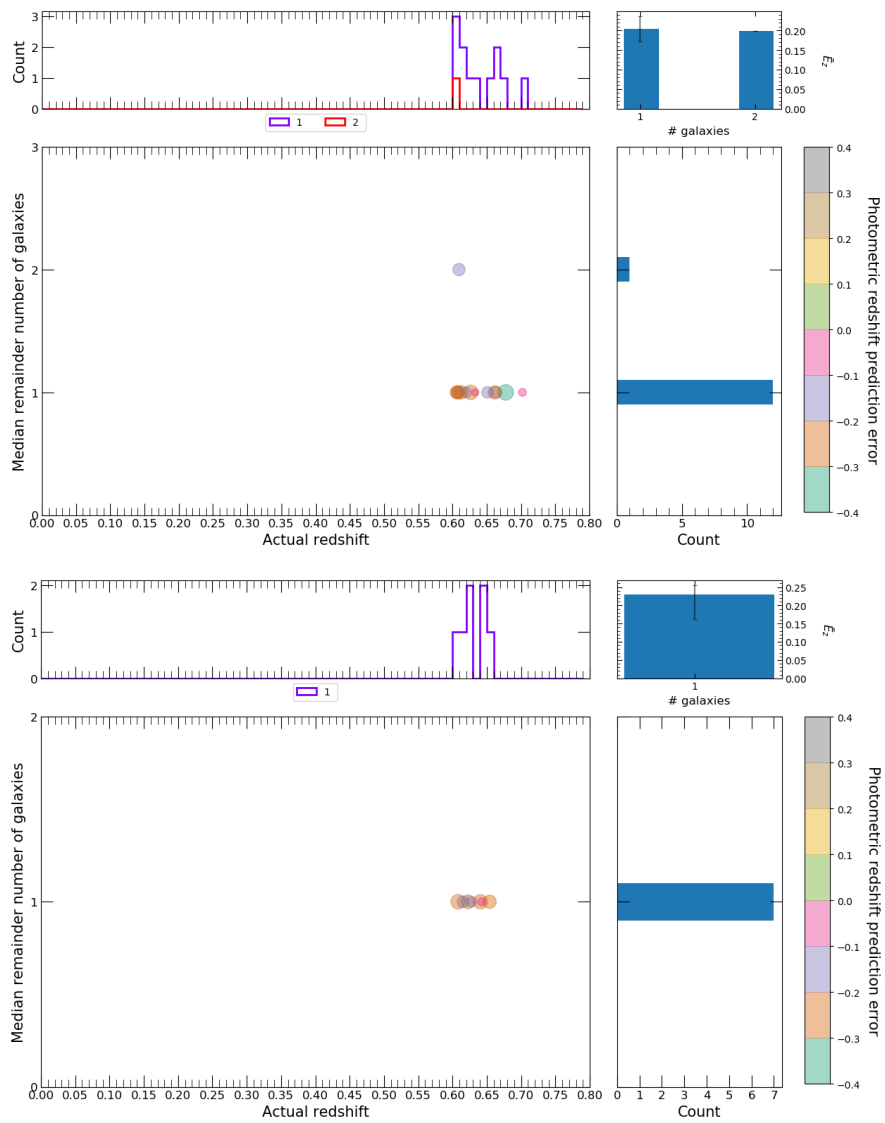

**Figure S50.** Plots displaying the number of galaxies used in photometric redshift predictions of clusters at high redshift versus 'actual' redshift of tested clusters, which did not qualify for the WNMR dataset, where predictions had full bootstrap resamples returned within a 21 (top row) or 32 (bottom row) arcseconds search radius. If a cluster has no or partial bootstrap resamples returned at 10 arcseconds then the search radius is increased until a prediction with full bootstrap resamples returned is obtained. It should be noted that the size of individual points change in relation to the value of the non-absolute photometric redshift prediction error. Frequency histograms of the distributions are also shown.  $\tilde{E}_z$  represents the median of photometric redshift prediction errors across all tested clusters for each number of galaxies bin.

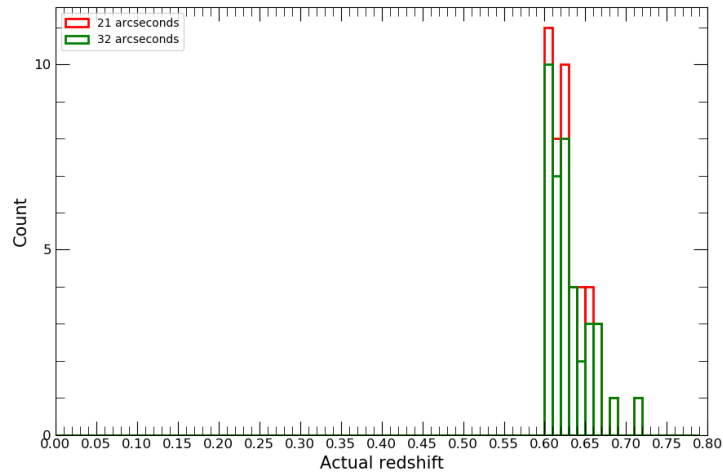

**Figure S51.** Frequency histograms displaying the 'actual' redshift distributions of clusters at high redshift, which did not qualify for the WNMR dataset, that had no bootstrap resamples returned within a 21 (red) or 32 (green) arcseconds search radius.

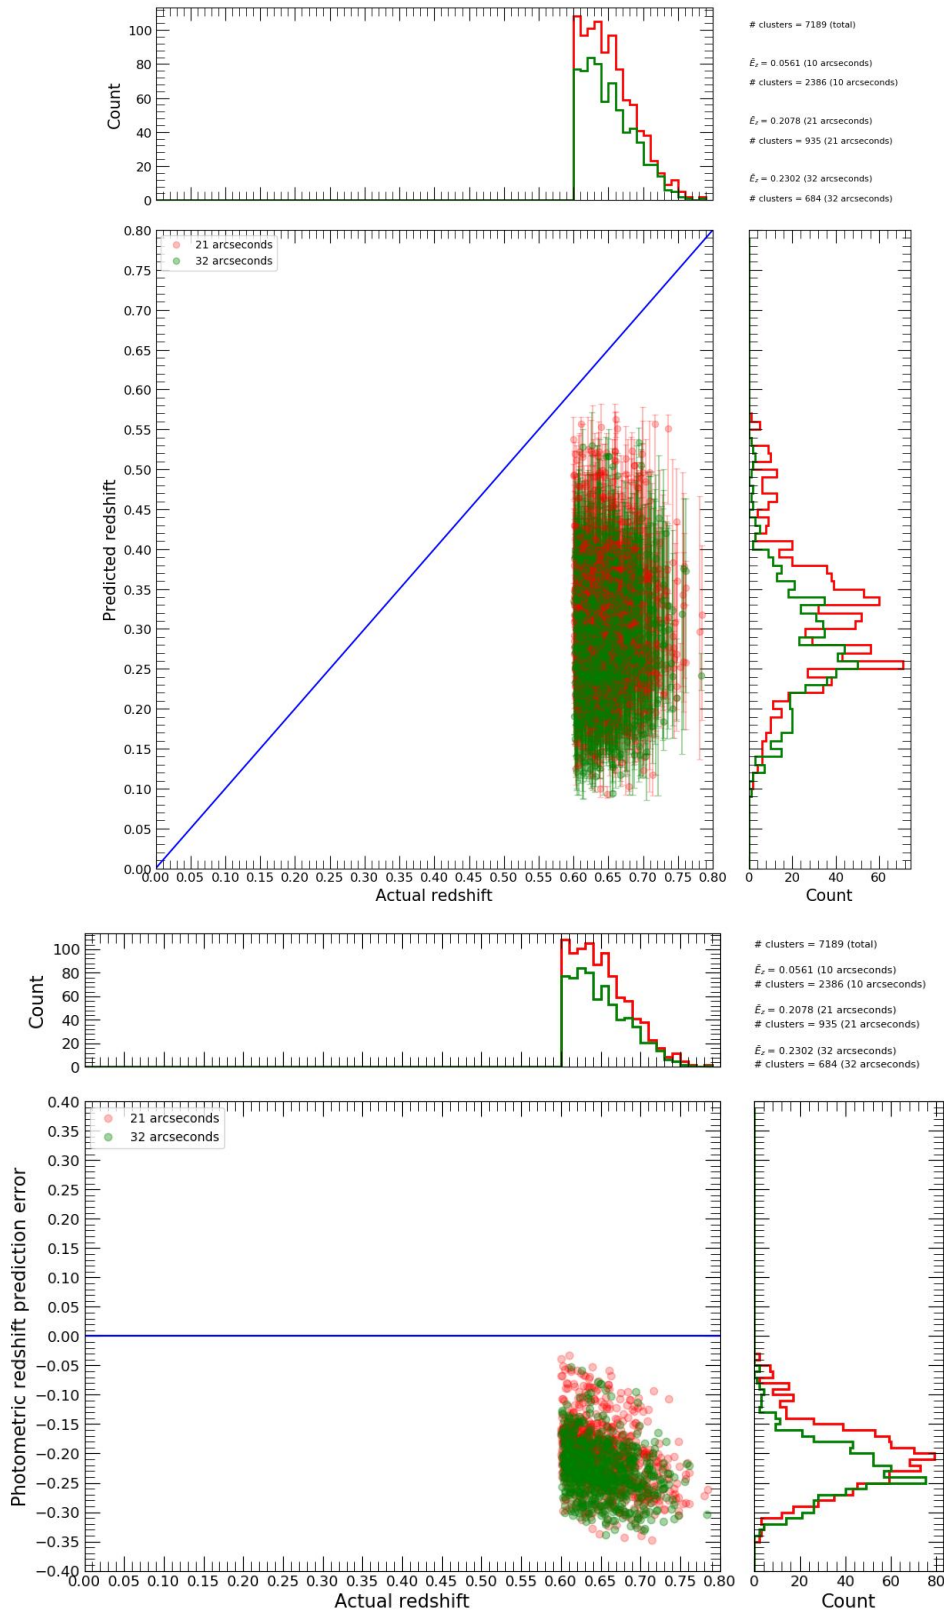

**Figure S52.** Plots displaying the performance of photometric redshift predictions of clusters at high redshift with low richness, which did not qualify for the WNMR dataset, that had full bootstrap resamples returned within a 21 (red) or 32 (green) arcseconds search radii. If a cluster has no or partial bootstrap resamples returned at 10 arcseconds then the search radius is increased until a prediction with full bootstrap resamples returned is obtained. Top row: Predicted versus 'actual' photometric redshift of tested clusters with frequency histograms of the distributions. Bottom row: Non-absolute photometric redshift prediction error versus 'actual' redshift of tested clusters with frequency histograms of the distributions. Other: '# clusters (total)' represents the total number of clusters at high redshift with low richness which did not qualify for the WNMR dataset, '# clusters' represents the number of clusters at high redshift with low richness which did not qualify for the WNMR dataset that have observed galaxies within a 10, 21 and 32 arcseconds search radii with full bootstrap resamples returned,  $\bar{E}_z$  represents the median of photometric redshift prediction errors across all tested clusters within a 10, 21 and 32 arcseconds search radii with full bootstrap resamples returned.



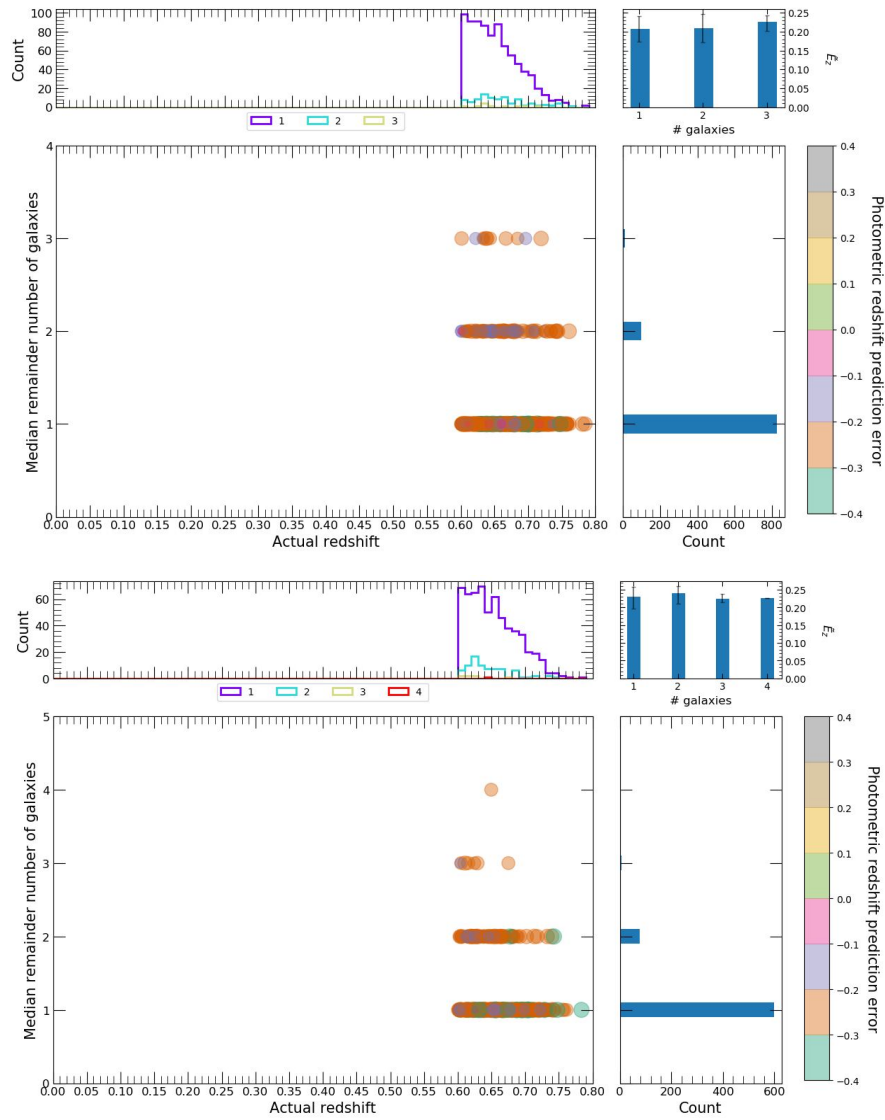

**Figure S53.** Plots displaying the number of galaxies used in photometric redshift predictions of clusters at high redshift with low richness versus ‘actual’ redshift of tested clusters, which did not qualify for the WNMR dataset, where predictions had full bootstrap resamples returned within a 21 (top row) or 32 (bottom row) arcseconds search radius. If a cluster has no or partial bootstrap resamples returned at 10 arcseconds then the search radius is increased until a prediction with full bootstrap resamples returned is obtained. It should be noted that the size of individual points change in relation to the value of the non-absolute photometric redshift prediction error. Frequency histograms of the distributions are also shown.  $\bar{E}_z$  represents the median of photometric redshift prediction errors across all tested clusters for each number of galaxies bin.

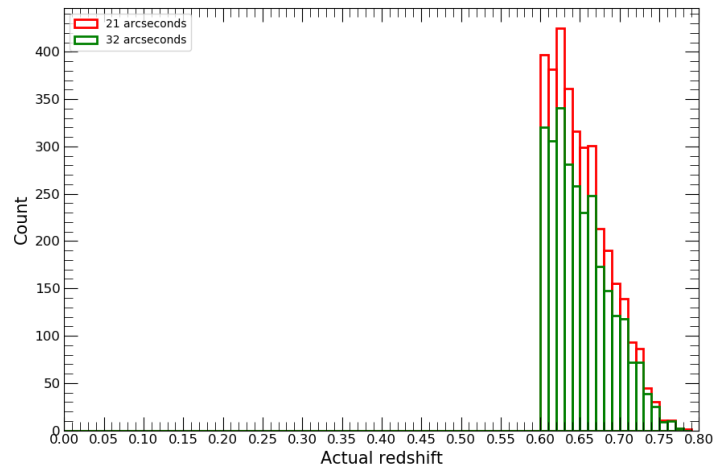

**Figure S54.** Frequency histograms displaying the ‘actual’ redshift distributions of clusters at high redshift with low richness, which did not qualify for the WNMR dataset, that had no bootstrap resamples returned within a 21 (red) or 32 (green) arcseconds search radius.

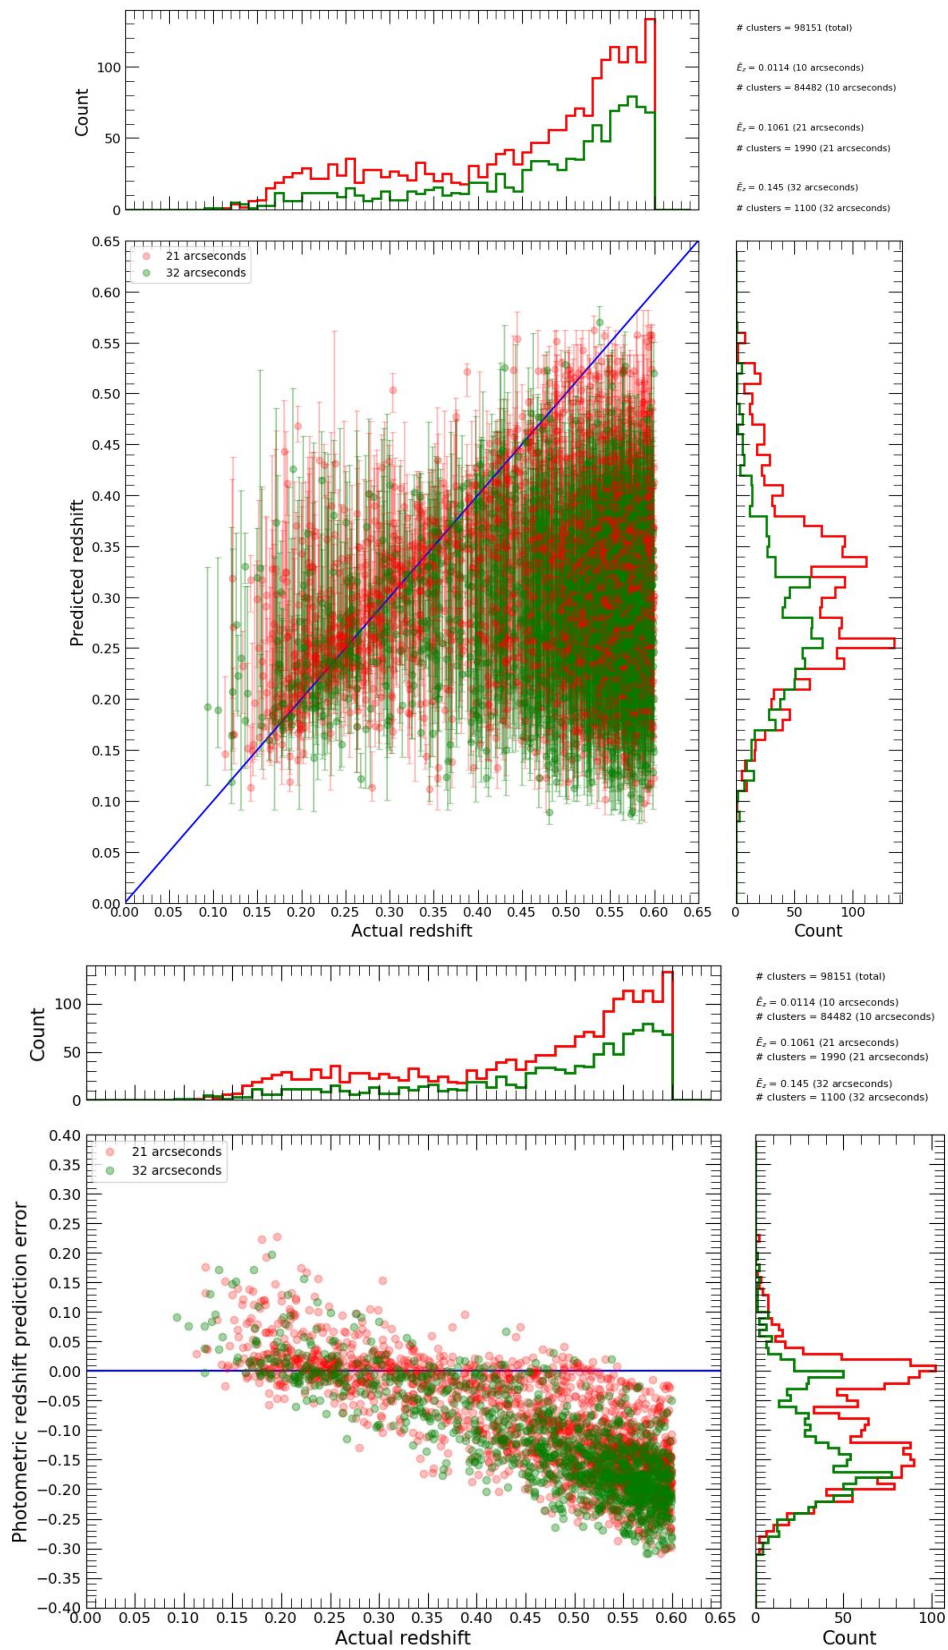

**Figure S55.** Plots displaying the performance of photometric redshift predictions of clusters with low richness, which did not qualify for the WNMR dataset, that had full bootstrap resamples returned within a 21 (red) or 32 (green) arcseconds search radii. If a cluster has no or partial bootstrap resamples returned at 10 arcseconds then the search radius is increased until a prediction with full bootstrap resamples returned is obtained. Top row: Predicted versus 'actual' photometric redshift of tested clusters with frequency histograms of the distributions. Bottom row: Non-absolute photometric redshift prediction error versus 'actual' redshift of tested clusters with frequency histograms of the distributions. Other: '# clusters (total)' represents the total number of clusters with low richness which did not qualify for the WNMR dataset, '# clusters' represents the number of clusters with low richness which did not qualify for the WNMR dataset that have observed galaxies within a 10, 21 and 32 arcseconds search radii with full bootstrap resamples returned,  $\bar{E}_z$  represents the median of photometric redshift prediction errors across all tested clusters within a 10, 21 and 32 arcseconds search radii with full bootstrap resamples returned.

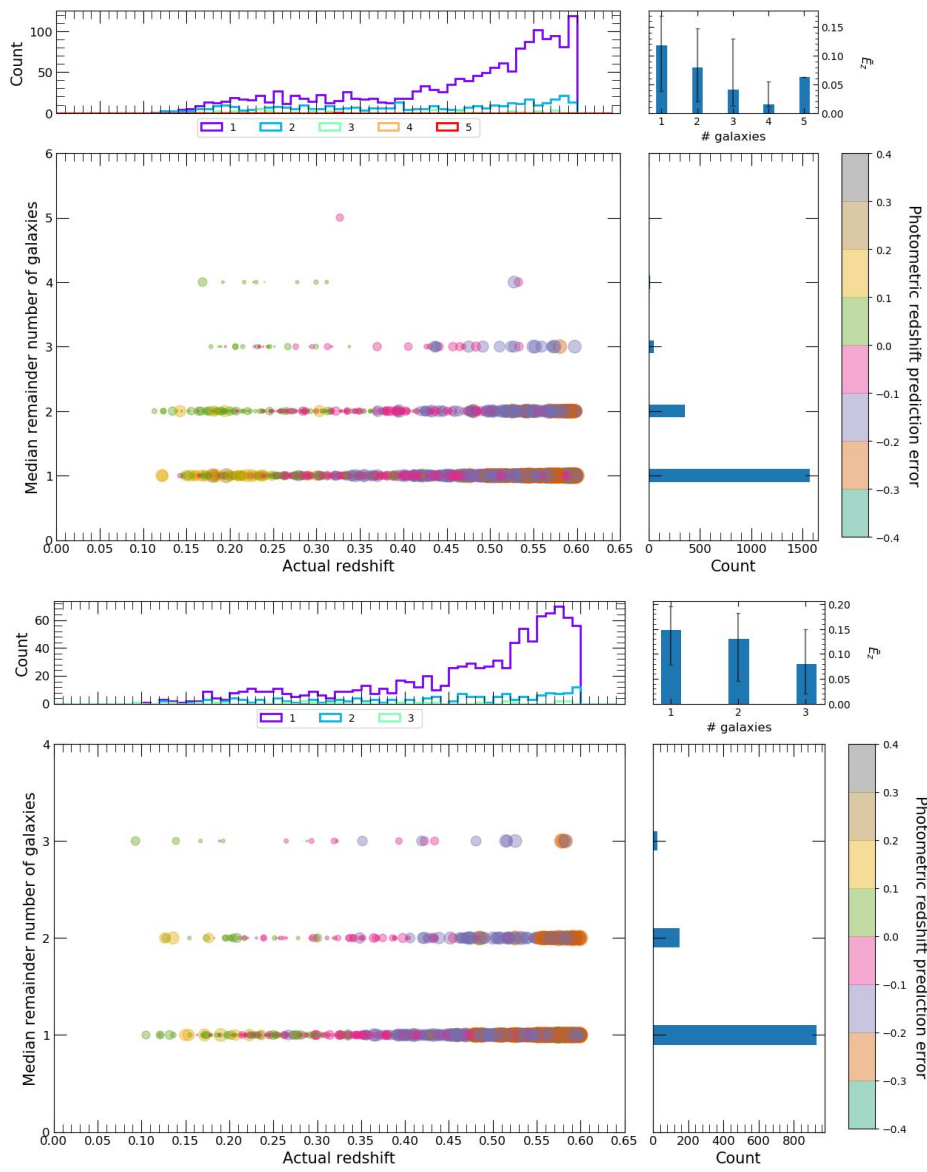

**Figure S56.** Plots displaying the number of galaxies used in photometric redshift predictions of clusters with low richness versus ‘actual’ redshift of tested clusters, which did not qualify for the WNMR dataset, where predictions had full bootstrap resamples returned within a 21 (top row) or 32 (bottom row) arcseconds search radius. If a cluster has no or partial bootstrap resamples returned at 10 arcseconds then the search radius is increased until a prediction with full bootstrap resamples returned is obtained. It should be noted that the size of individual points change in relation to the value of the non-absolute photometric redshift prediction error. Frequency histograms of the distributions are also shown.  $\bar{E}_z$  represents the median of photometric redshift prediction errors across all tested clusters for each number of galaxies bin.

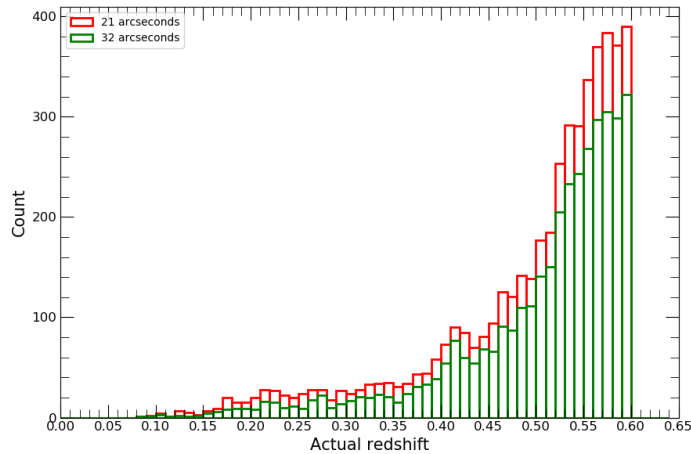

**Figure S57.** Frequency histograms displaying the ‘actual’ redshift distributions of clusters with low richness, which did not qualify for the WNMR dataset, that had no bootstrap resamples returned within a 21 (red) or 32 (green) arcseconds search radius.

## APPENDIX

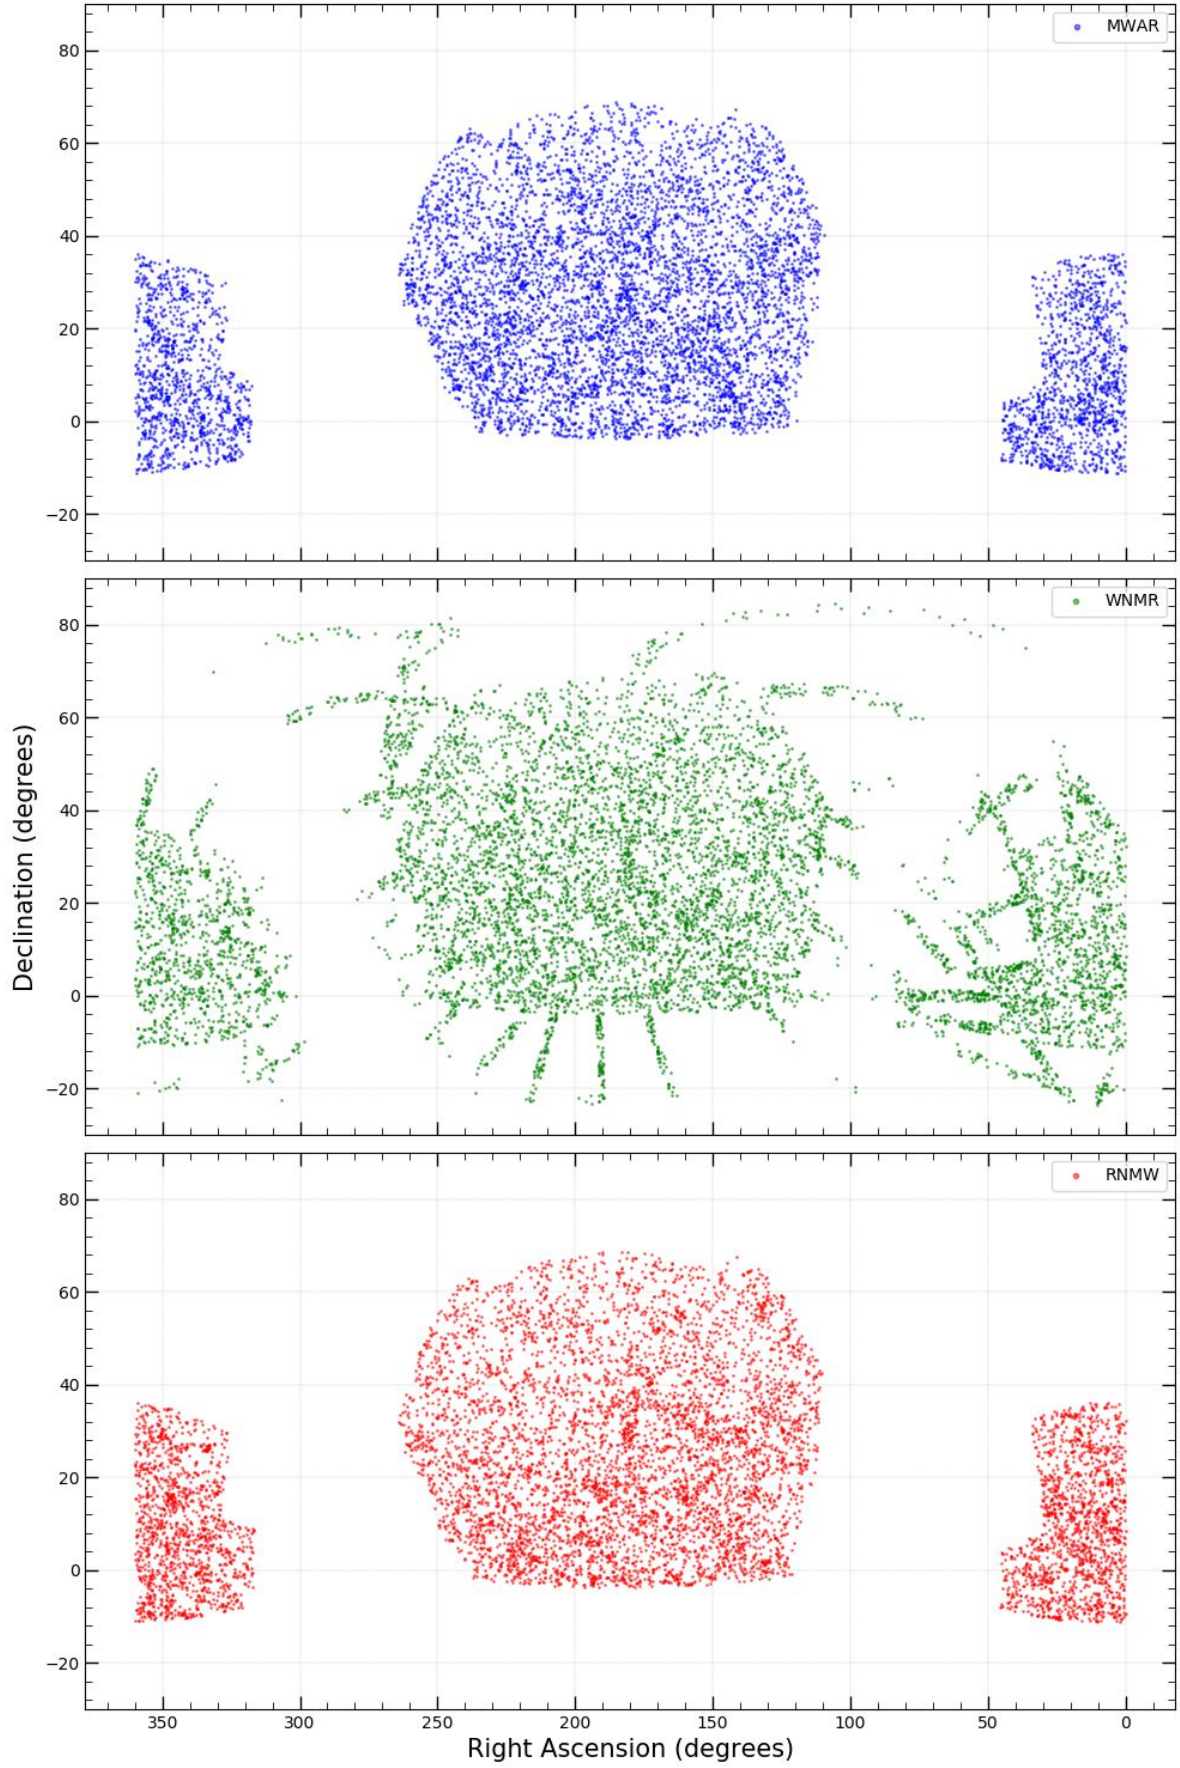

**Figure SA1.** Astronomical sky maps with the J2000 epoch coordinate system displaying the observed positions of clusters in the MWAR (top row), WNMR (middle row) and RNMW (bottom row) datasets.



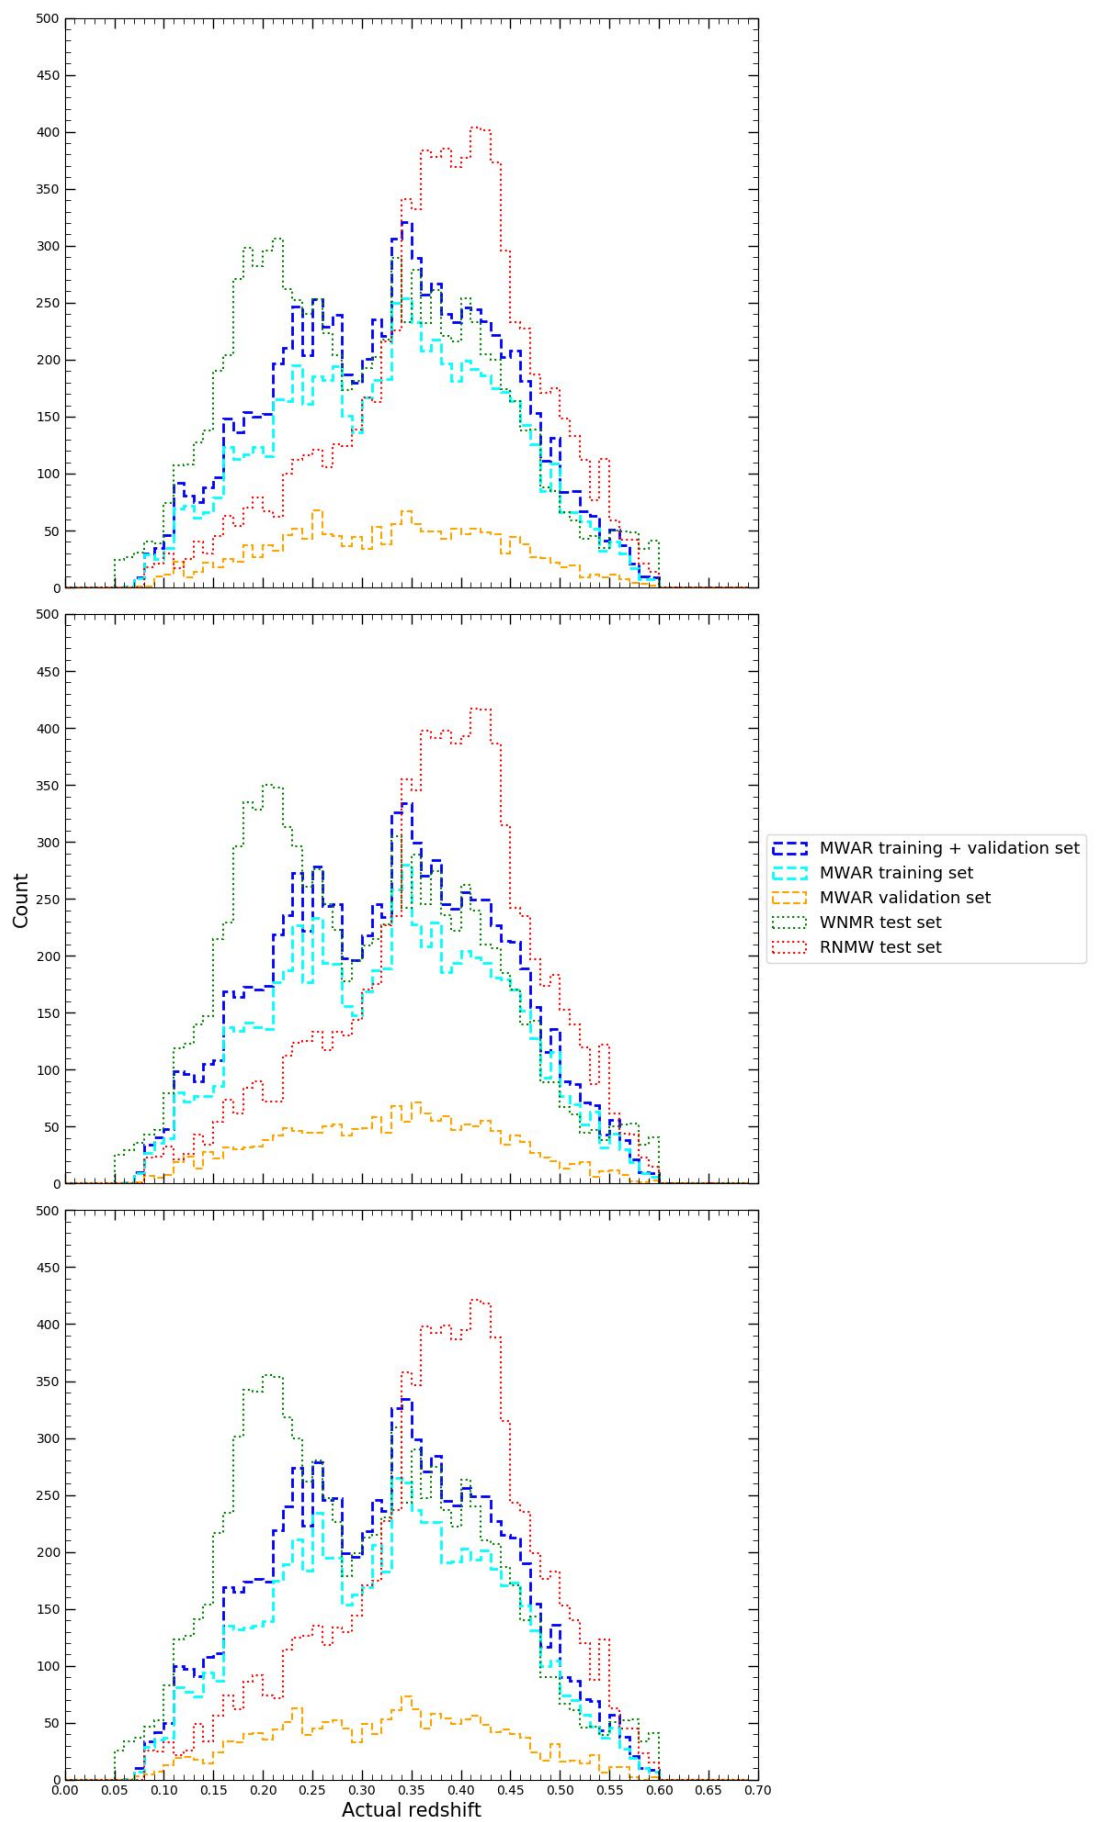

**Figure SA2.** Frequency histograms of the 'actual' redshift distributions, where photometric redshifts of clusters in the MWAR dataset (blue dashed line), MWAR training set (cyan dashed line), MWAR validation set (orange dashed line) and WNMR test set (green dotted line) are originally estimated by WHL12. Whilst photometric redshifts of clusters in the RNMW test set (red dotted line) are originally estimated by redMaPPer. The top row contains clusters within a 10 arcseconds search radius, the middle row contains clusters within a 21 arcseconds search radius and the bottom row contains clusters within a 32 arcseconds search radius.

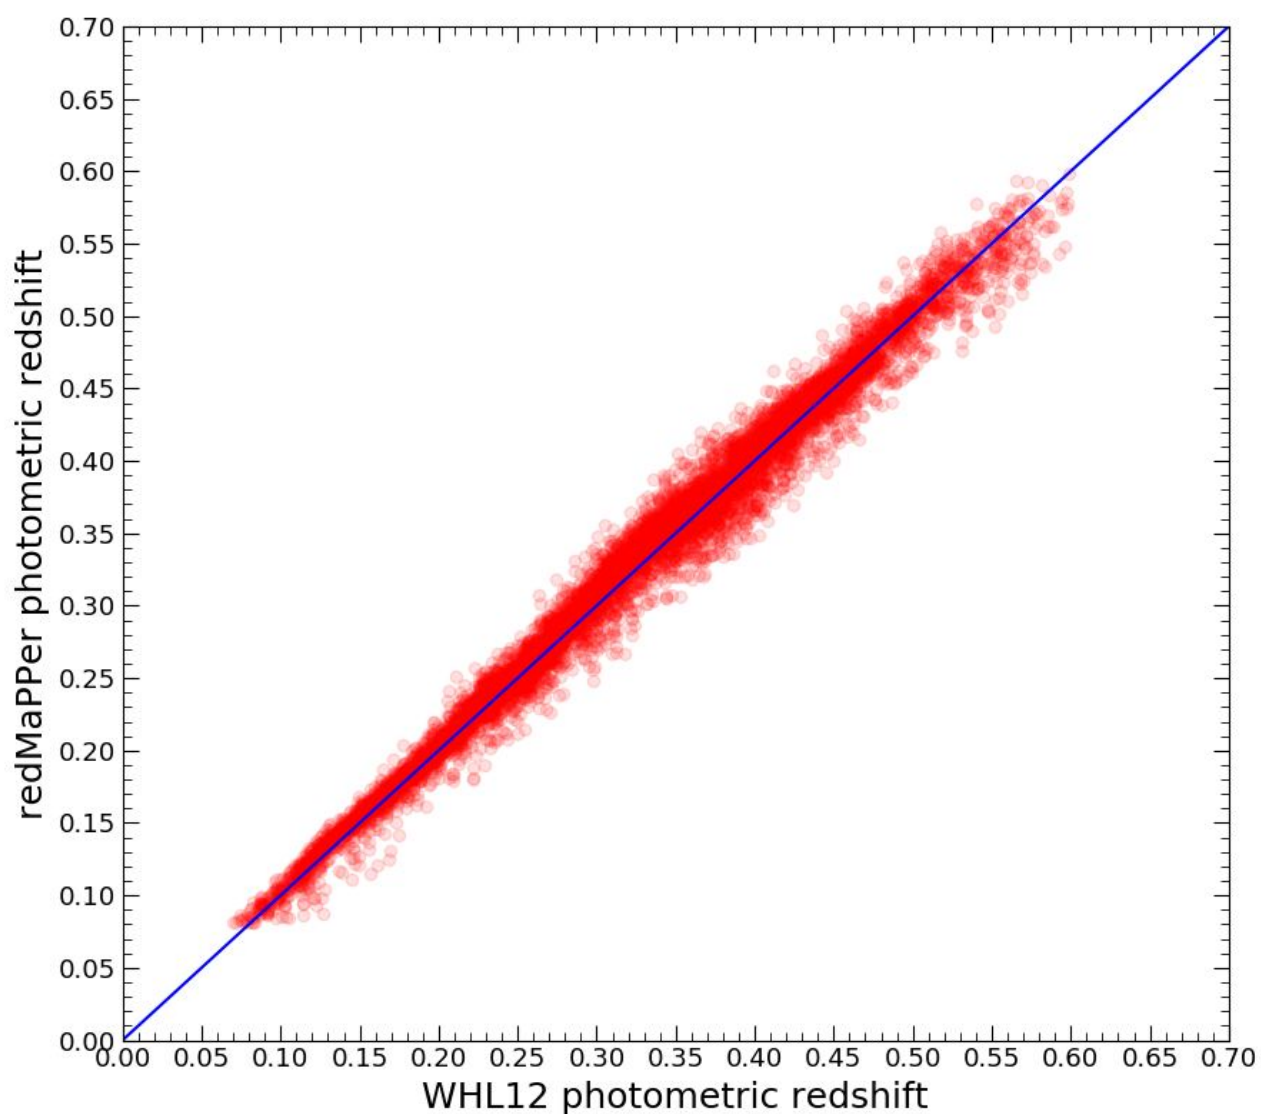

**Figure SA3.** Comparison of photometric redshifts for clusters in the MWAR dataset that are originally estimated by the WHL12 and redMaPPer cluster catalogues.



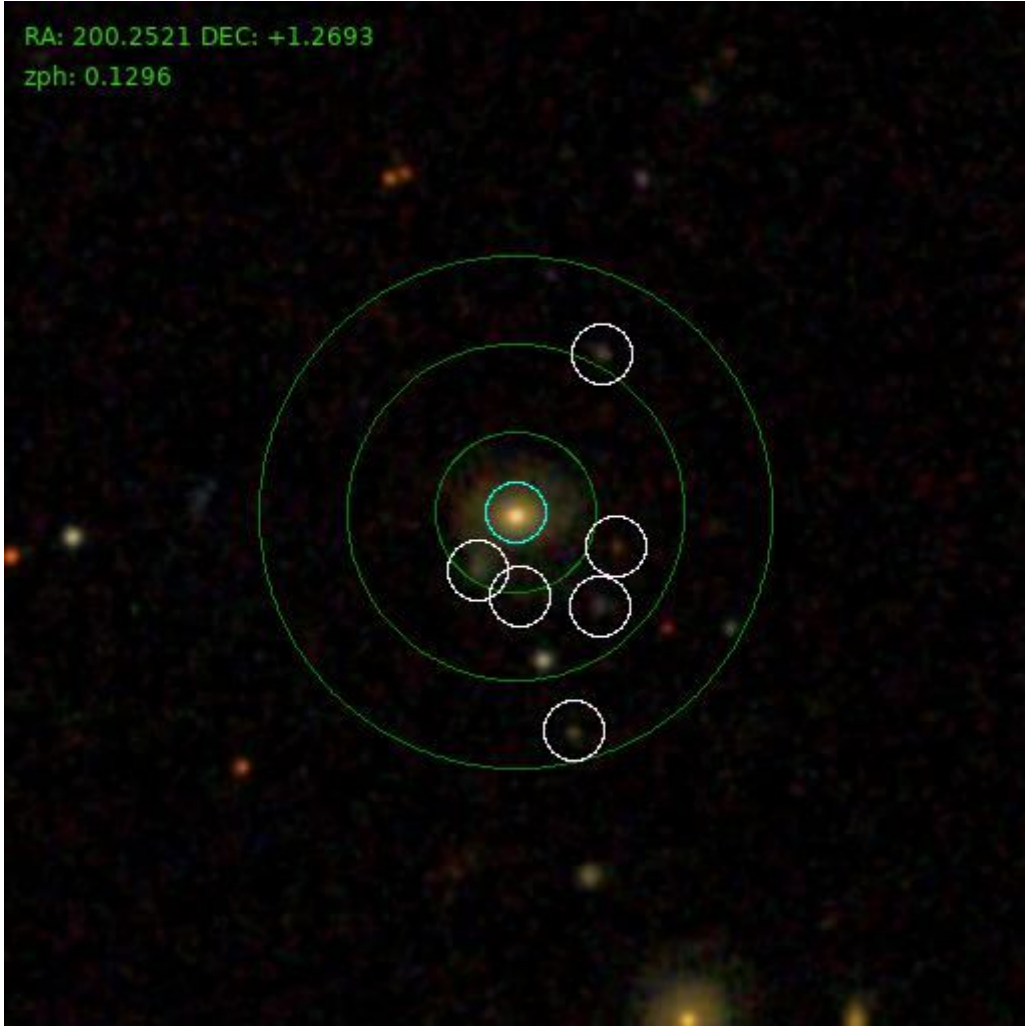

**Figure SA4.** An SDSS image of a cluster from the WNMR test set with J2000 coordinates of RA: 200.2521 and Dec: +1.2693. The cluster has a photometric redshift of  $z_{ph}: 0.1296$  in the WHL12 cluster catalogue. The green circles represent the size of the 10, 21 and 32 arcseconds search radii respectively. Any objects with no circle surrounding it within the 32 arcseconds search radius is not considered to be a galaxy or is a galaxy with poor photometry. The white circles represent galaxies with ‘clean’ photometry, as determined by SDSS, found within the 32 arcseconds search radius that are removed if all LM-0.5 filter magnitude-cuts (excluding the u filter) for the 32 arcseconds search radius are applied at the same time. The cyan circles represent galaxies with also ‘clean’ photometry, as determined by SDSS, found within the 32 arcseconds search radius that remain if all LM-0.5 filter magnitude-cuts (excluding the u filter) for the 32 arcseconds search radius are applied at the same time. From which, we find that only the central galaxy remains within the 32 arcseconds search radius, such that the tuned model returns photometric redshift estimates of  $z_{ph}: 0.1269$  with  $CI_{95\%}=[0.0961, 0.3093]$  for the 10 arcseconds search radius,  $z_{ph}: 0.1092$  with  $CI_{95\%}=[0.0893, 0.4661]$  for the 21 arcseconds search radius and  $z_{ph}: 0.3976$  with  $CI_{95\%}=[0.1526, 0.4918]$  for the 32 arcseconds search radius. This example shows that the training set itself can contaminate model predictions when a larger search radius is applied, as we observe that no interloping galaxies are included when the 32 arcseconds search radius is used.

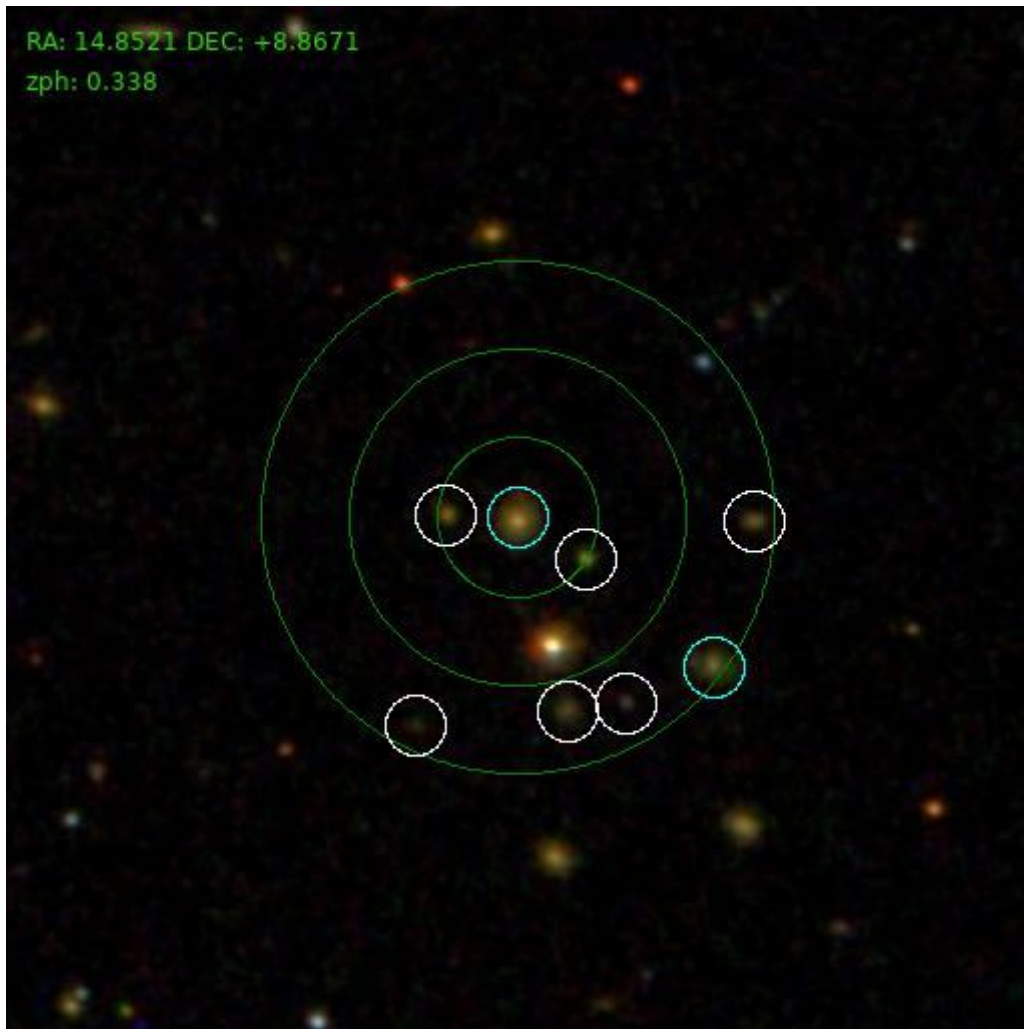

**Figure SA5.** An SDSS image of a cluster from the WNMR test set with J2000 coordinates of RA: 14.8521 and Dec: +8.8671. The cluster has a photometric redshift of  $z_{ph}$ : 0.338 in the WHL12 cluster catalogue. The green circles represent the size of the 10, 21 and 32 arcseconds search radii respectively. Any objects with no circle surrounding it within the 32 arcseconds search radius is not considered to be a galaxy or is a galaxy with poor photometry. The white circles represent galaxies with 'clean' photometry, as determined by SDSS, found within the 32 arcseconds search radius that are removed if all LM-0.5 filter magnitude-cuts (excluding the u filter) for the 32 arcseconds search radius are applied at the same time. The cyan circles represent galaxies with also 'clean' photometry, as determined by SDSS, found within the 32 arcseconds search radius that remain if all LM-0.5 filter magnitude-cuts (excluding the u filter) for the 32 arcseconds search radius are applied at the same time. From which, we find that the central galaxy and another galaxy remains within the 32 arcseconds search radius, such that the tuned model returns photometric redshift estimates of  $z_{ph}$ : 0.1859 with  $CI_{95\%}=[0.1664, 0.2261]$  for the 10 arcseconds search radius,  $z_{ph}$ : 0.1877 with  $CI_{95\%}=[0.1653, 0.2519]$  for the 21 arcseconds search radius and  $z_{ph}$ : 0.1651 with  $CI_{95\%}=[0.1431, 0.2001]$  for the 32 arcseconds search radius. This example shows that the training set itself can contaminate model predictions at all search radii, as we observe that no obvious interloping galaxies are included for any search radii.

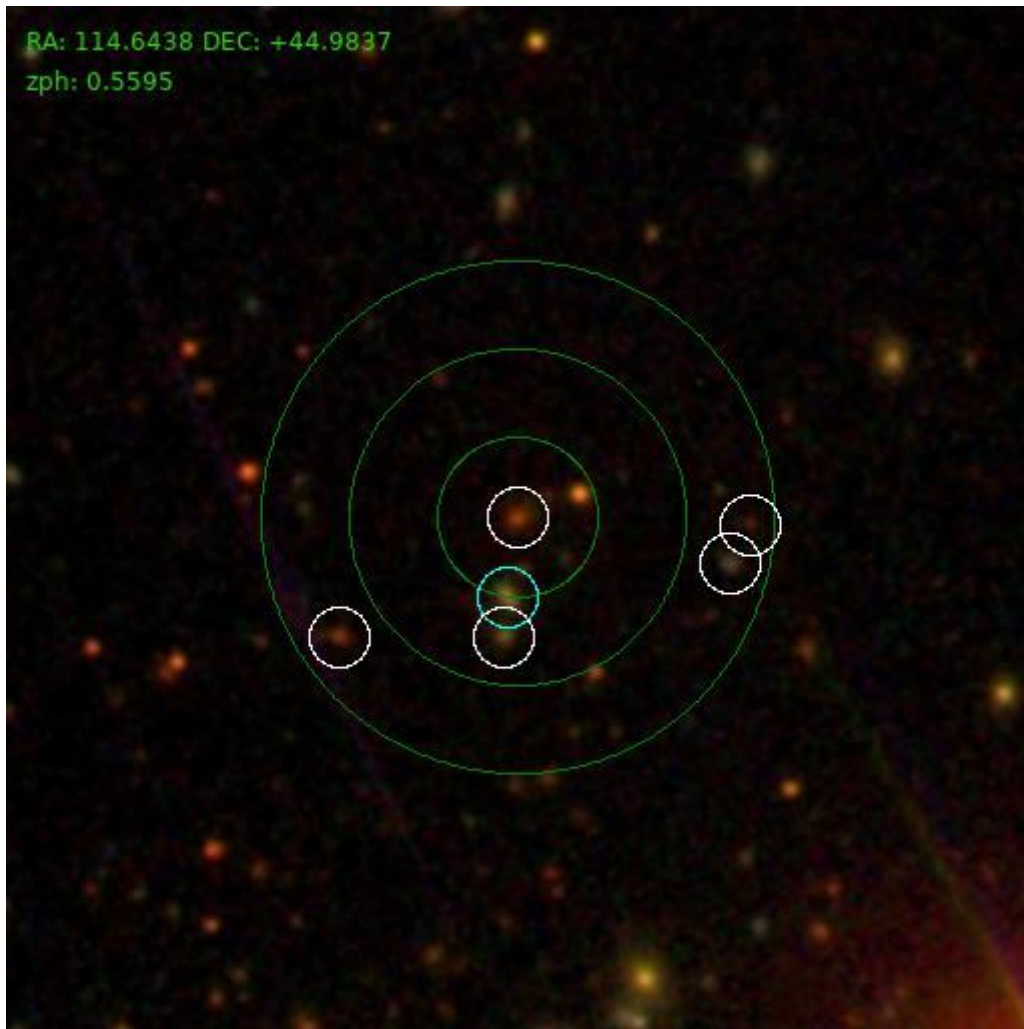

**Figure SA6.** An SDSS image of a cluster from the WNMR test set with J2000 coordinates of RA: 114.6438 and Dec: +44.9837. The cluster has a photometric redshift of  $z_{ph}$ : 0.5595 in the WHL12 cluster catalogue. The green circles represent the size of the 10, 21 and 32 arcseconds search radii respectively. Any objects with no circle surrounding it within the 32 arcseconds search radius is not considered to be a galaxy or is a galaxy with poor photometry. The white circles represent galaxies with ‘clean’ photometry, as determined by SDSS, found within the 32 arcseconds search radius that are removed if all LM-0.5 filter magnitude-cuts (excluding the u filter) for the 32 arcseconds search radius are applied at the same time. The cyan circles represent galaxies with also ‘clean’ photometry, as determined by SDSS, found within the 32 arcseconds search radius that remain if all LM-0.5 filter magnitude-cuts (excluding the u filter) for the 32 arcseconds search radius are applied at the same time. From which, we find that an interloping galaxy remains within the 32 arcseconds search radius, such that the tuned model returns photometric redshift estimates of  $z_{ph}$ : 0.1730 with  $CI_{95\%}=[0.1153, 0.2350]$  for the 10 arcseconds search radius,  $z_{ph}$ : 0.2399 with  $CI_{95\%}=[0.1960, 0.2710]$  for the 21 arcseconds search radius and  $z_{ph}$ : 0.1637 with  $CI_{95\%}=[0.1152, 0.3672]$  for the 32 arcseconds search radius. This example shows that an interloping galaxy within the 10 arcseconds search radius, presumably at lower redshift than the cluster itself, can contaminate model predictions for all search radii.

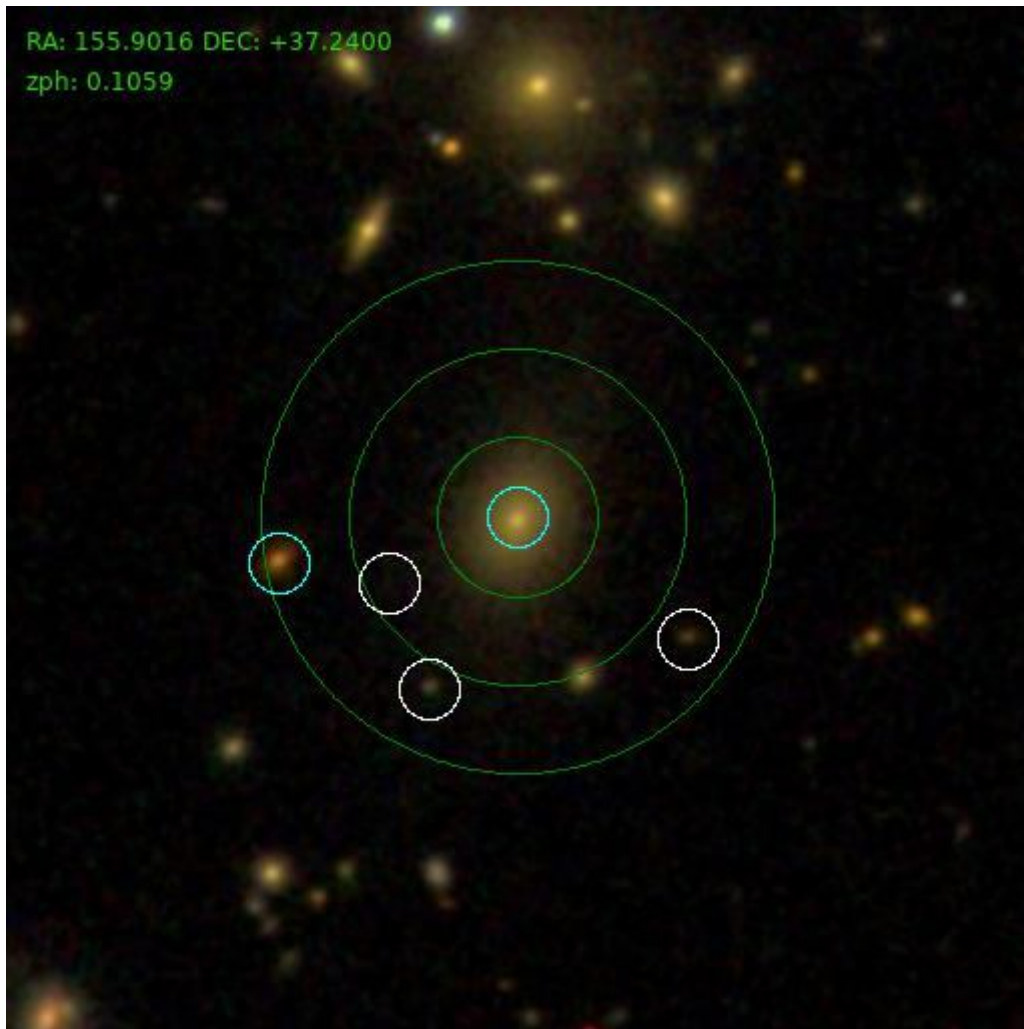

**Figure SA7.** An SDSS image of a cluster from the RNMW test set with J2000 coordinates of RA: 155.9016 and Dec: +37.2400. The cluster has a photometric redshift of  $z_{ph}: 0.1059$  in the redMaPPer cluster catalogue. The green circles represent the size of the 10, 21 and 32 arcseconds search radii respectively. Any objects with no circle surrounding it within the 32 arcseconds search radius is not considered to be a galaxy or is a galaxy with poor photometry. The white circles represent galaxies with 'clean' photometry, as determined by SDSS, found within the 32 arcseconds search radius that are removed if all LM-0.5 filter magnitude-cuts (excluding the u filter) for the 32 arcseconds search radius are applied at the same time. The cyan circles represent galaxies with also 'clean' photometry, as determined by SDSS, found within the 32 arcseconds search radius that remain if all LM-0.5 filter magnitude-cuts (excluding the u filter) for the 32 arcseconds search radius are applied at the same time. From which, we find that the central galaxy and an interloping galaxy remains within the 32 arcseconds search radius, such that the tuned model returns photometric redshift estimates of  $z_{ph}: 0.1115$  with  $CI_{95\%}=[0.0914, 0.1239]$  for the 10 arcseconds search radius,  $z_{ph}: 0.1121$  with  $CI_{95\%}=[0.1024, 0.1198]$  for the 21 arcseconds search radius and  $z_{ph}: 0.2709$  with  $CI_{95\%}=[0.1972, 0.4003]$  for the 32 arcseconds search radius. This example shows that an interloping galaxy, presumably at higher redshift than the cluster itself, can contaminate model predictions when the search radius increases.



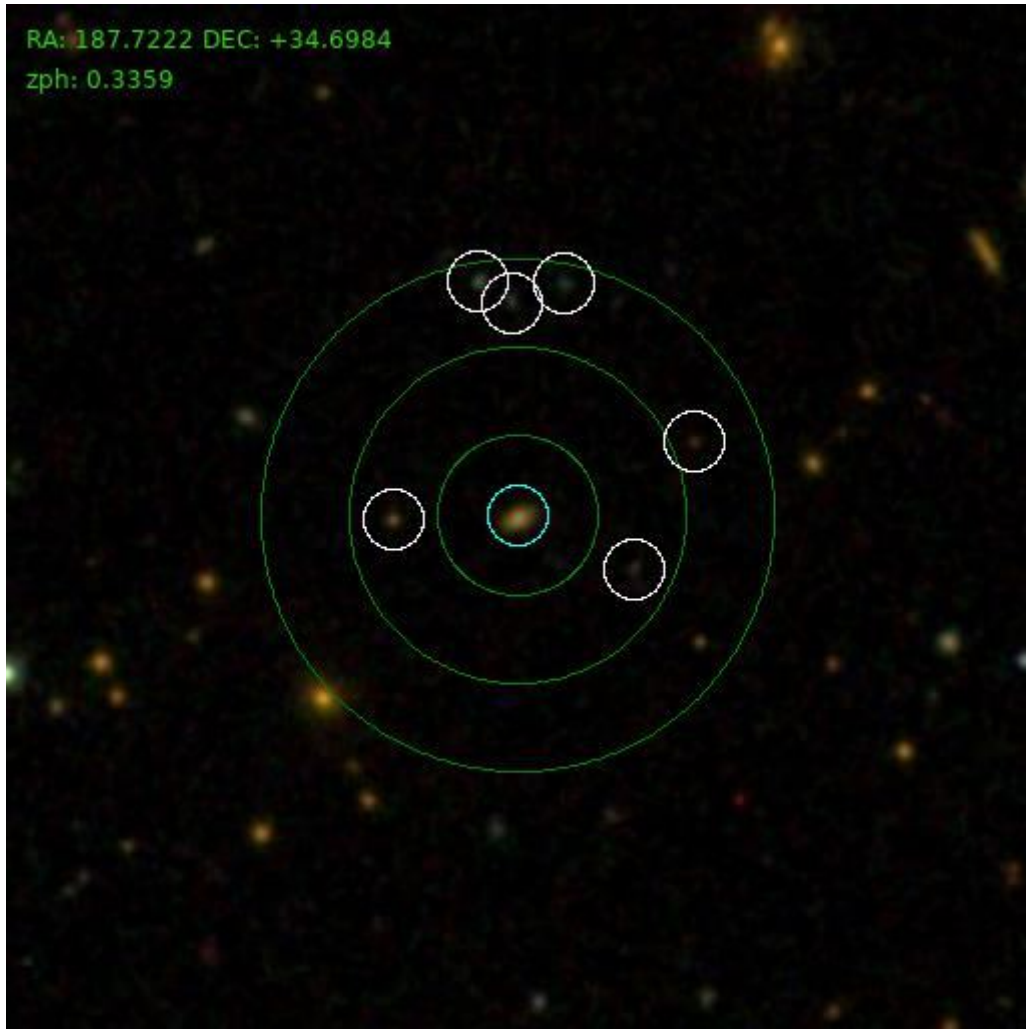

**Figure SA8.** An SDSS image of a cluster from the RNMW test set with J2000 coordinates of RA: 187.7222 and Dec: +34.6984. The cluster has a photometric redshift of  $z_{ph}: 0.3359$  in the redMaPPer cluster catalogue. The green circles represent the size of the 10, 21 and 32 arcseconds search radii respectively. Any objects with no circle surrounding it within the 32 arcseconds search radius is not considered to be a galaxy or is a galaxy with poor photometry. The white circles represent galaxies with 'clean' photometry, as determined by SDSS, found within the 32 arcseconds search radius that are removed if all LM-0.5 filter magnitude-cuts (excluding the u filter) for the 32 arcseconds search radius are applied at the same time. The cyan circles represent galaxies with also 'clean' photometry, as determined by SDSS, found within the 32 arcseconds search radius that remain if all LM-0.5 filter magnitude-cuts (excluding the u filter) for the 32 arcseconds search radius are applied at the same time. From which, we find that only the central galaxy remains within the 32 arcseconds search radius, such that the tuned model returns photometric redshift estimates of  $z_{ph}: 0.1664$  with  $CI_{95\%}=[0.1189, 0.1820]$  for the 10 arcseconds search radius,  $z_{ph}: 0.1617$  with  $CI_{95\%}=[0.1264, 0.2041]$  for the 21 arcseconds search radius and  $z_{ph}: 0.1474$  with  $CI_{95\%}=[0.1191, 0.2131]$  for the 32 arcseconds search radius. This example also shows that the training set itself can contaminate model predictions at all search radii, as we observe that no interloping galaxies are included for any search radii.

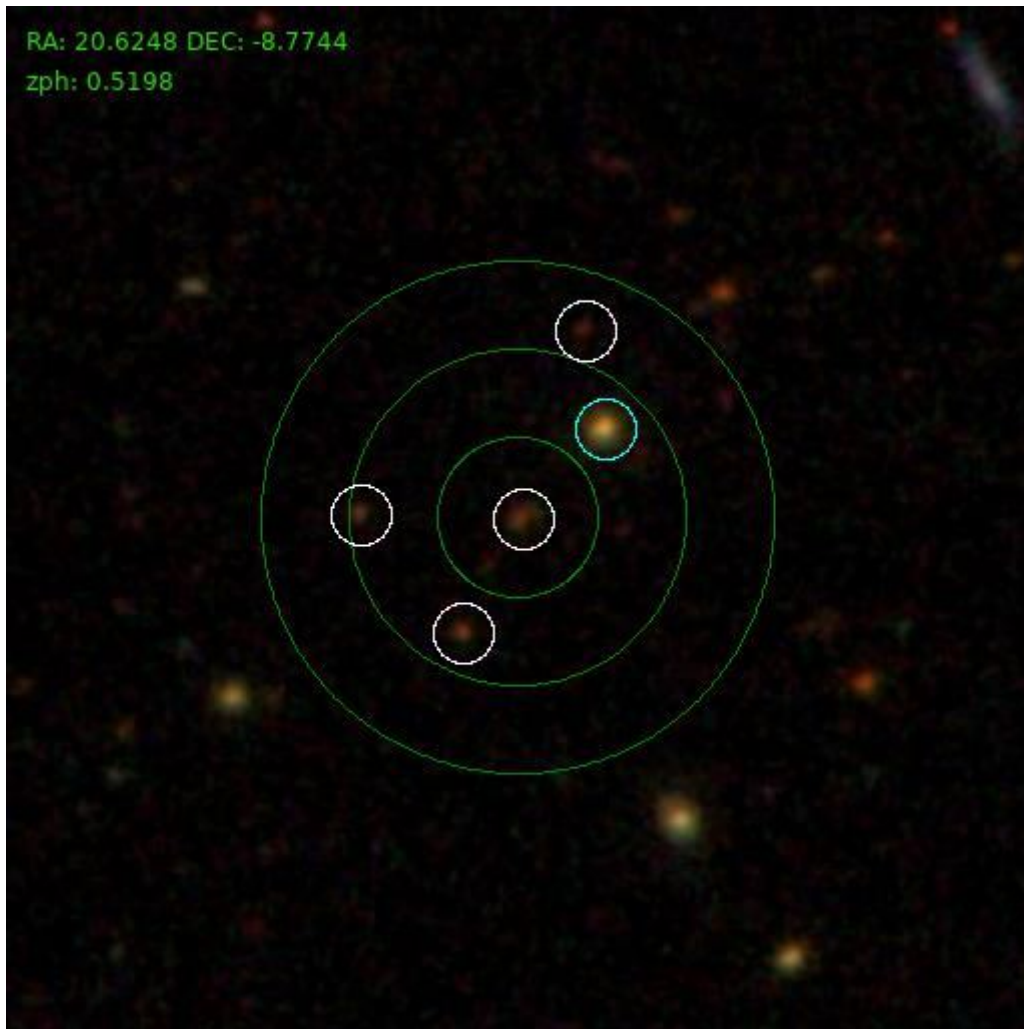

**Figure SA9.** An SDSS image of a cluster from the RNMW test set with J2000 coordinates of RA: 20.6248 and Dec: -8.7744. The cluster has a photometric redshift of  $z_{ph}: 0.5198$  in the redMaPPer cluster catalogue. The green circles represent the size of the 10, 21 and 32 arcseconds search radii respectively. Any objects with no circle surrounding it within the 32 arcseconds search radius is not considered to be a galaxy or is a galaxy with poor photometry. The white circles represent galaxies with ‘clean’ photometry, as determined by SDSS, found within the 32 arcseconds search radius that are removed if all LM-0.5 filter magnitude-cuts (excluding the u filter) for the 32 arcseconds search radius were applied at the same time. The cyan circles represent galaxies with also ‘clean’ photometry, as determined by SDSS, found within the 32 arcseconds search radius that remain if all LM-0.5 filter magnitude-cuts (excluding the u filter) for the 32 arcseconds search radius were applied at the same time. From which, we find that an interloping galaxy remains within the 32 arcseconds search radius, such that the tuned model returns photometric redshift estimates of  $z_{ph}: 0.5121$  with  $CI_{95\%}=[0.4954, 0.5281]$  for the 10 arcseconds search radius,  $z_{ph}: 0.4191$  with  $CI_{95\%}=[0.2343, 0.4699]$  for the 21 arcseconds search radius and  $z_{ph}: 0.1415$  with  $CI_{95\%}=[0.1259, 0.2168]$  for the 32 arcseconds search radius. This example shows that an interloping galaxy, presumably at lower redshift than the cluster itself, can contaminate model predictions when the search radius increases.



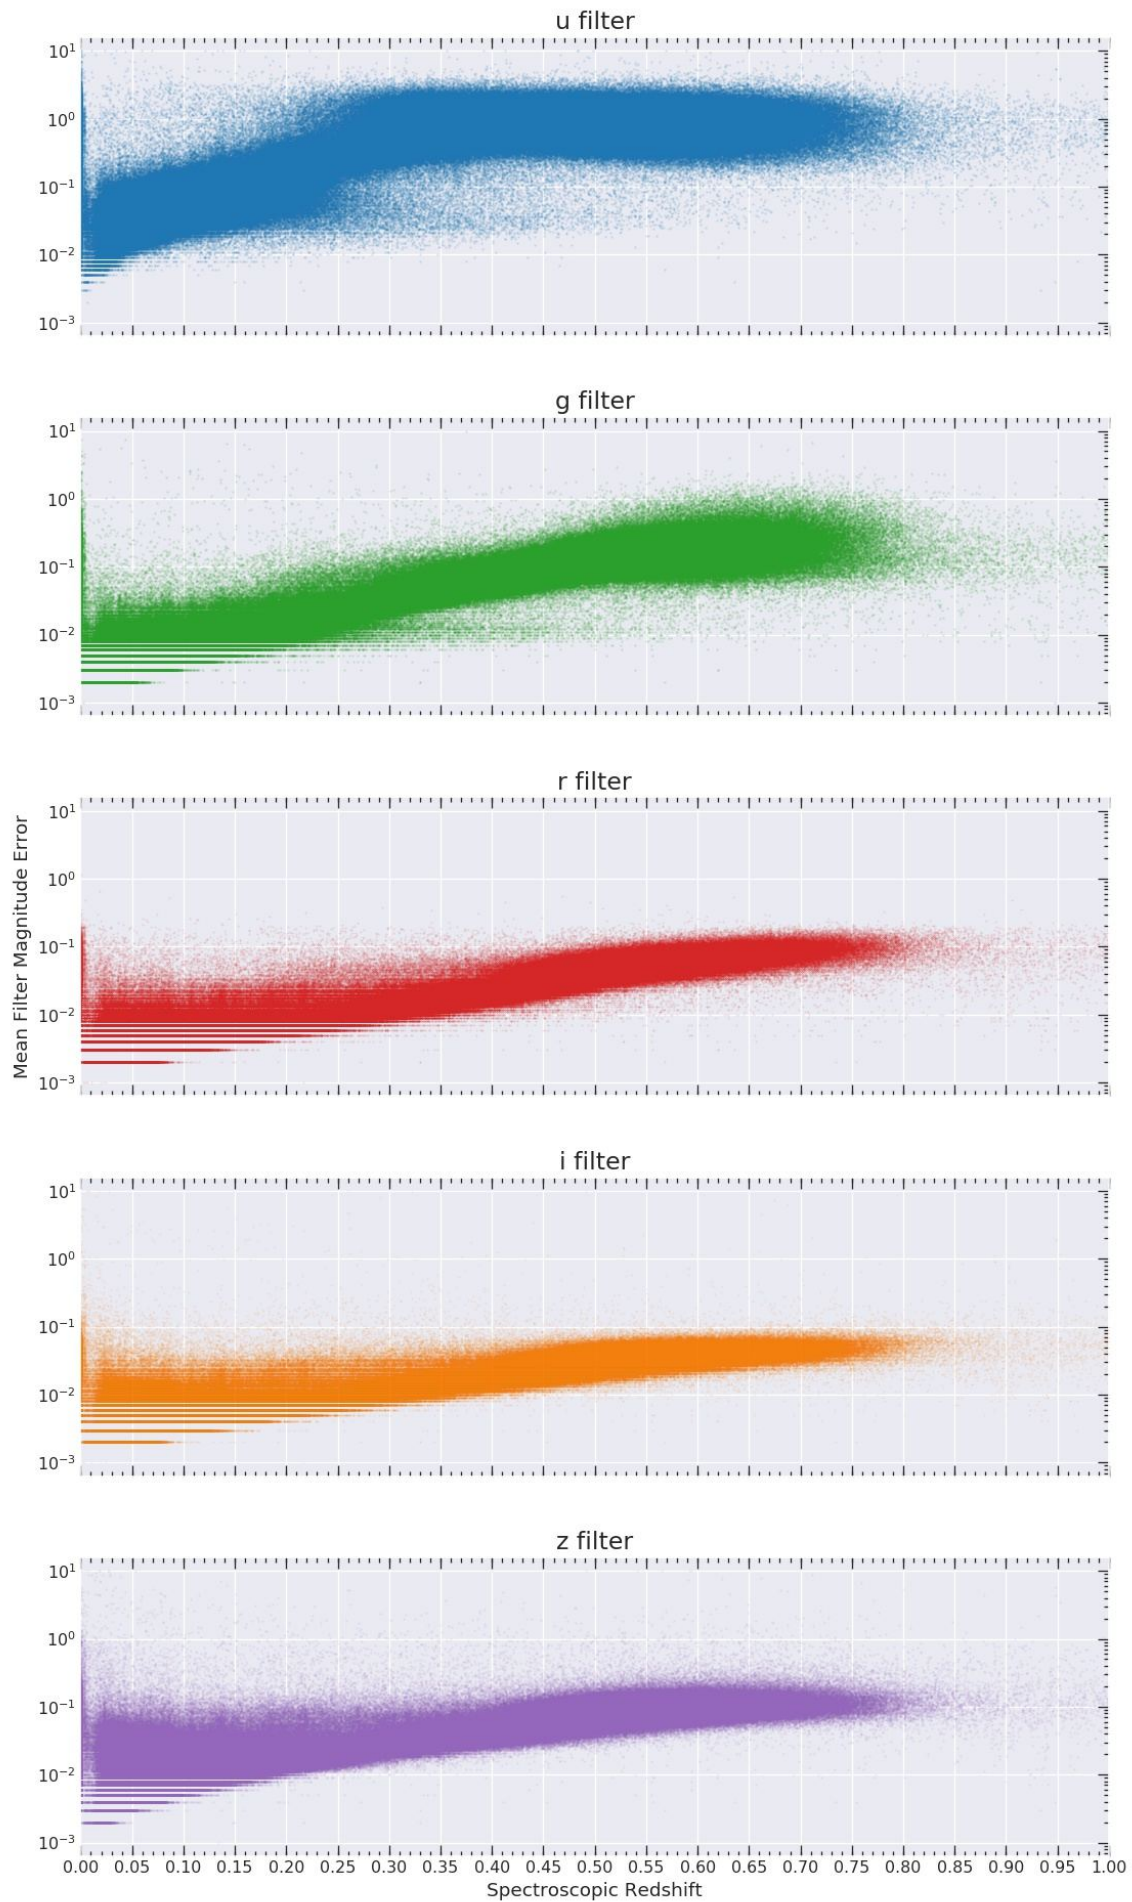

**Figure SA10.** Plots displaying the mean filter magnitude errors versus spectroscopic redshift of observed galaxies in SDSS for the u (top row), g (second from top row), r (middle row), i (second from bottom row) and z (bottom row) filters.

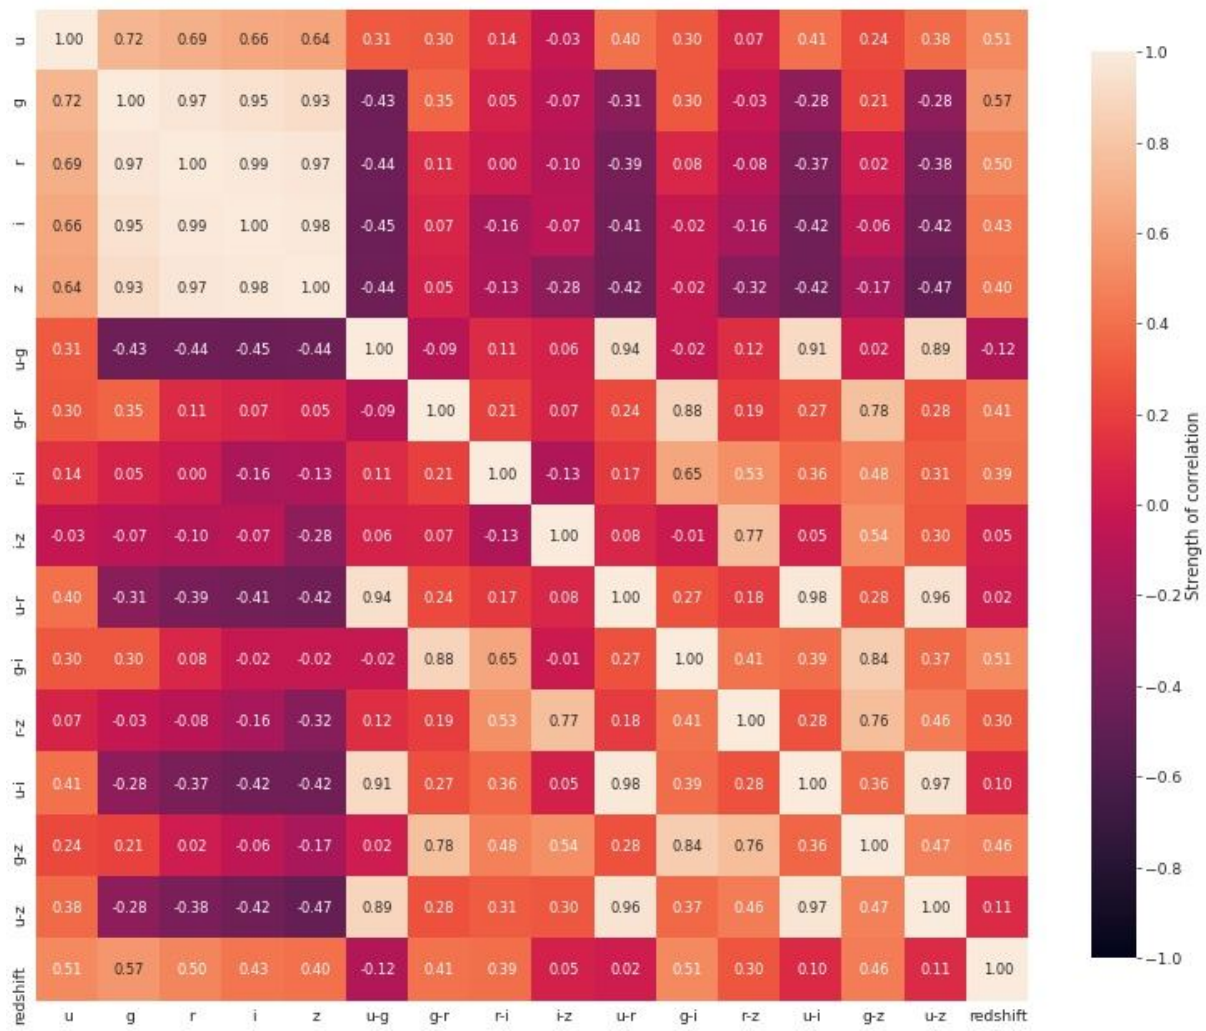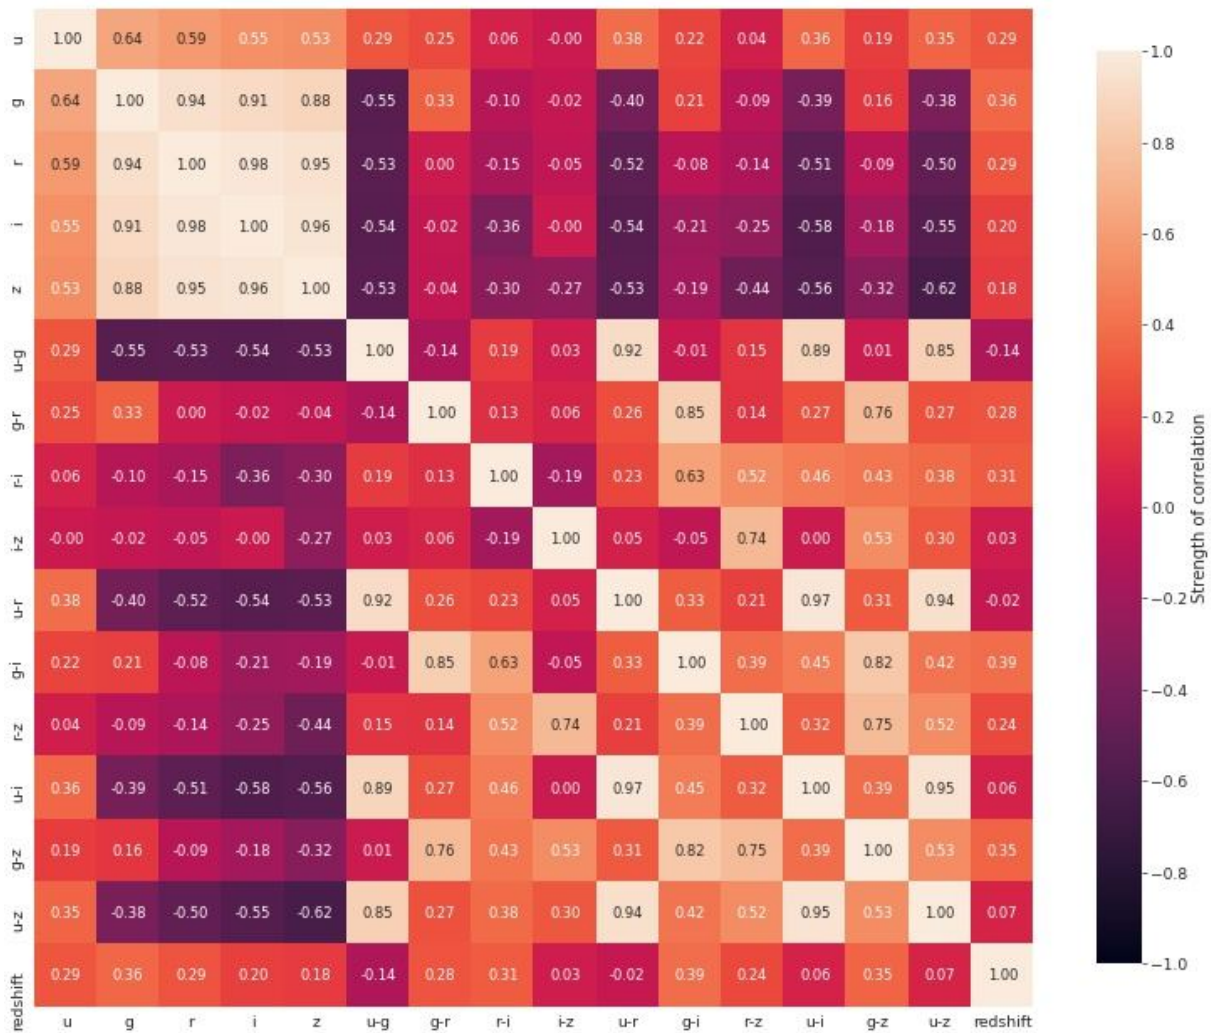



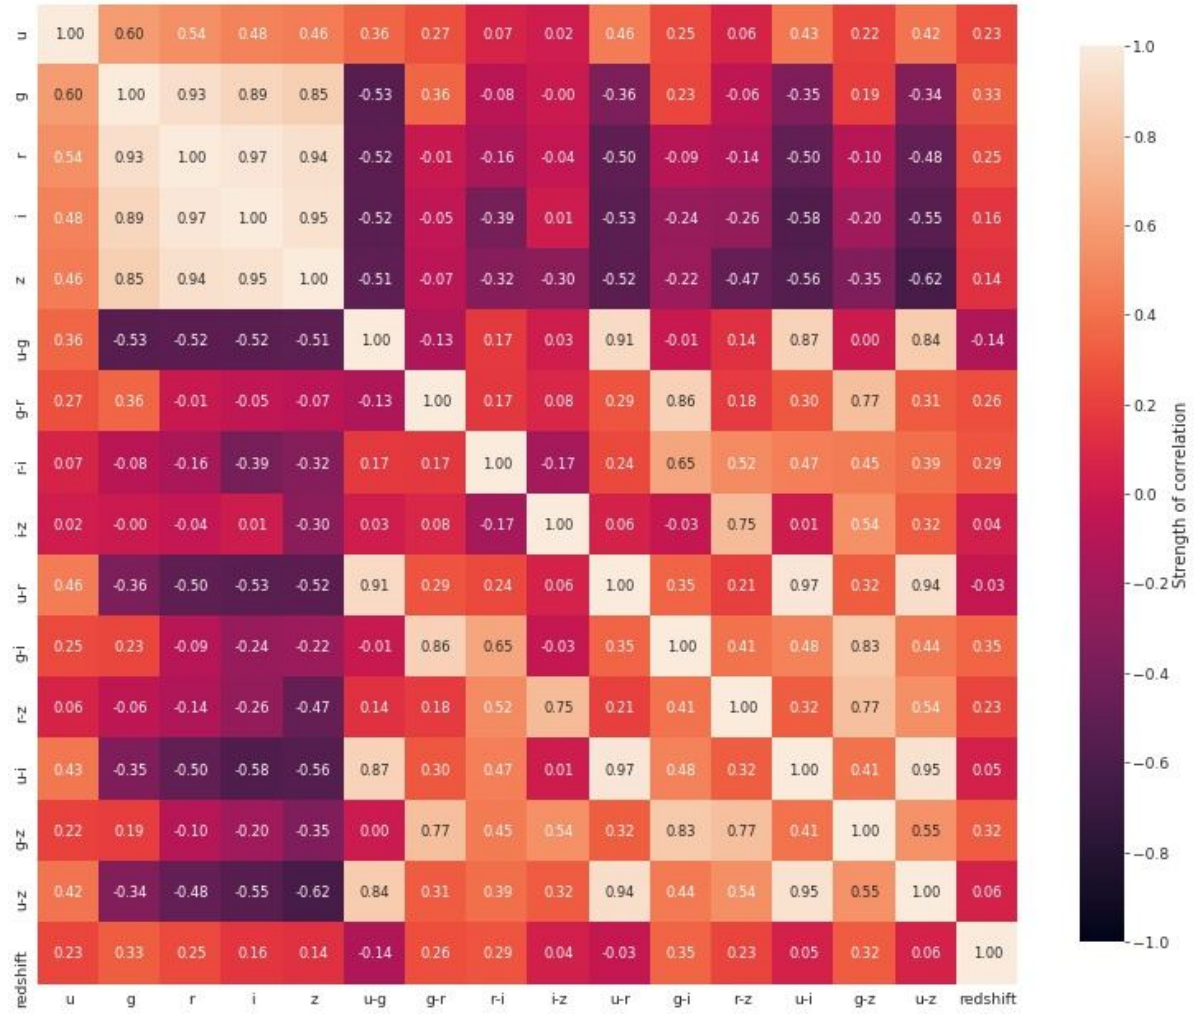

**Figure SA11.** Correlation matrix heatmaps of all features with raw photometry data from the MWAR training set for the 10 (top row), 21 (middle row) and 32 (bottom row) arcseconds search radius. The colourbar represents the strength of correlation between the features.

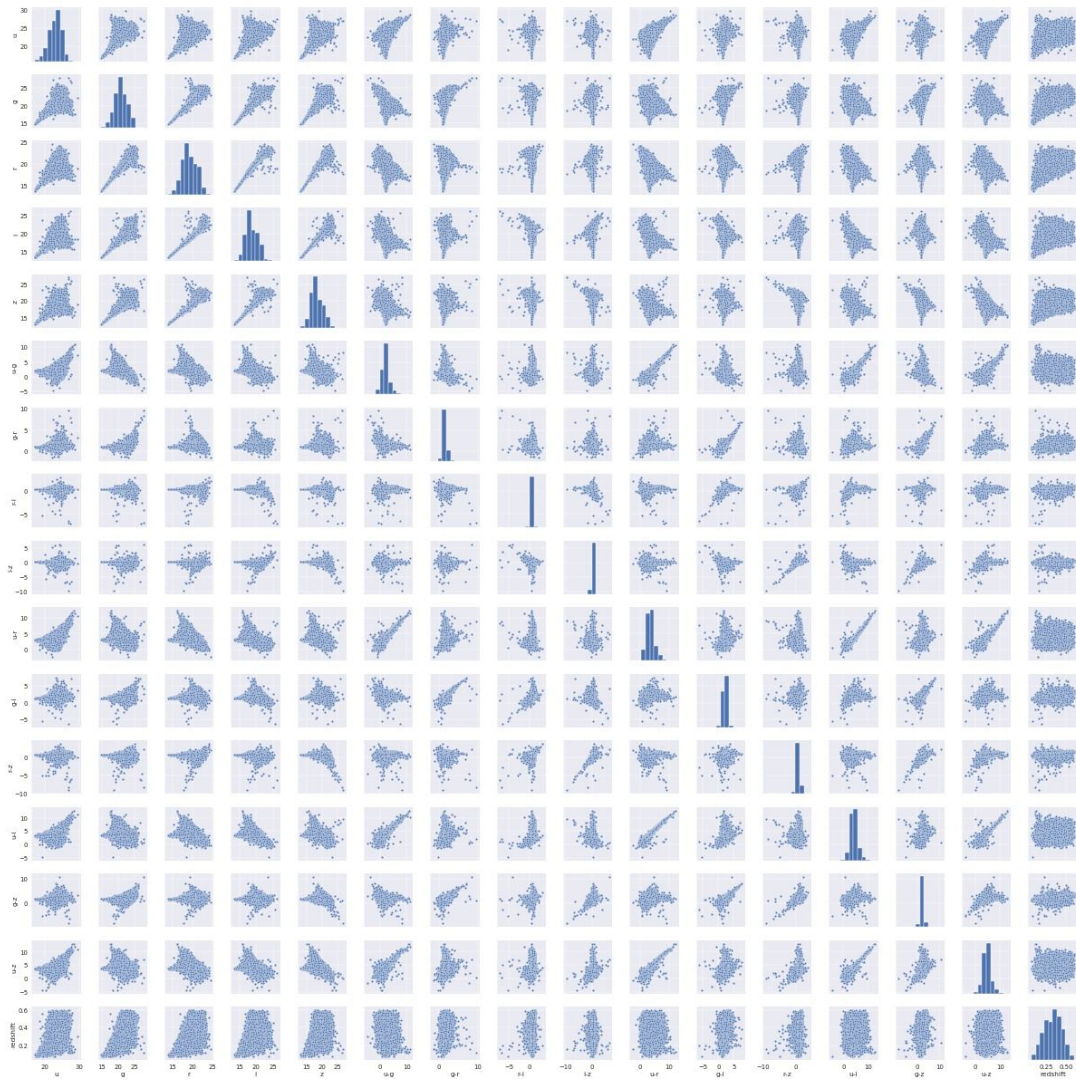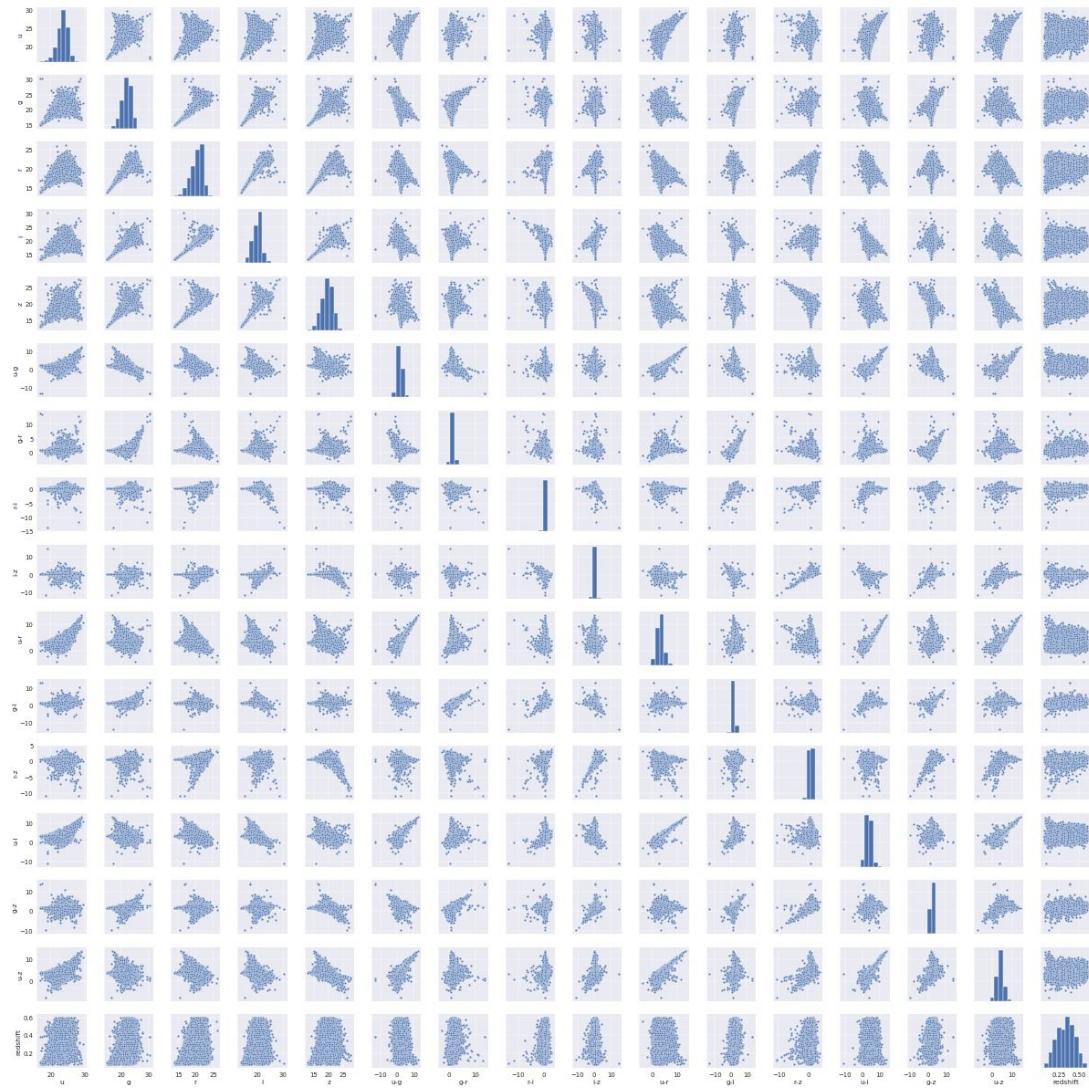



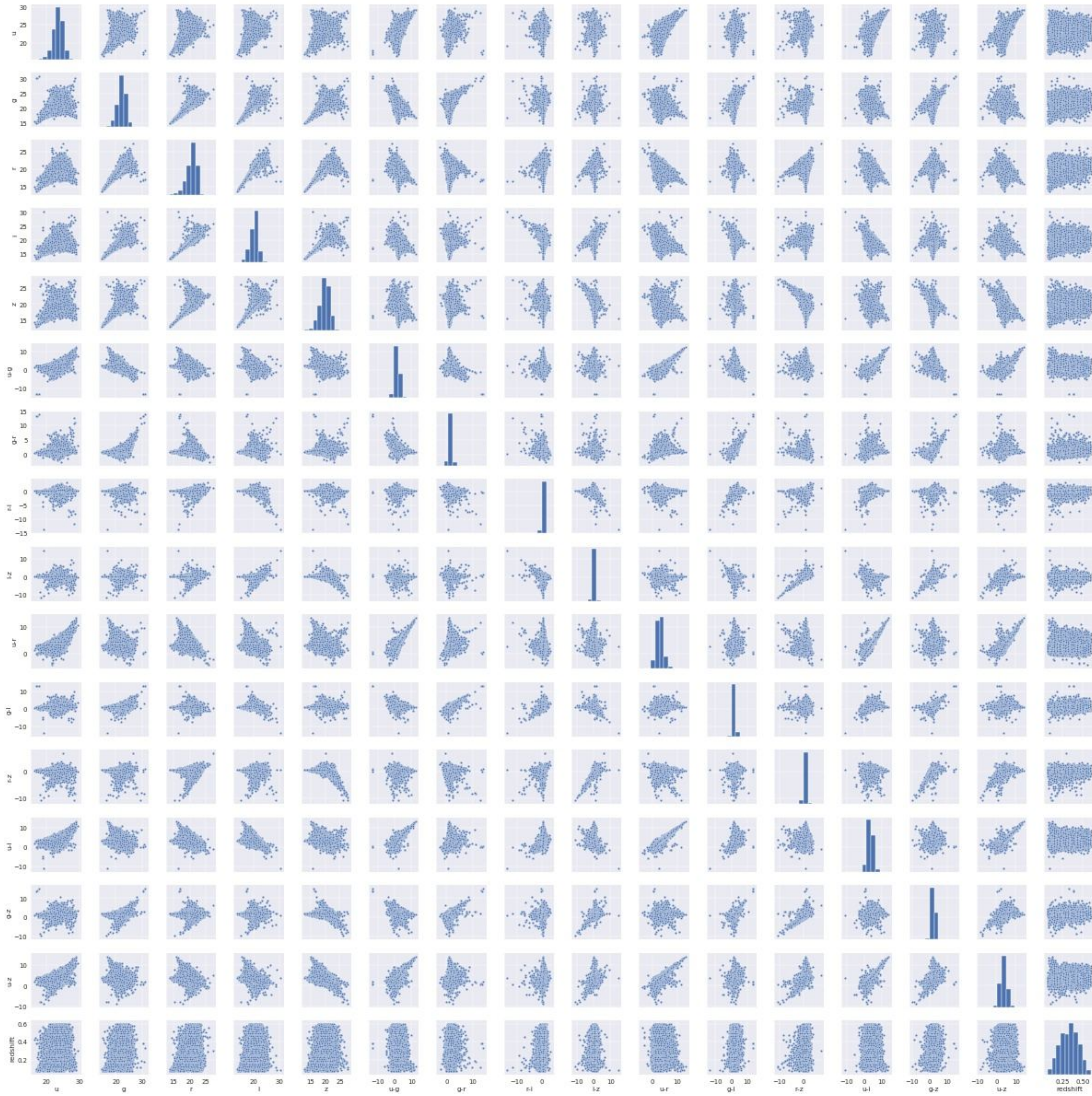

**Figure SA12.** Correlation matrix scatterplots of all features with raw photometry data from the MWAR training set for the 10 (top row), 21 (middle row) and 32 (bottom row) arcseconds search radius.

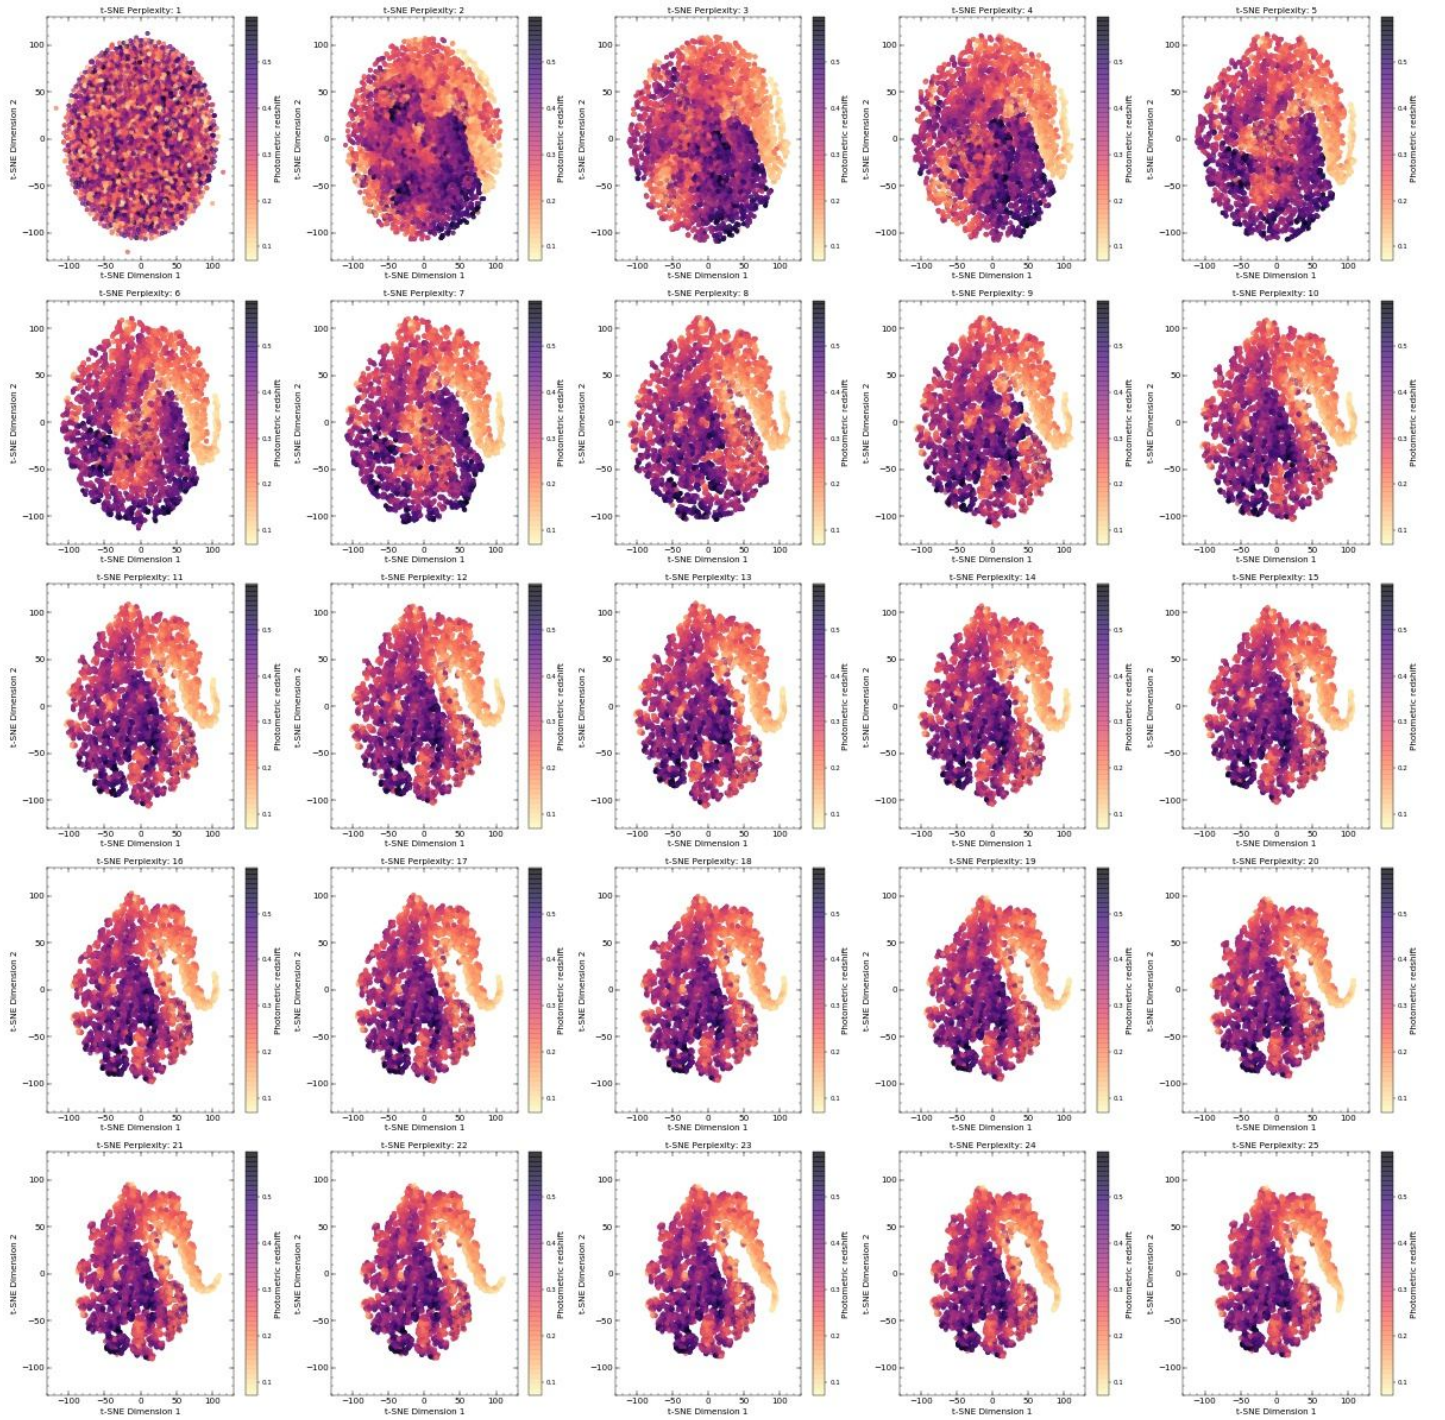

**Figure SA13.** Two dimensional representation of the feature space in the MWAR training set with no feature scaling applied for a 10 arcseconds search radius with LM filter magnitude-cuts applied using the t-SNE algorithm. The colourbar represents the photometric redshift of galaxies found within the search radius of clusters originally estimated by WHL12. The t-SNE perplexity value relates to the number of nearest neighbours used to compress the dimensionality of the dataset.



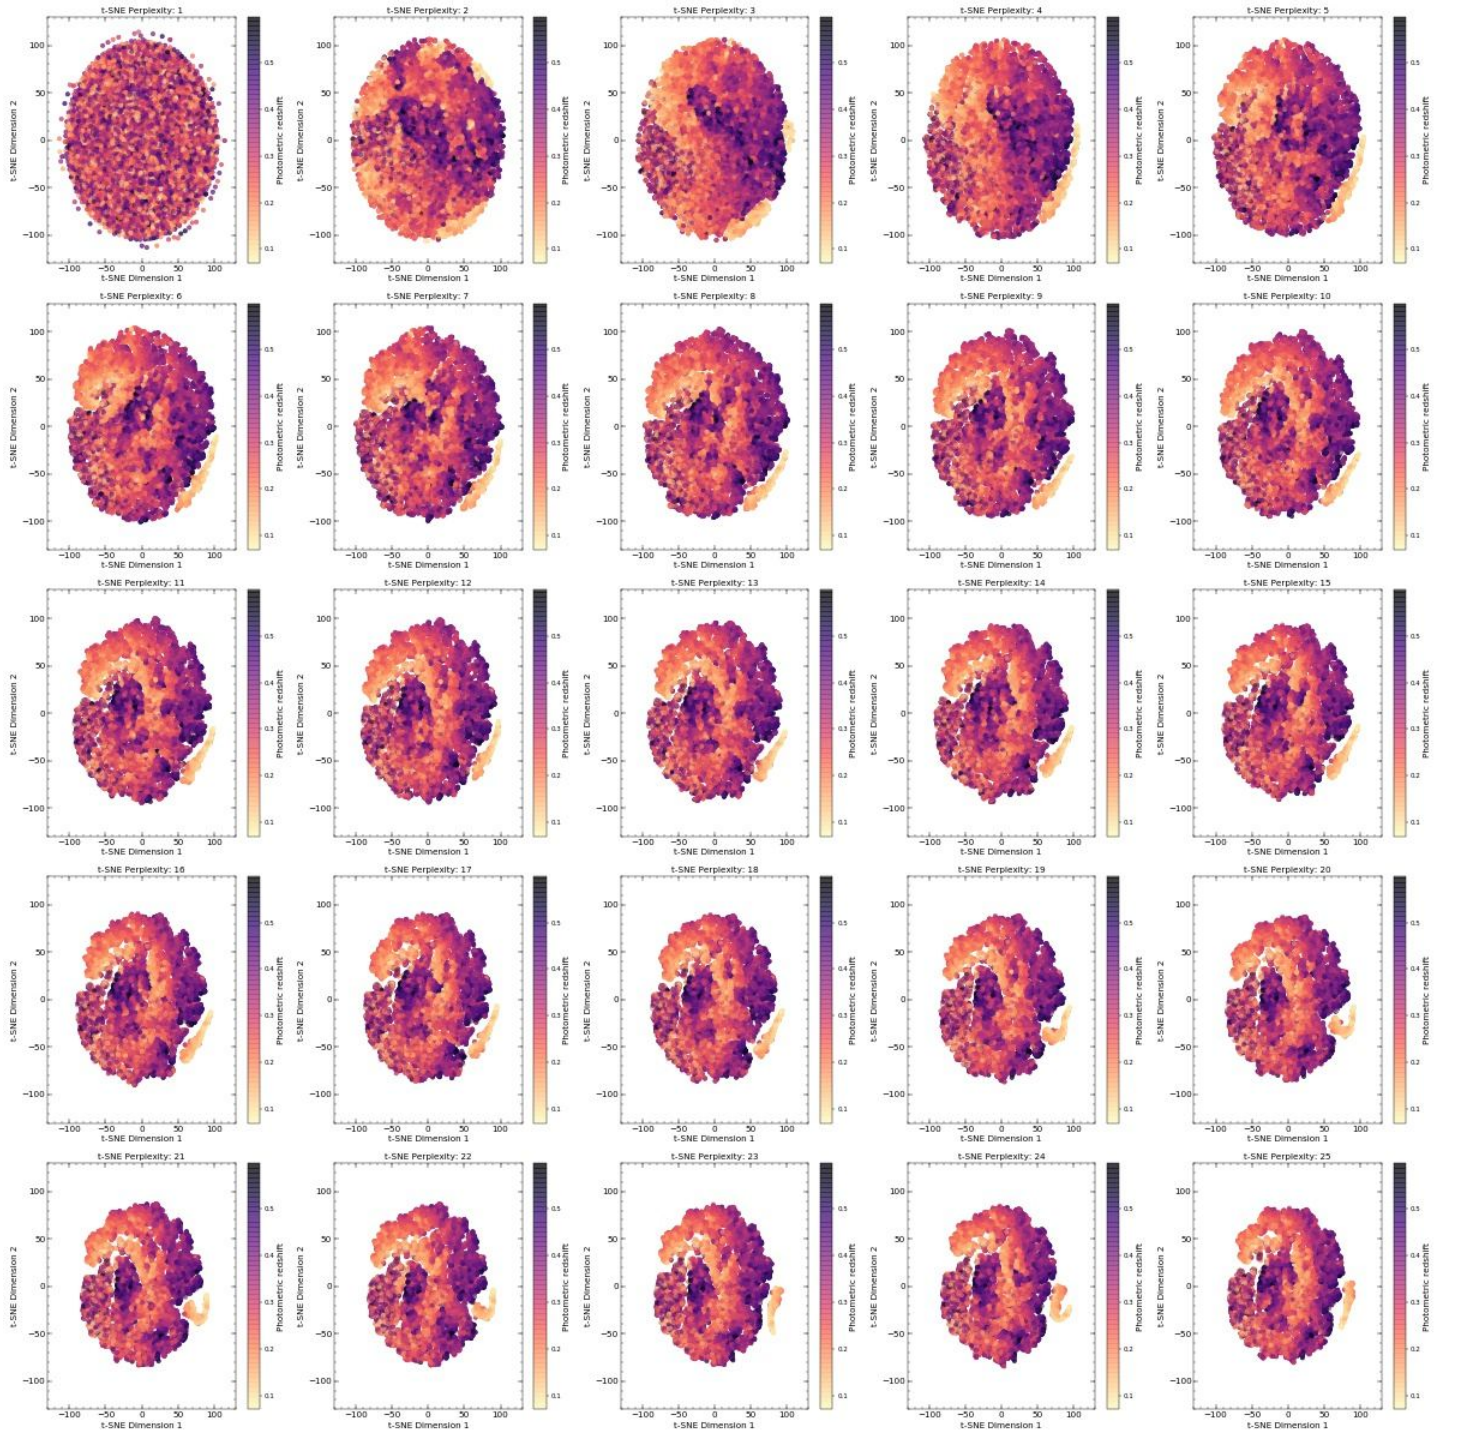

**Figure SA14.** Two dimensional representation of the feature space in the MWAR training set with no feature scaling applied for a 21 arcseconds search radius with LM filter magnitude-cuts applied using the t-SNE algorithm. The colourbar represents the photometric redshift of galaxies found within the search radius of clusters originally estimated by WHL12. The t-SNE perplexity value relates to the number of nearest neighbours used to compress the dimensionality of the dataset.



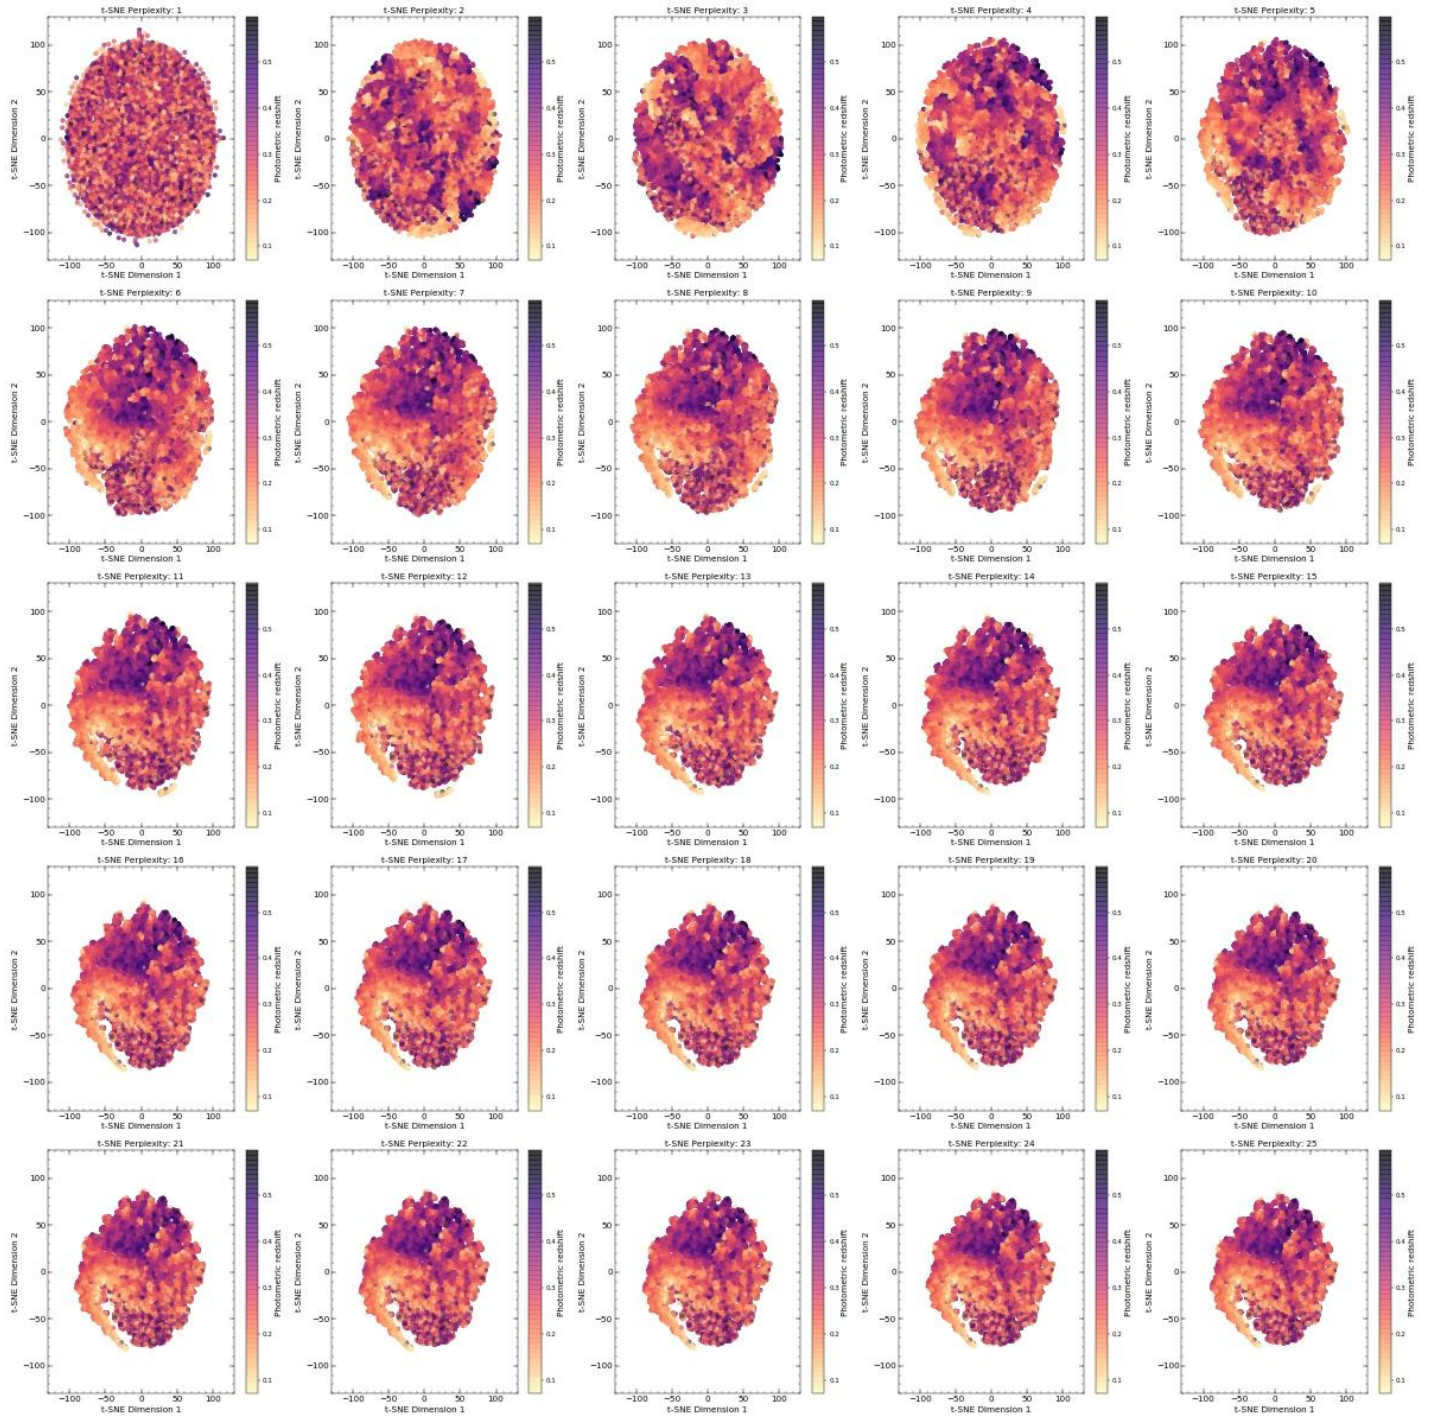

**Figure SA15.** Two dimensional representation of the feature space in the MWAR training set with no feature scaling applied for a 32 arcseconds search radius with LM-0.5 filter magnitude-cuts applied using the t-SNE algorithm. The colourbar represents the photometric redshift of galaxies found within the search radius of clusters originally estimated by WHL12. The t-SNE perplexity value relates to the number of nearest neighbours used to compress the dimensionality of the dataset.



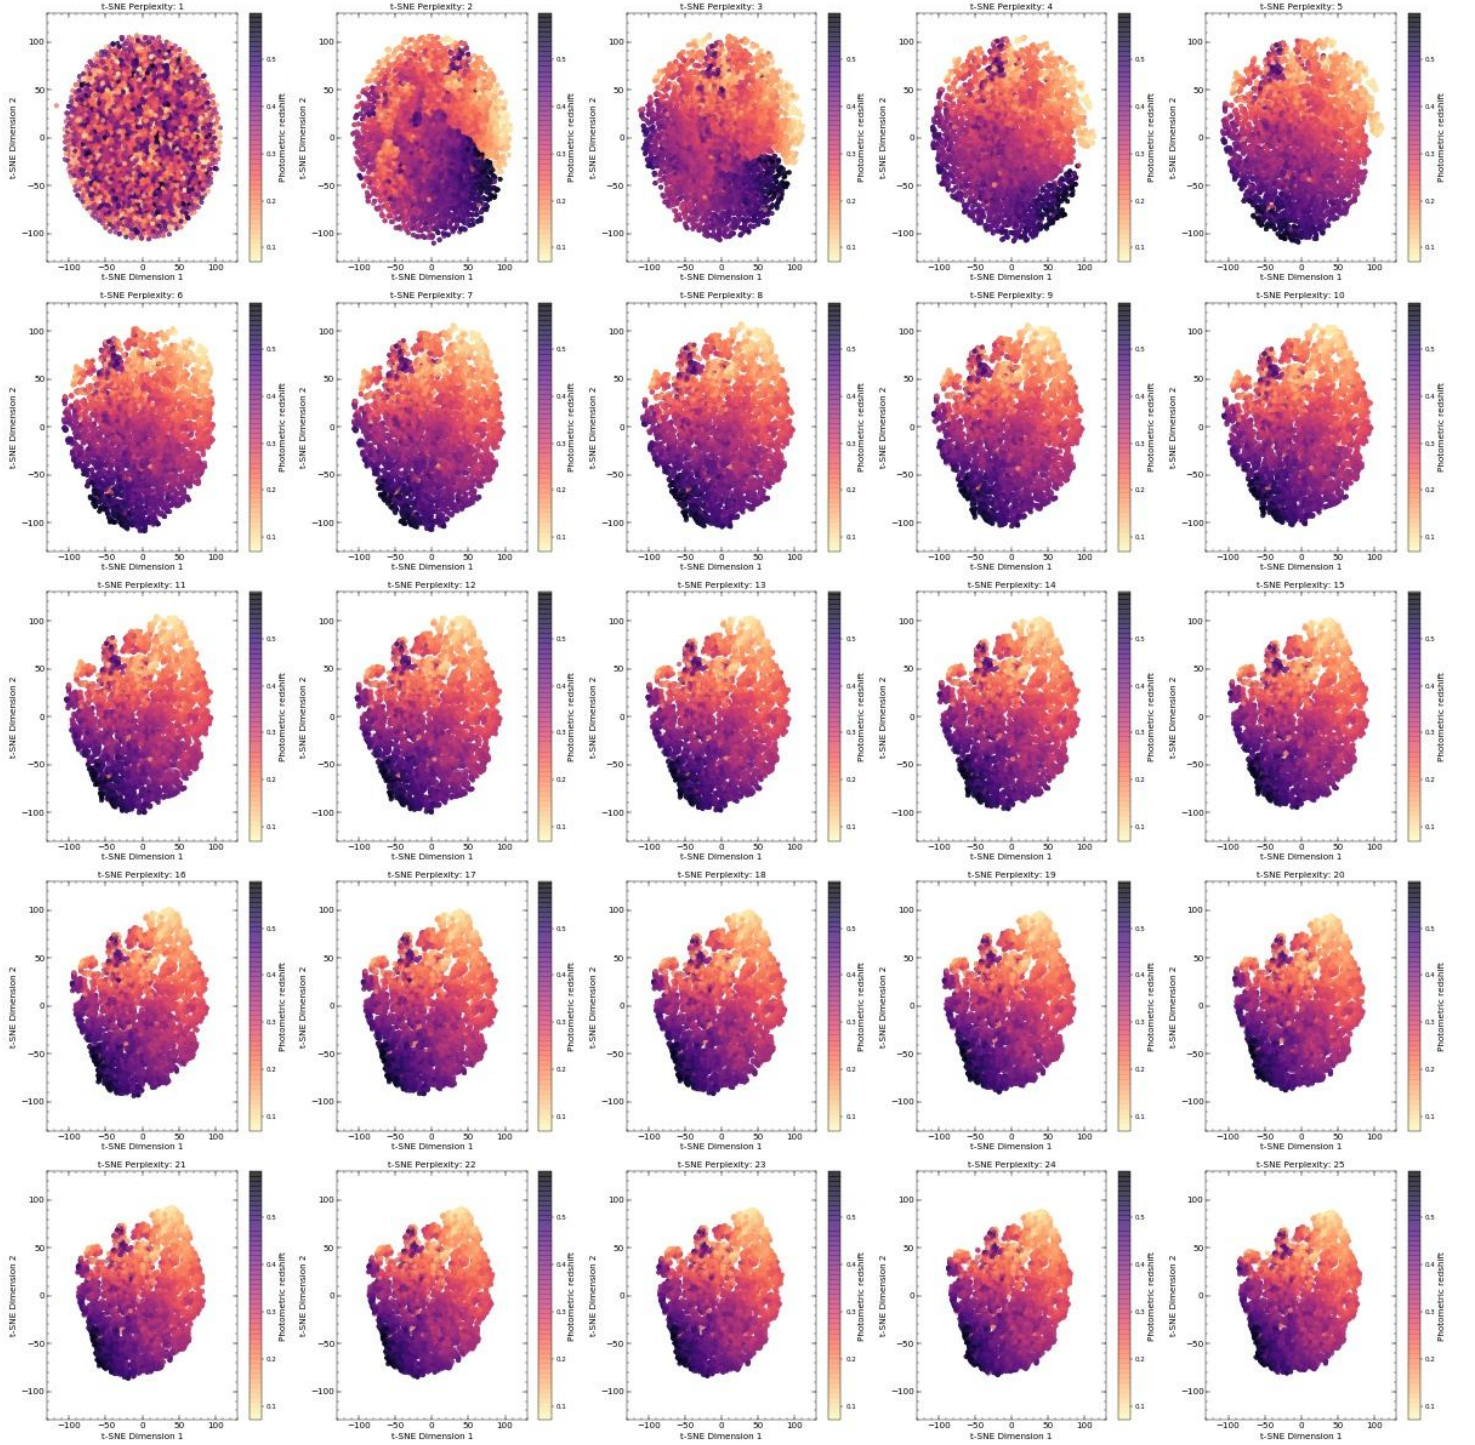

**Figure SA16.** Two dimensional representation of the feature space in the MWAR training set with feature scaling applied for a 10 arcseconds search radius with LM filter magnitude-cuts applied using the t-SNE algorithm. The colourbar represents the photometric redshift of galaxies found within the search radius of clusters originally estimated by WHL12. The t-SNE perplexity value relates to the number of nearest neighbours used to compress the dimensionality of the dataset.



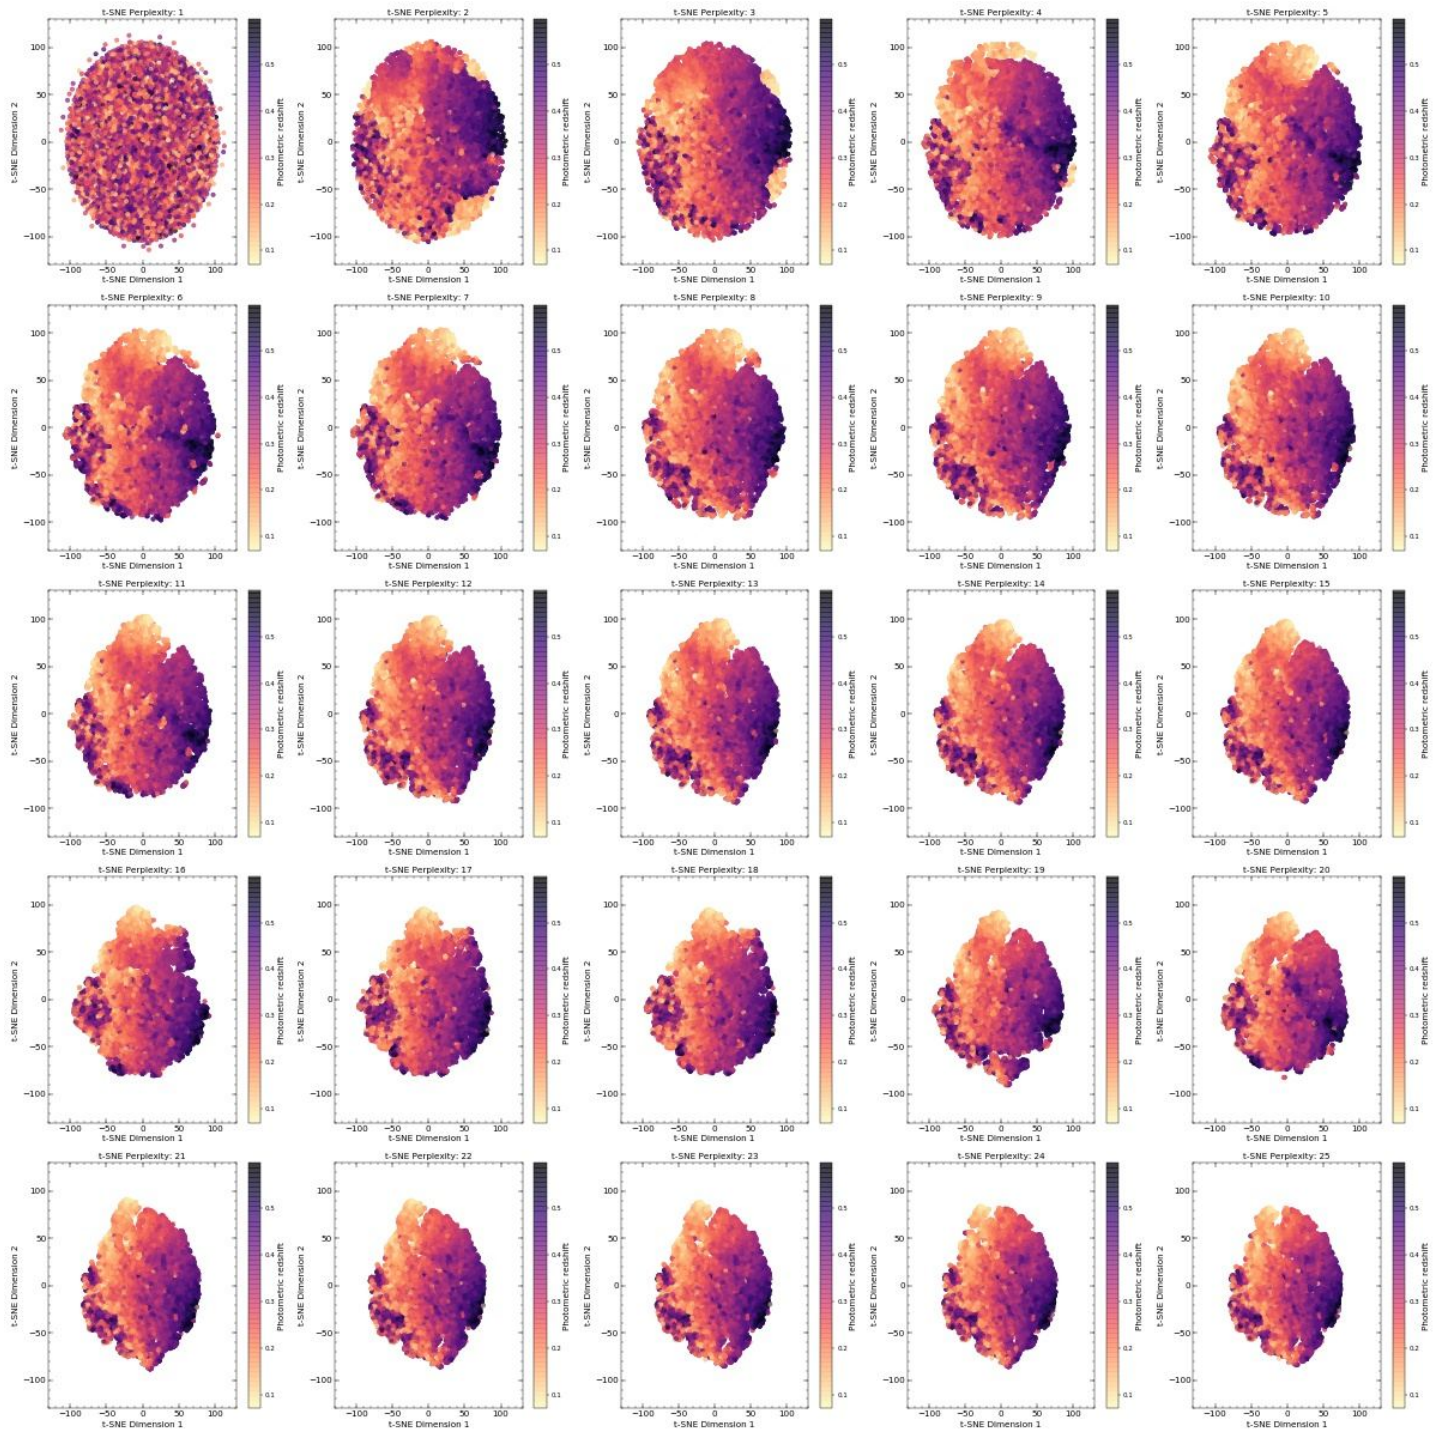

**Figure SA17.** Two dimensional representation of the feature space in the MWAR training set with feature scaling applied for a 21 arcseconds search radius with LM filter magnitude-cuts applied using the t-SNE algorithm. The colourbar represents the photometric redshift of galaxies found within the search radius of clusters originally estimated by WHL12. The t-SNE perplexity value relates to the number of nearest neighbours used to compress the dimensionality of the dataset.

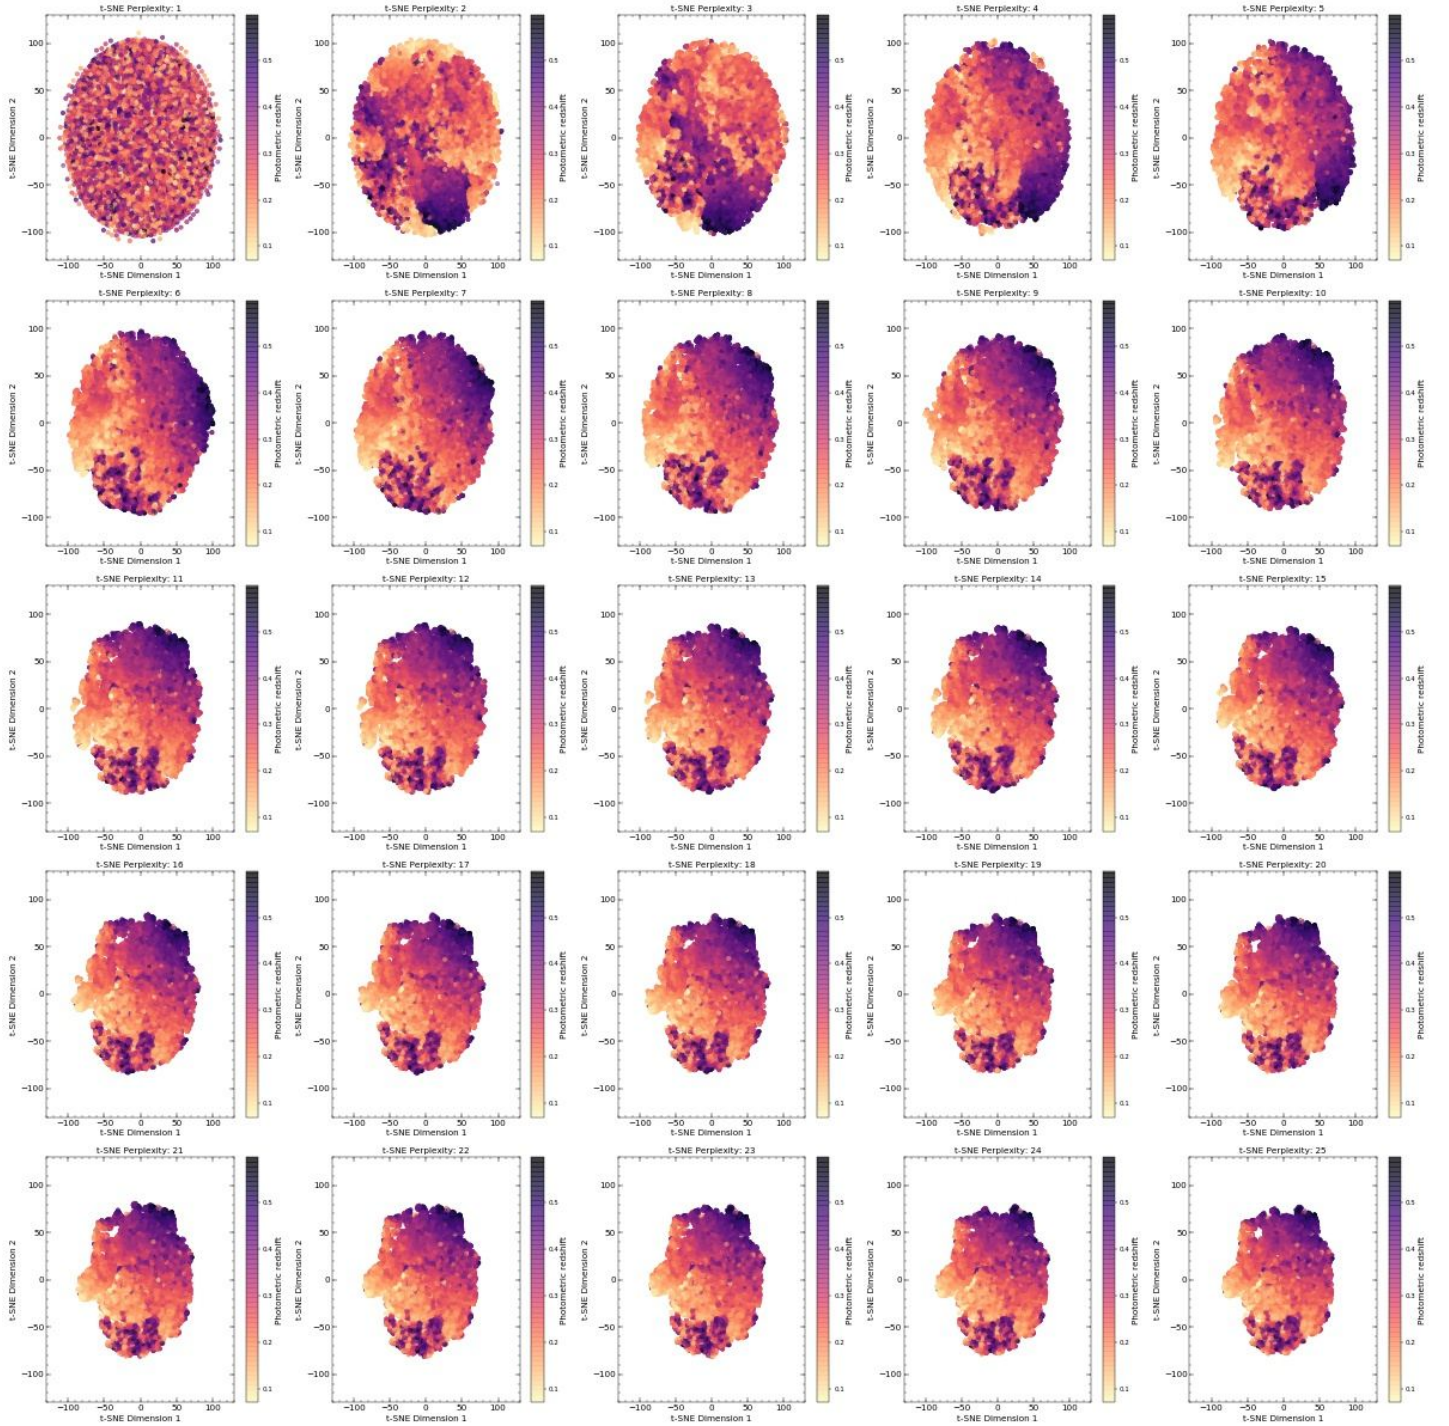

**Figure SA18.** Two dimensional representation of the feature space in the MWAR training set with feature scaling applied for a 32 arcseconds search radius with LM-0.5 filter magnitude-cuts applied using the t-SNE algorithm. The colourbar represents the photometric redshift of galaxies found within the search radius of clusters originally estimated by WHL12. The t-SNE perplexity value relates to the number of nearest neighbours used to compress the dimensionality of the dataset.
